# Supplementary material for: Variations of absolute source positions determined from quad-band VLBI observations
Source: arXiv:2501.18276 source file (2025-01-30)
Supplement: Supplementary file 1 [file supplementary_position_time_series.pdf]

**supplementary for manuscript entitled “Variations of absolute source positions determined from quad-band VLBI observations”**

MING HUI XU<sup>1</sup> AND PATRICK CHARLOT<sup>2</sup>

<sup>1</sup>*Deutsches GeoForschungsZentrum (GFZ), Telegrafenberg, 14476 Potsdam, Germany*

<sup>2</sup>*Laboratoire d’astrophysique de Bordeaux, Univ. de Bordeaux, CNRS, B18N, Allée Geoffroy Saint-Hilaire, 33615 Pessac, France*

**ABSTRACT**

Active Galactic Nuclei (AGNs) observed with the technique of very long baseline interferometry (VLBI) are used as fiducial references on the sky to precisely measure the shape and orientation of the Earth. Their positions form a celestial reference frame that plays an important role in both astronomy and geodesy. This study investigates the accuracy and stability of the positions of the AGNs that are measured by simultaneous VLBI observations at 3.3, 5.5, 6.6, and 10.5 GHz. Based on position time series from dedicated geodetic solutions, we characterize the observed source position variations and identify the possible factors causing such variations. We find that the primary contributor is source structure for sources above 20° declination while the sensitivity of the observations to the declination coordinate predominates for sources below 20° declination. The position time series are further explored to derive more realistic uncertainties for the quad-band positions. Significant position offsets with respect to the positions at 2.2/8.6 GHz are found for 15% of the sources. For 6% of the sources, the offsets are larger than 0.8 milli-arcseconds. Source structure may be divided into two parts: the invisible structure (within the beam size) and the visible structure (on larger scales). The latter causes closure delays enlarging post-fit delay residuals in geodetic solutions whereas the former causes source position changes. Such position changes will contribute significantly to the offsets between radio and optical positions. Overall, this work highlights the necessity to have a specific quad-band catalog for processing operational quad-band observations.

*Keywords:* celestial reference frame – AGNs – VLBI – VGOS – source structure

**1. PLOTS OF QUAD-BAND POSITION TIME SERIES**

In this supplementary document, we provide the quad-band position time series for 96 sources, with two of them per page. For each source, the position time series was obtained from a global solution where the position of the source was estimated session-wise. These daily position coordinates are relative to its S/X position in the ICRF3. Color coding depicts the epoch of each of the quad-band sessions where the source was observed. The standard deviation of the position estimates with respect to the weighted mean, for both RA and Dec coordinates, is reported in the upper-right corner. Position estimates with a strong correlation ( $> 0.7$ ) between right ascension and declination are not shown as they have very large uncertainties due to a few observations in those epochs. The source name and the number of sessions (i.e., the number of the daily estimates presented in the plot) are reported in the upper-left corner.

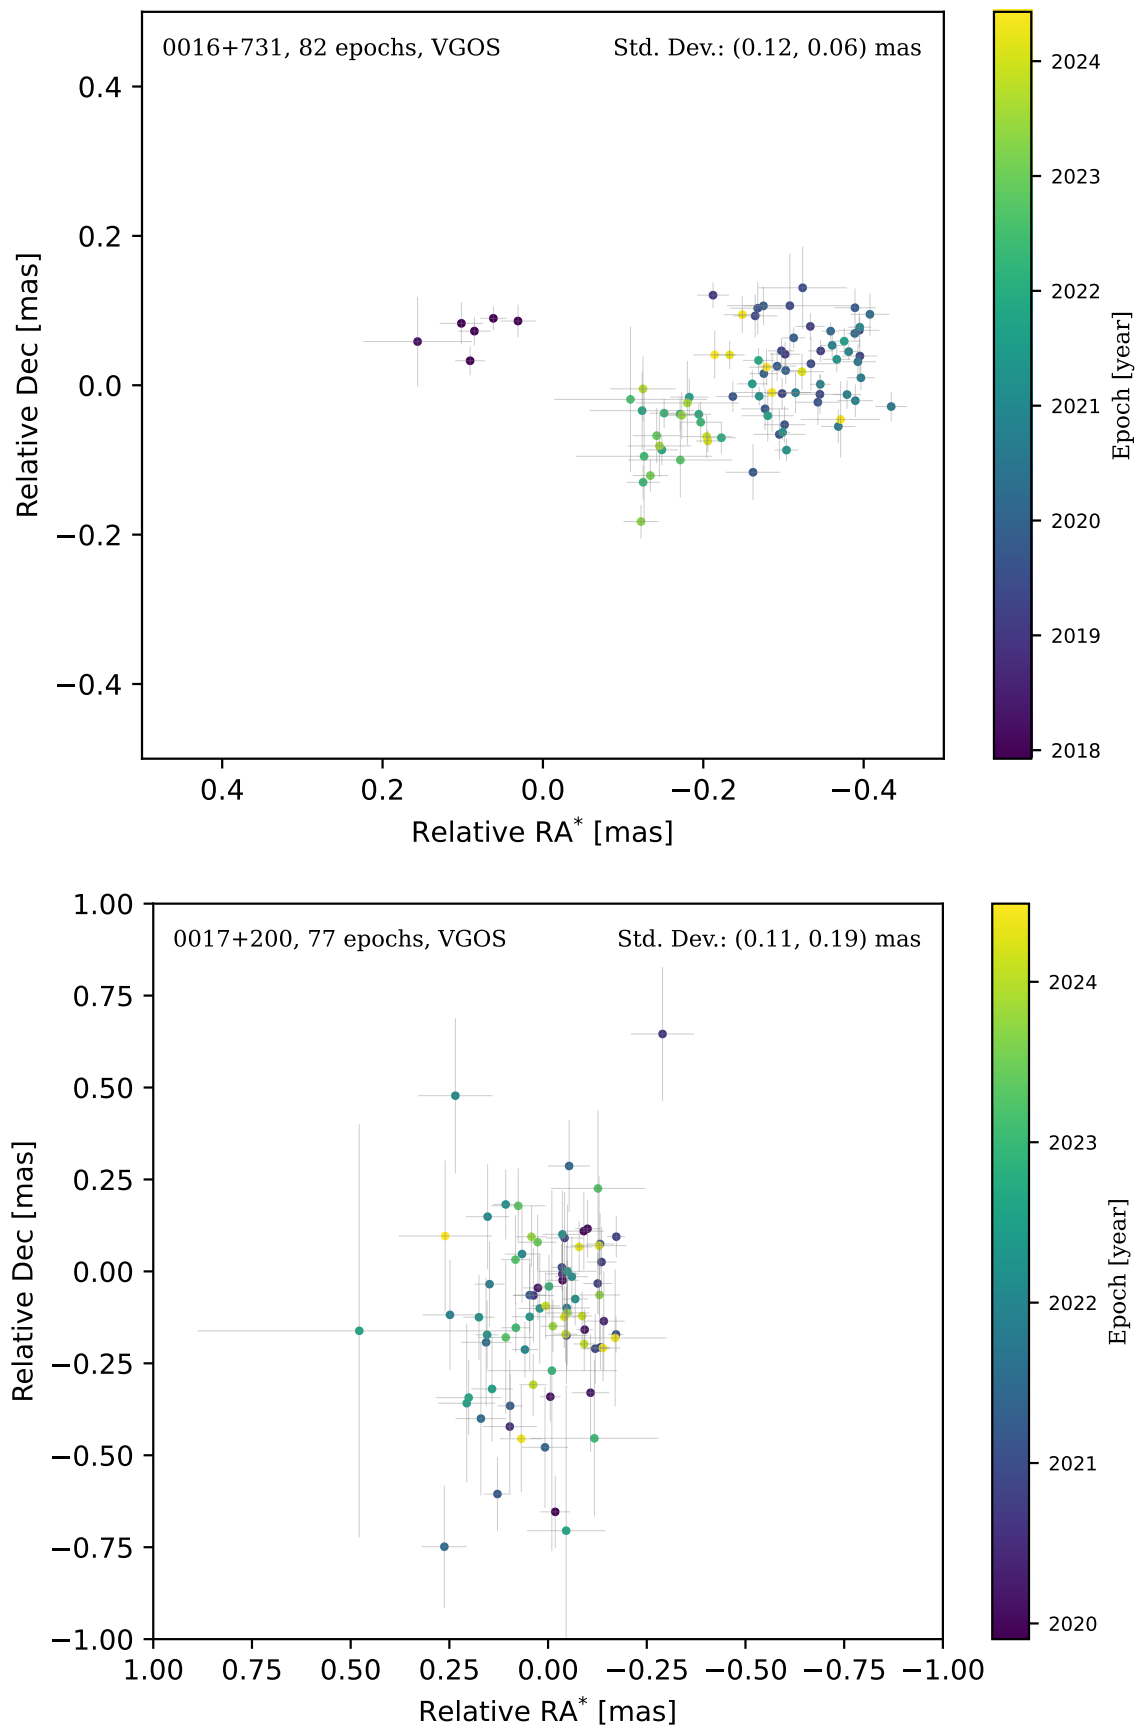

**Figure 1.** Position time series

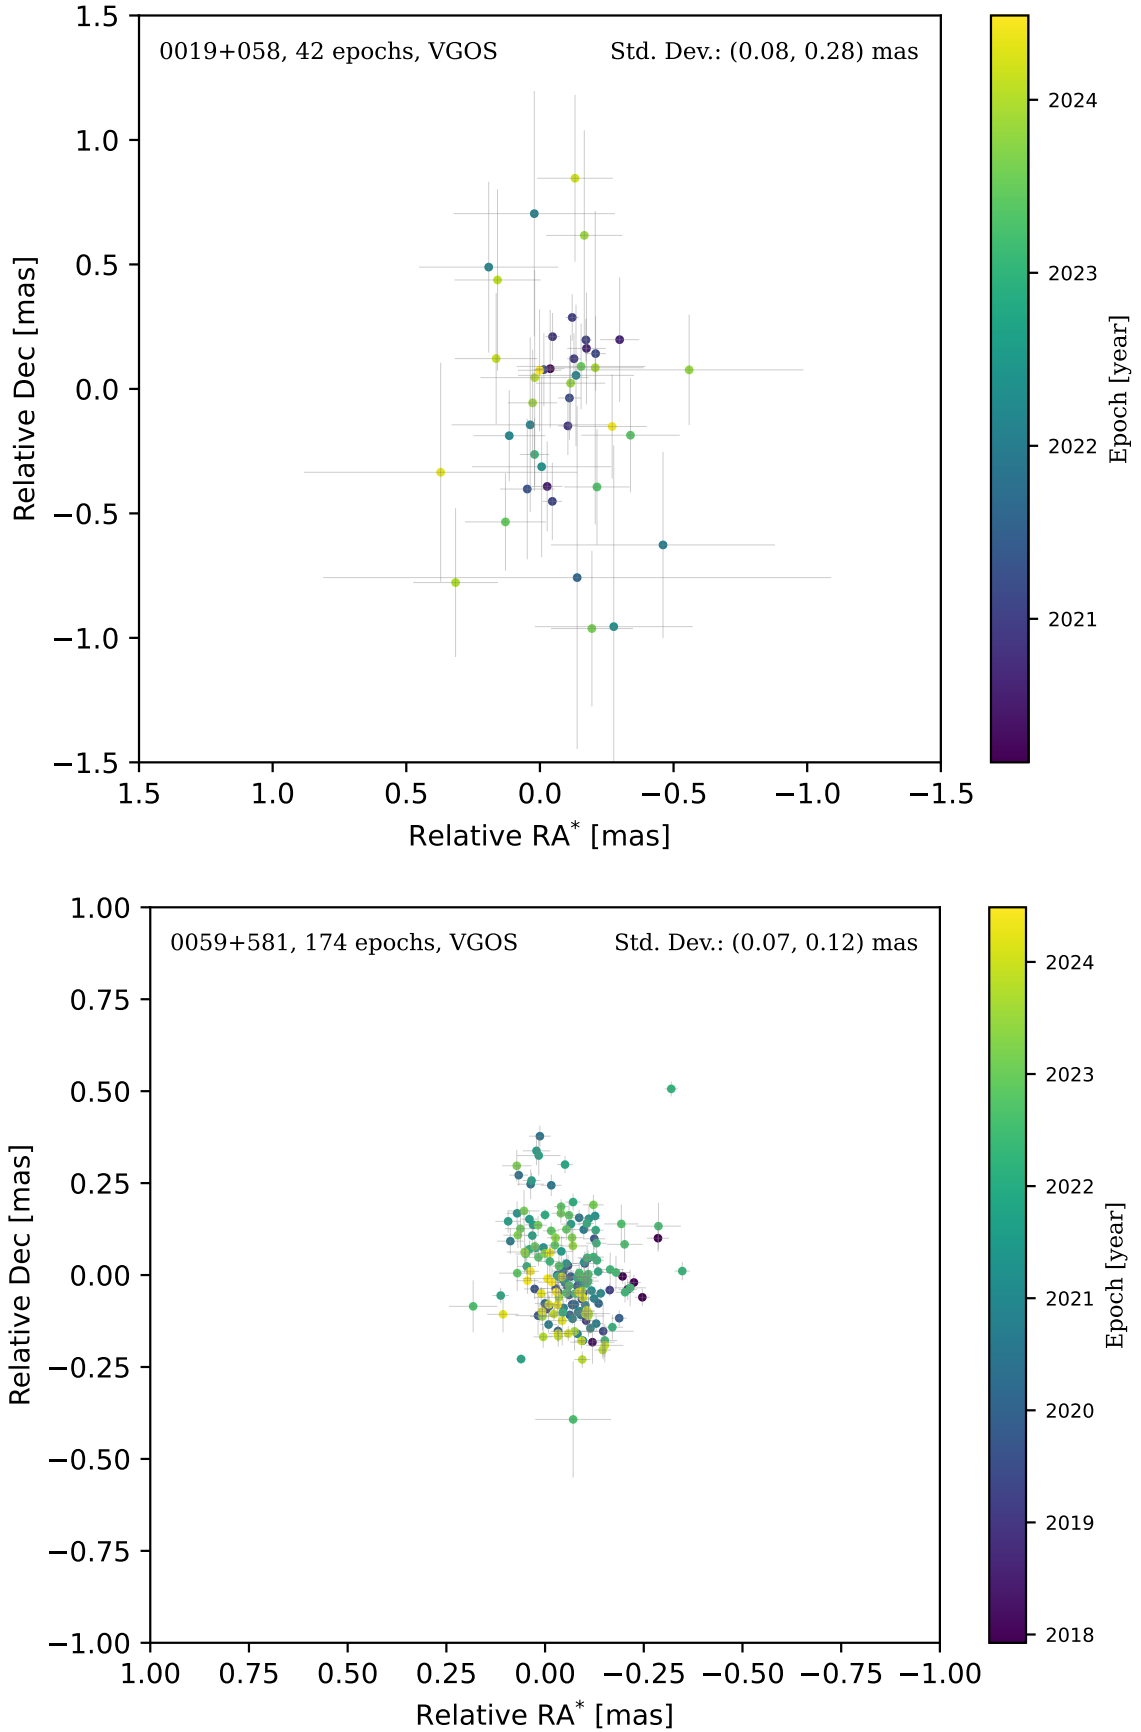**Figure 2.** Position time series

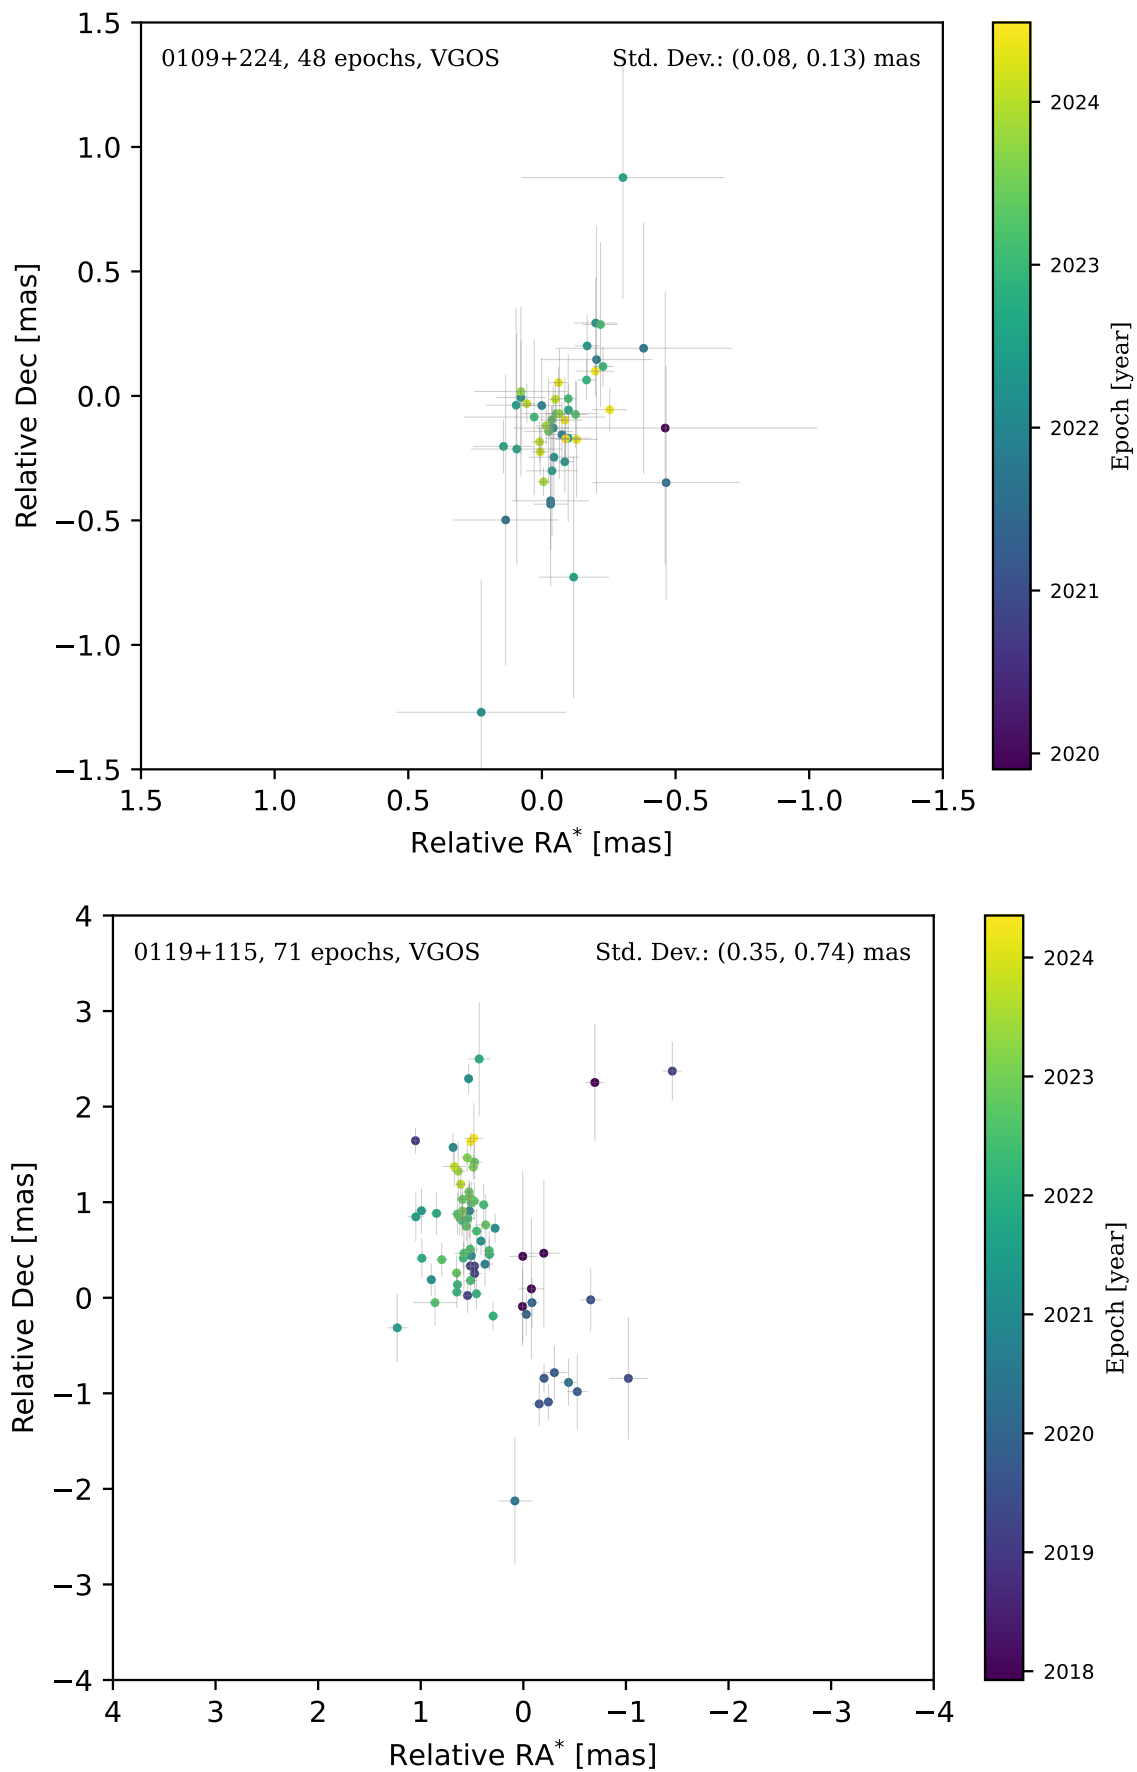

**Figure 3.** Position time series

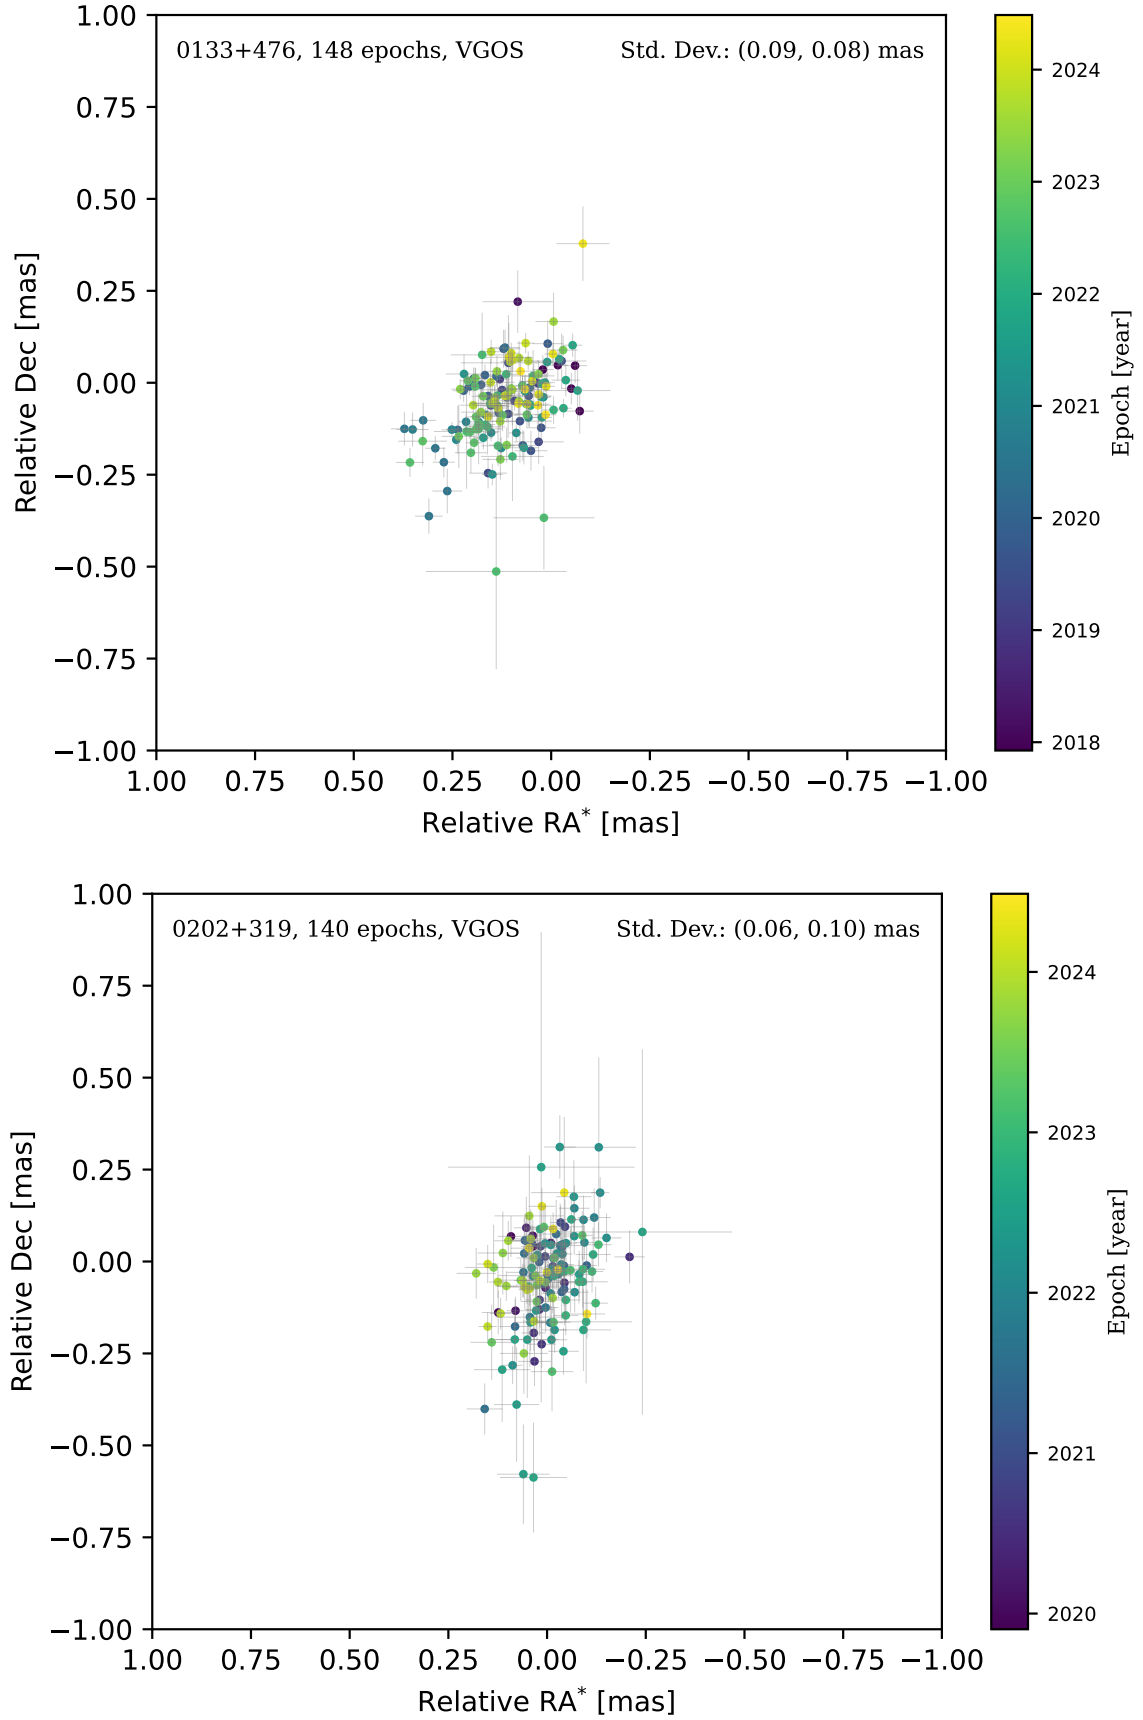

Figure 4. Position time series

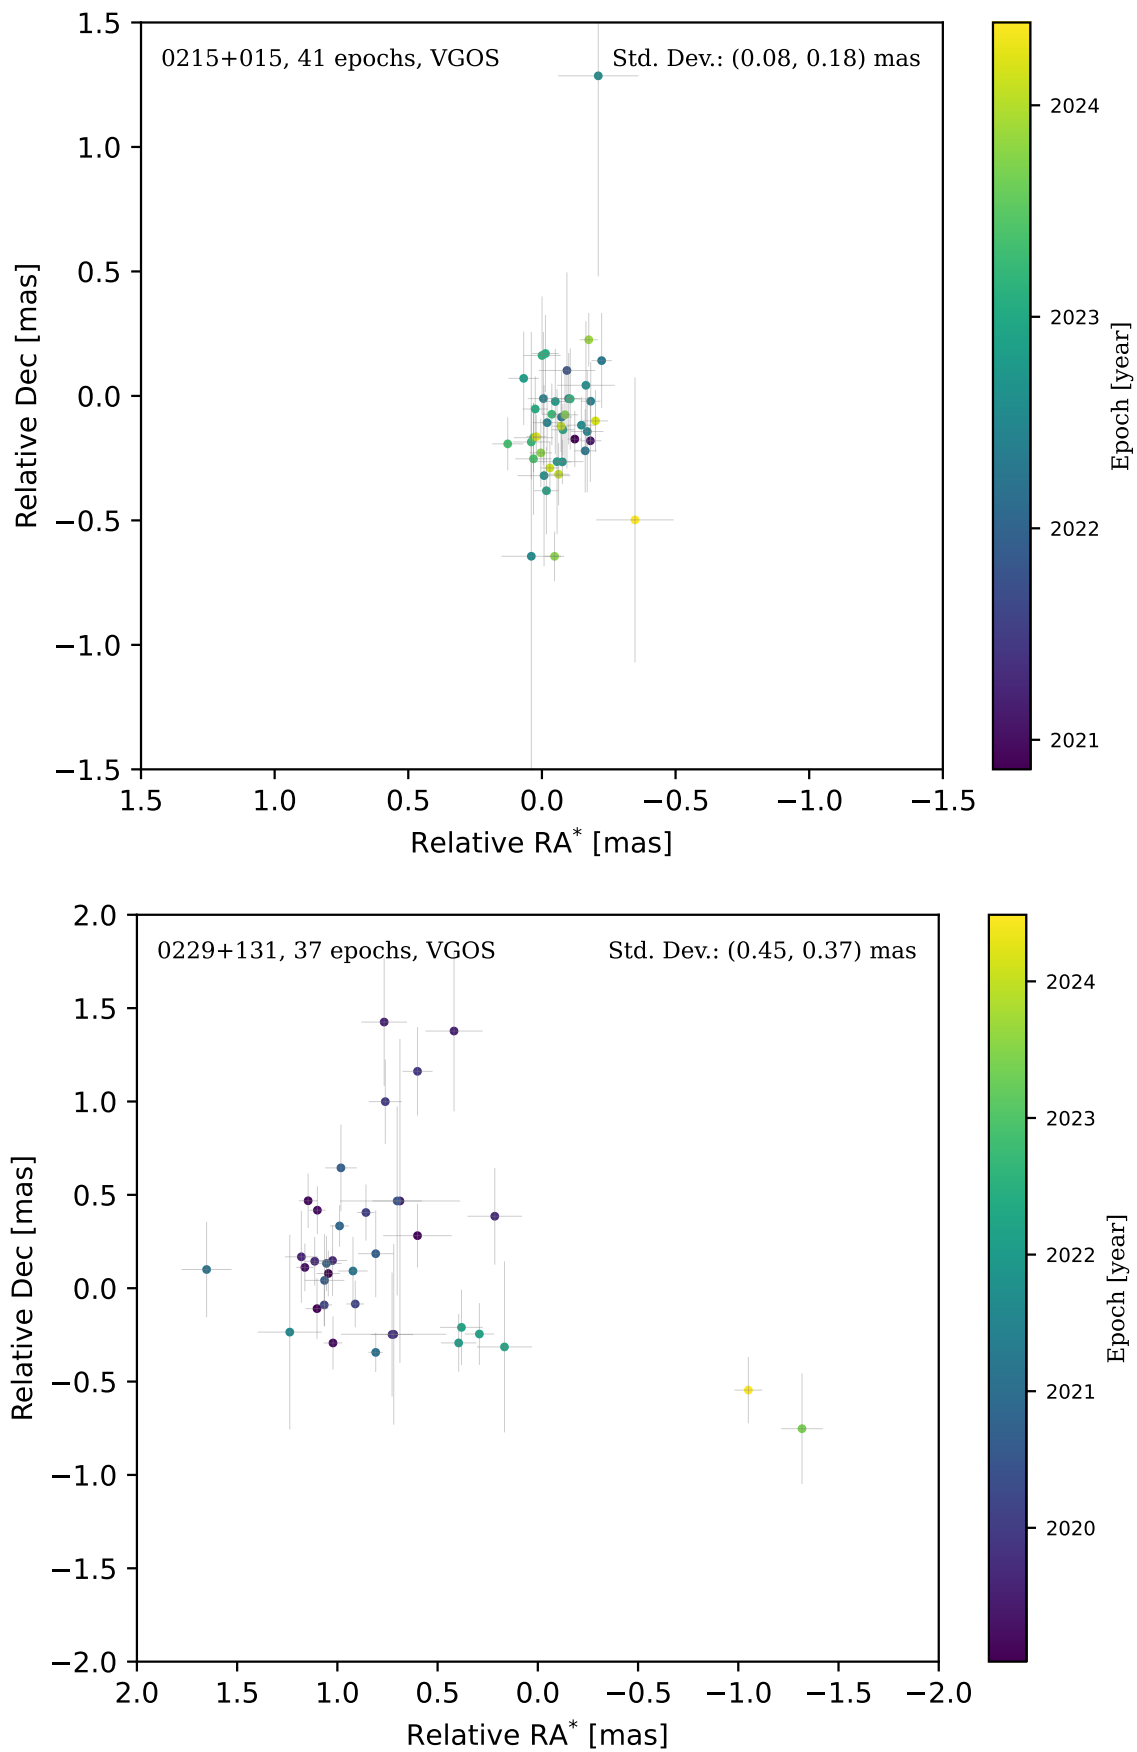

**Figure 5.** Position time series

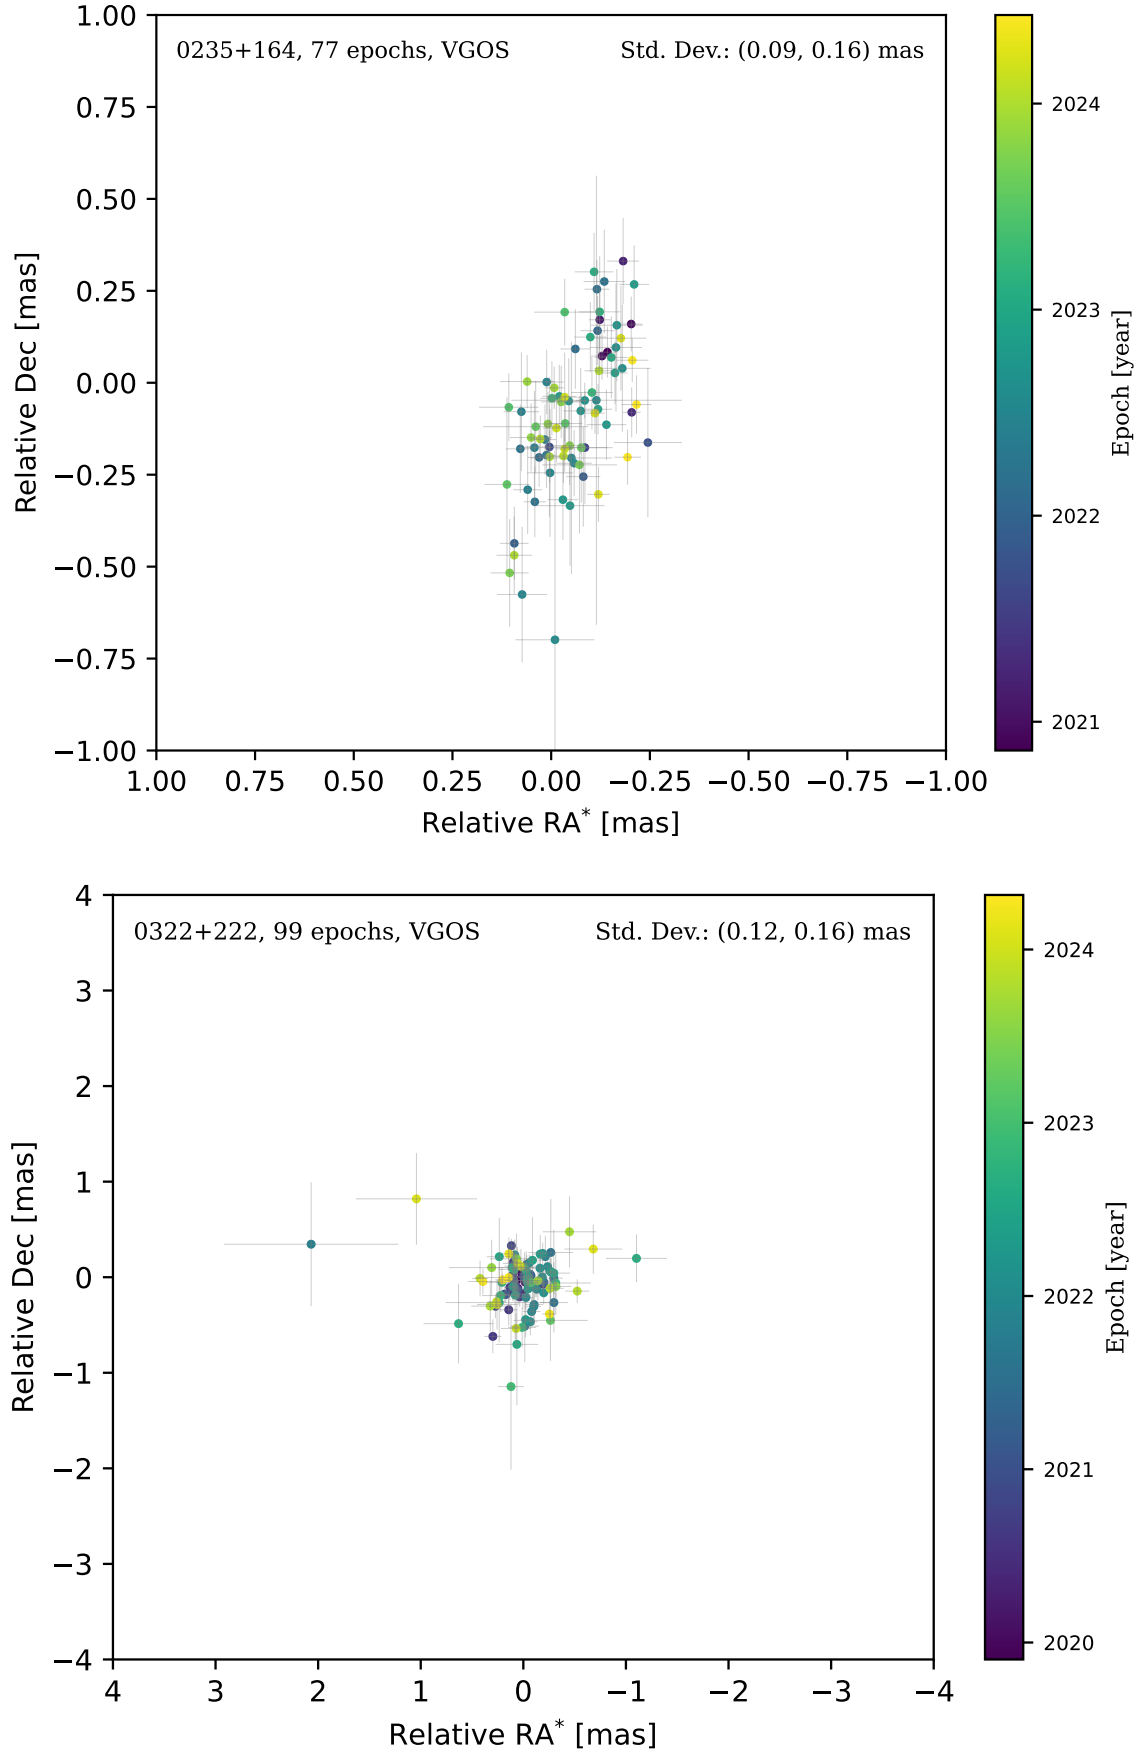

Figure 6. Position time series

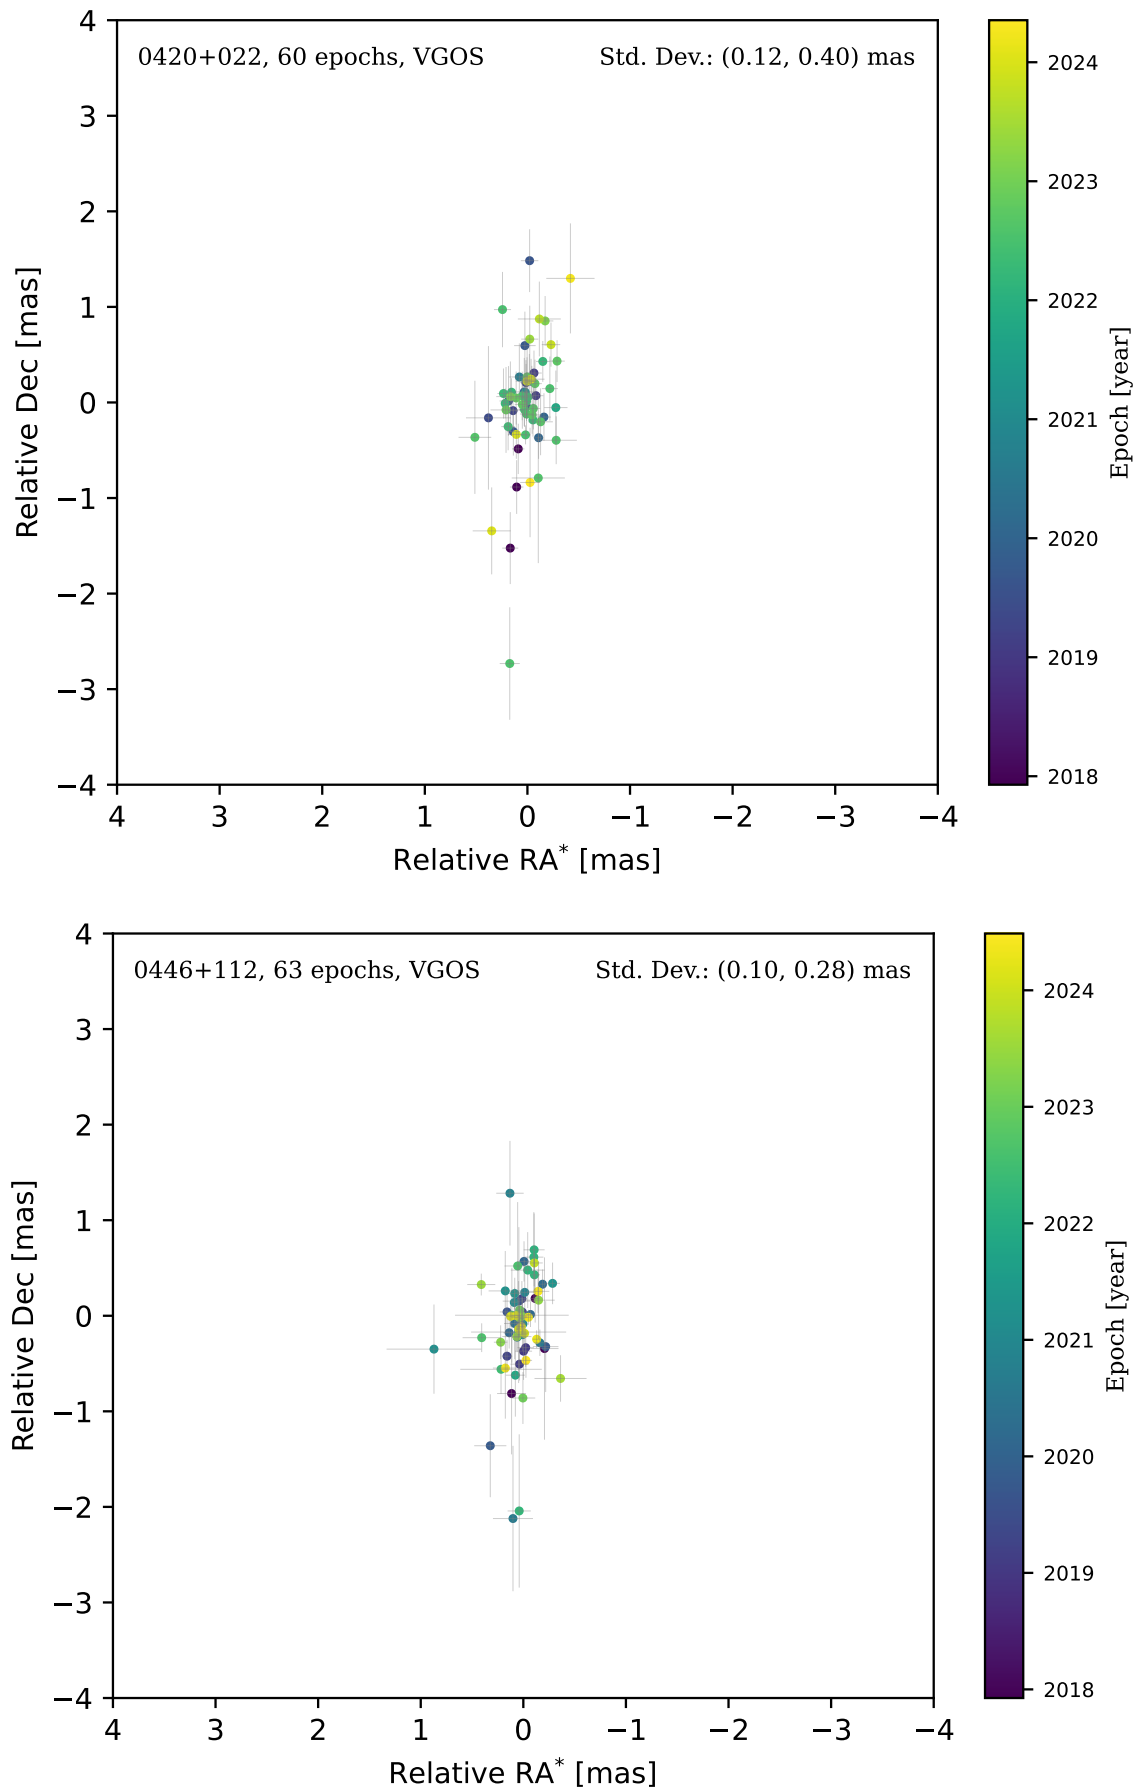

**Figure 7.** Position time series



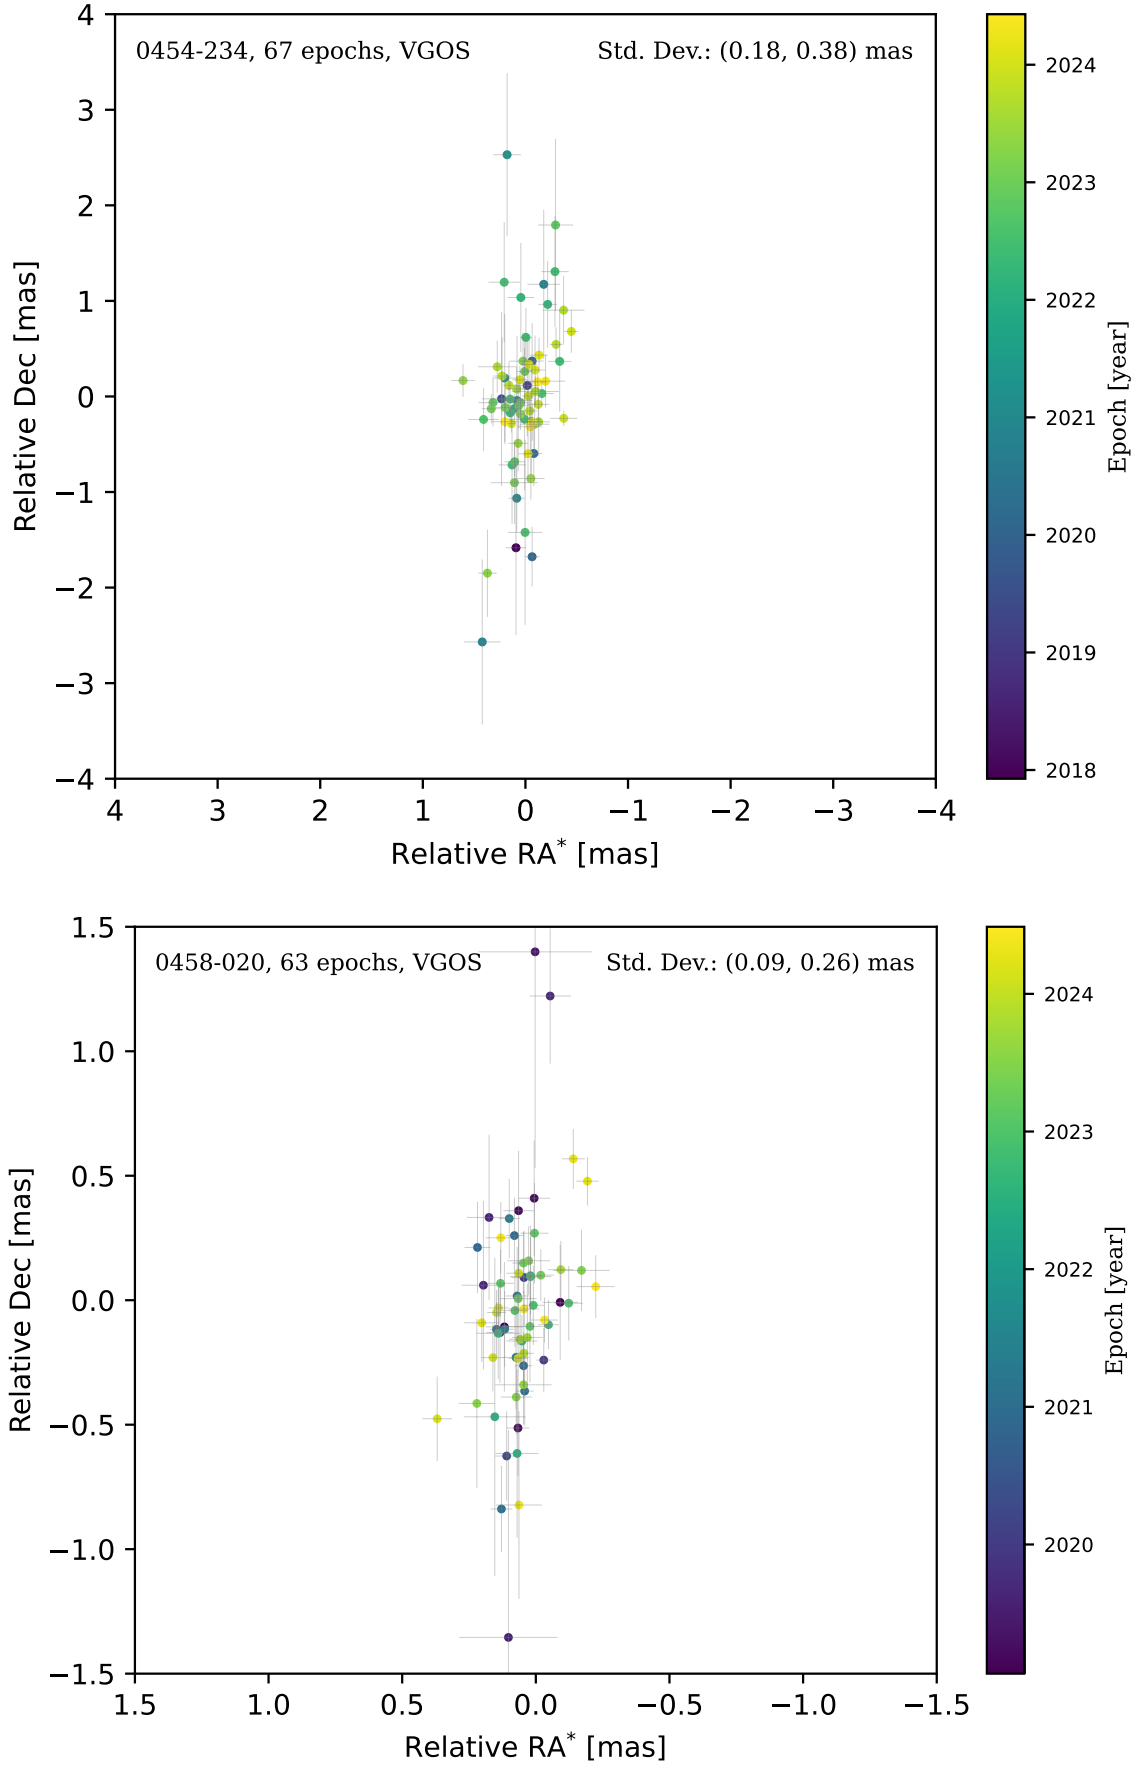

Figure 8. Position time series

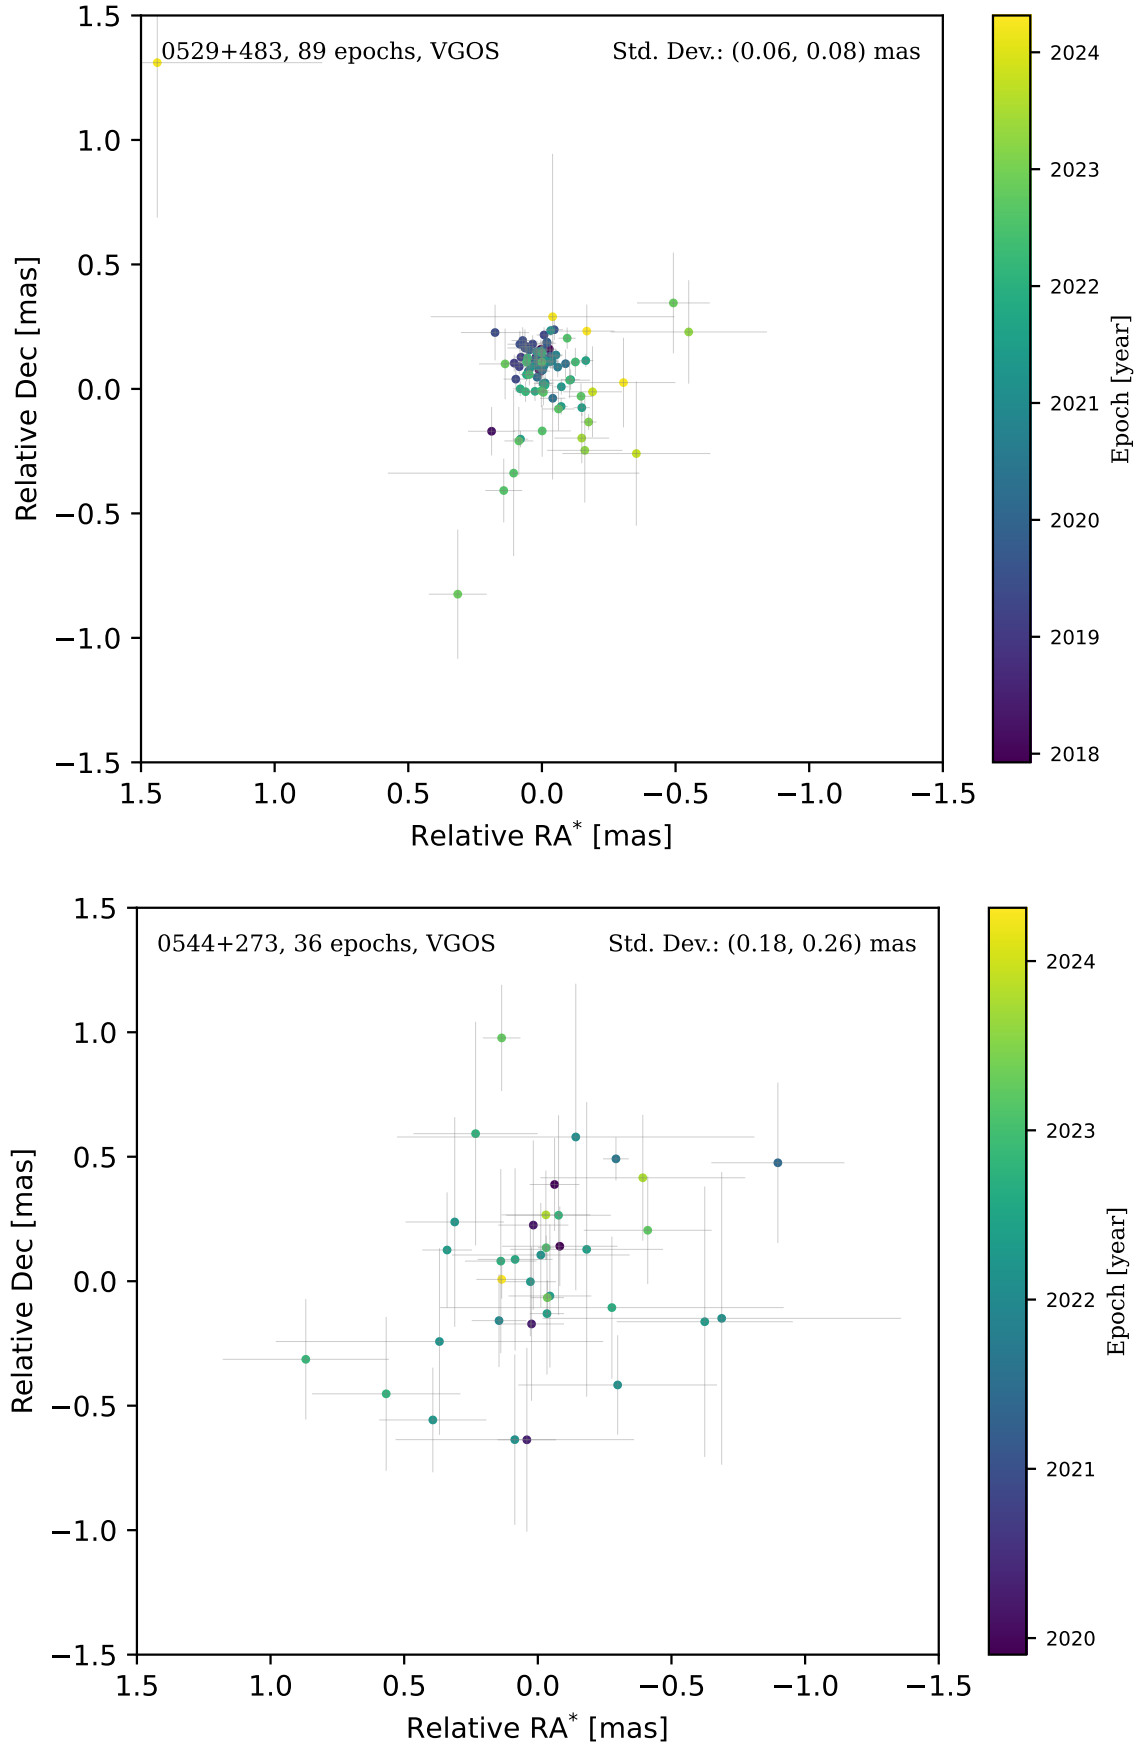

**Figure 9.** Position time series

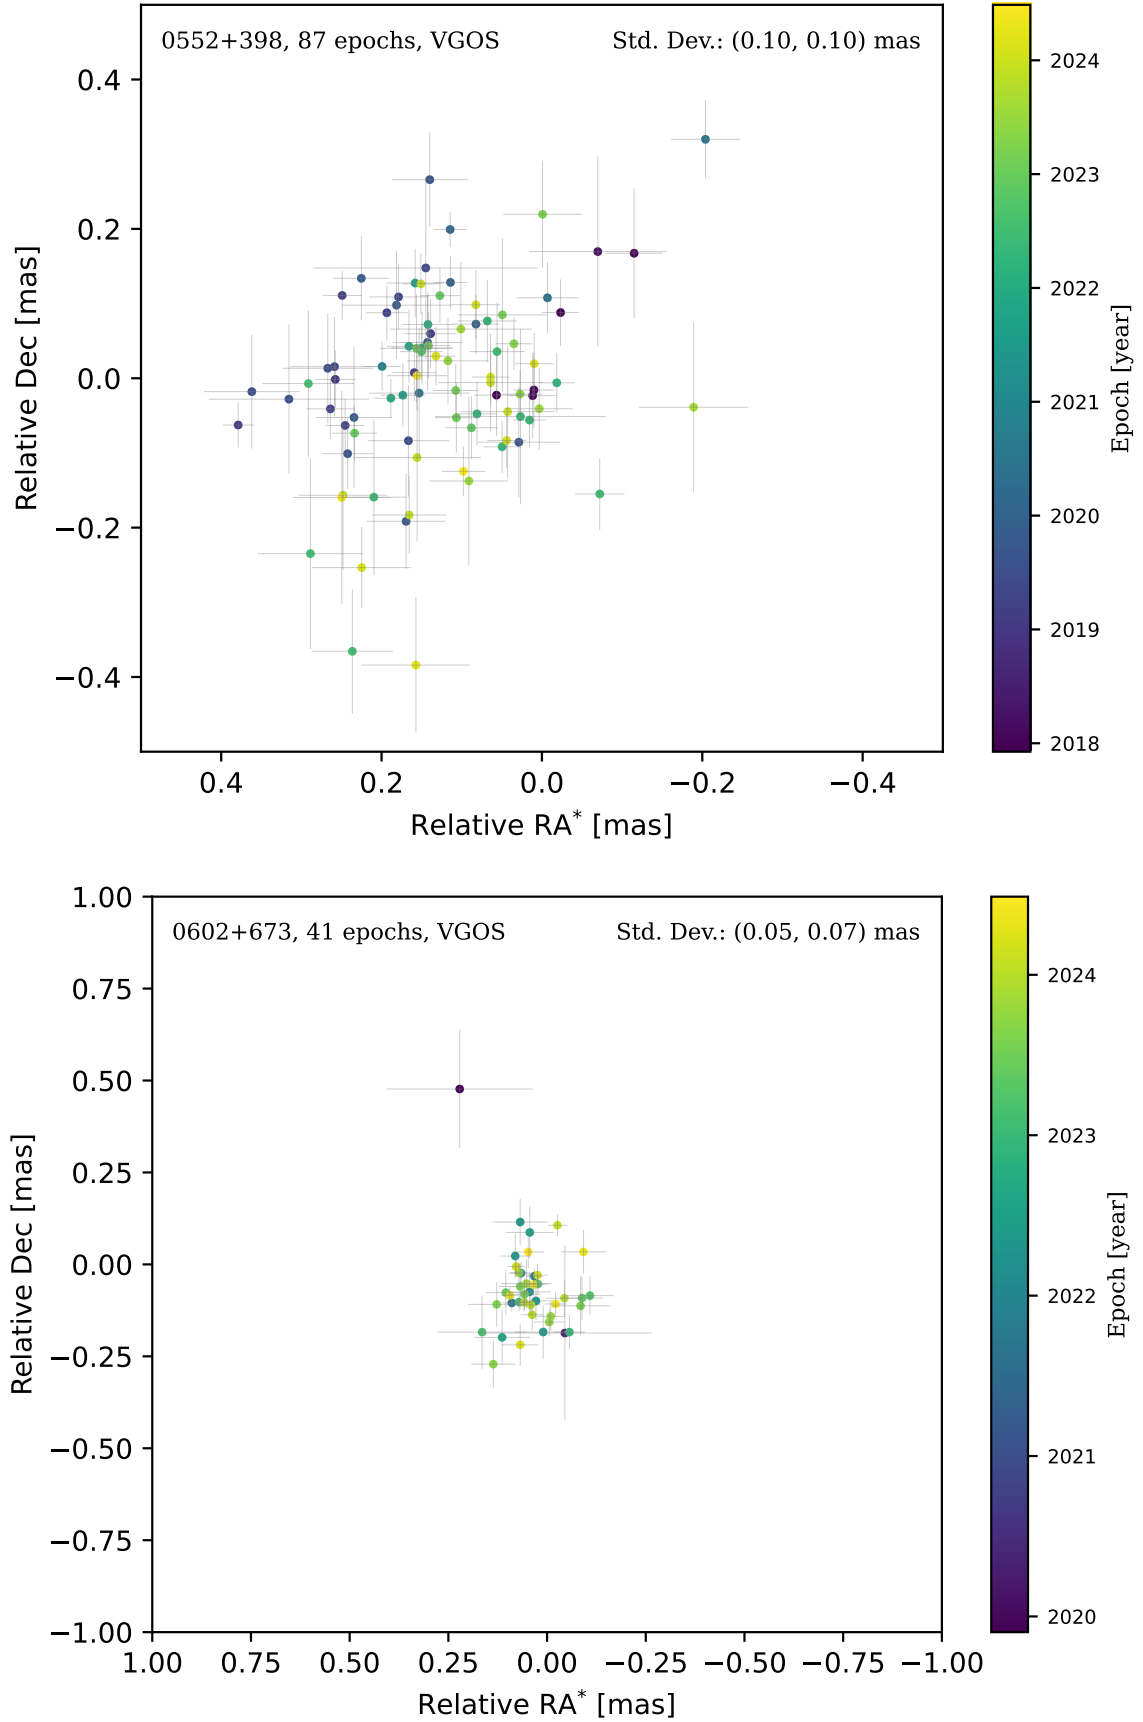

Figure 10. Position time series

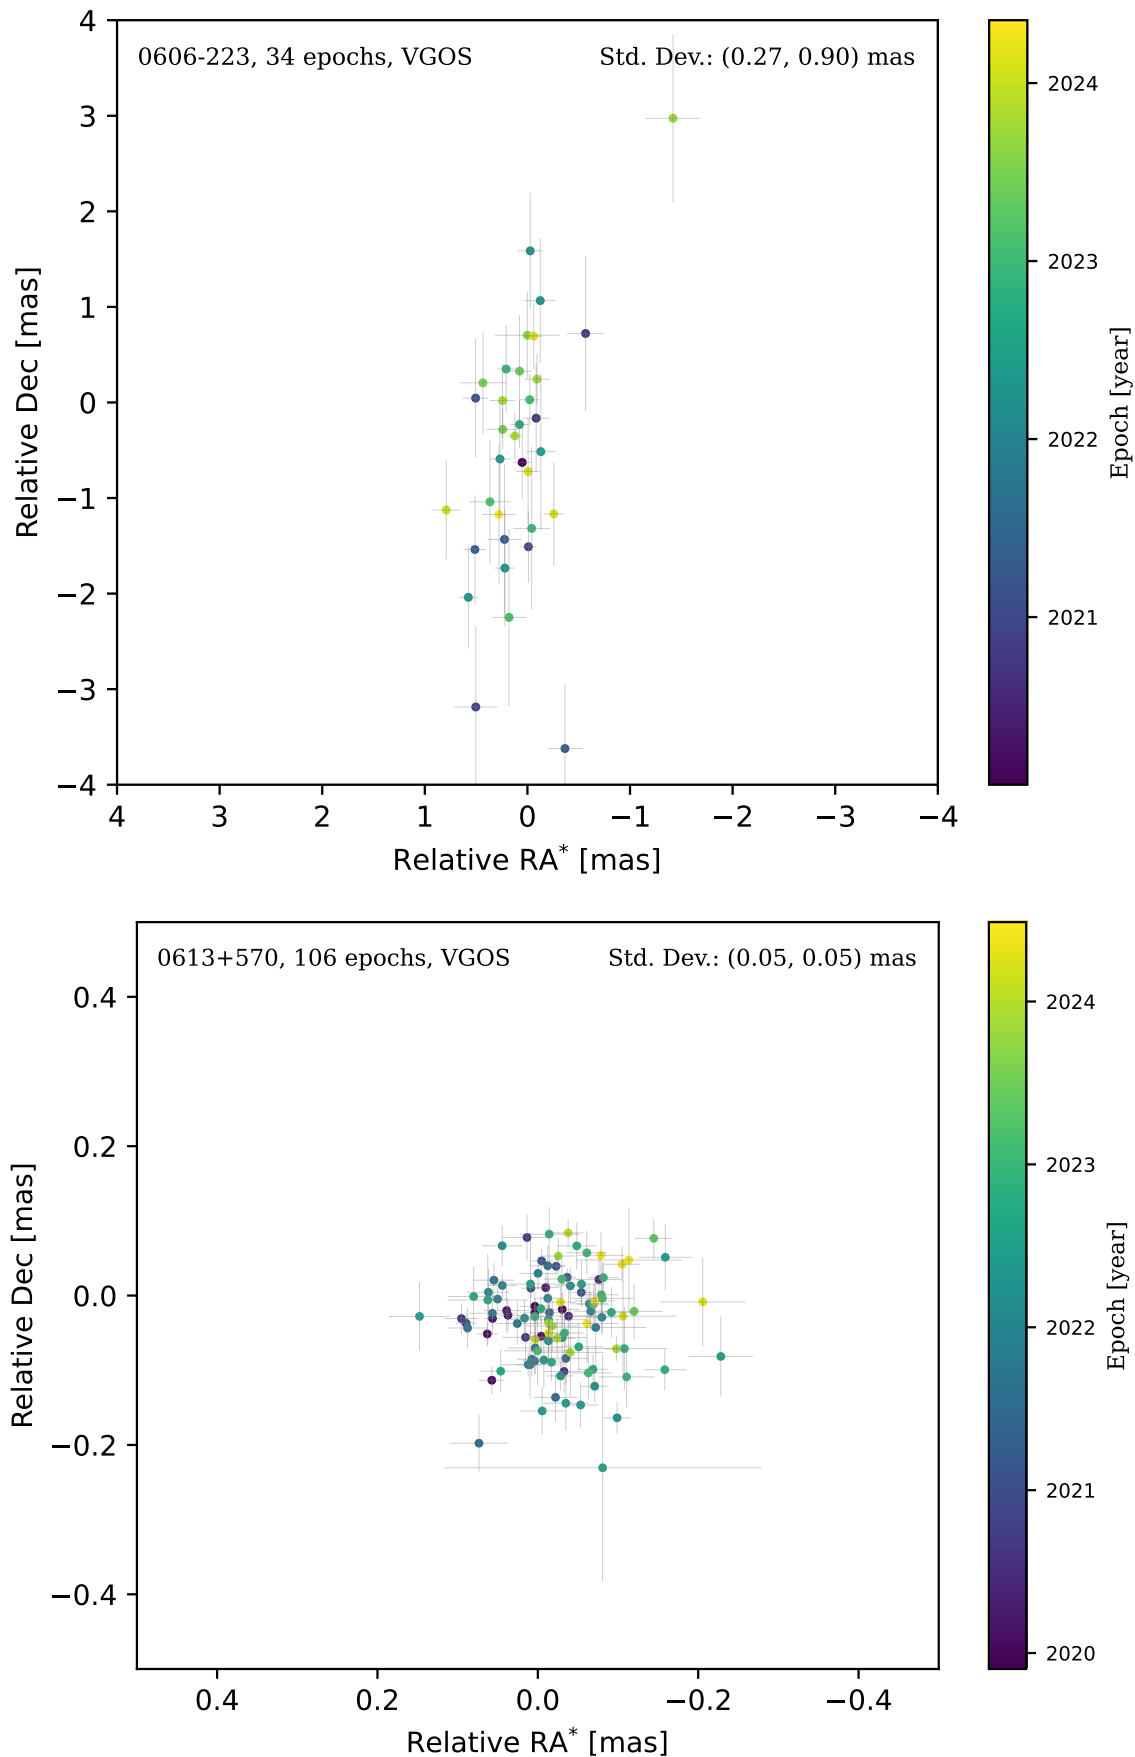

**Figure 11.** Position time series

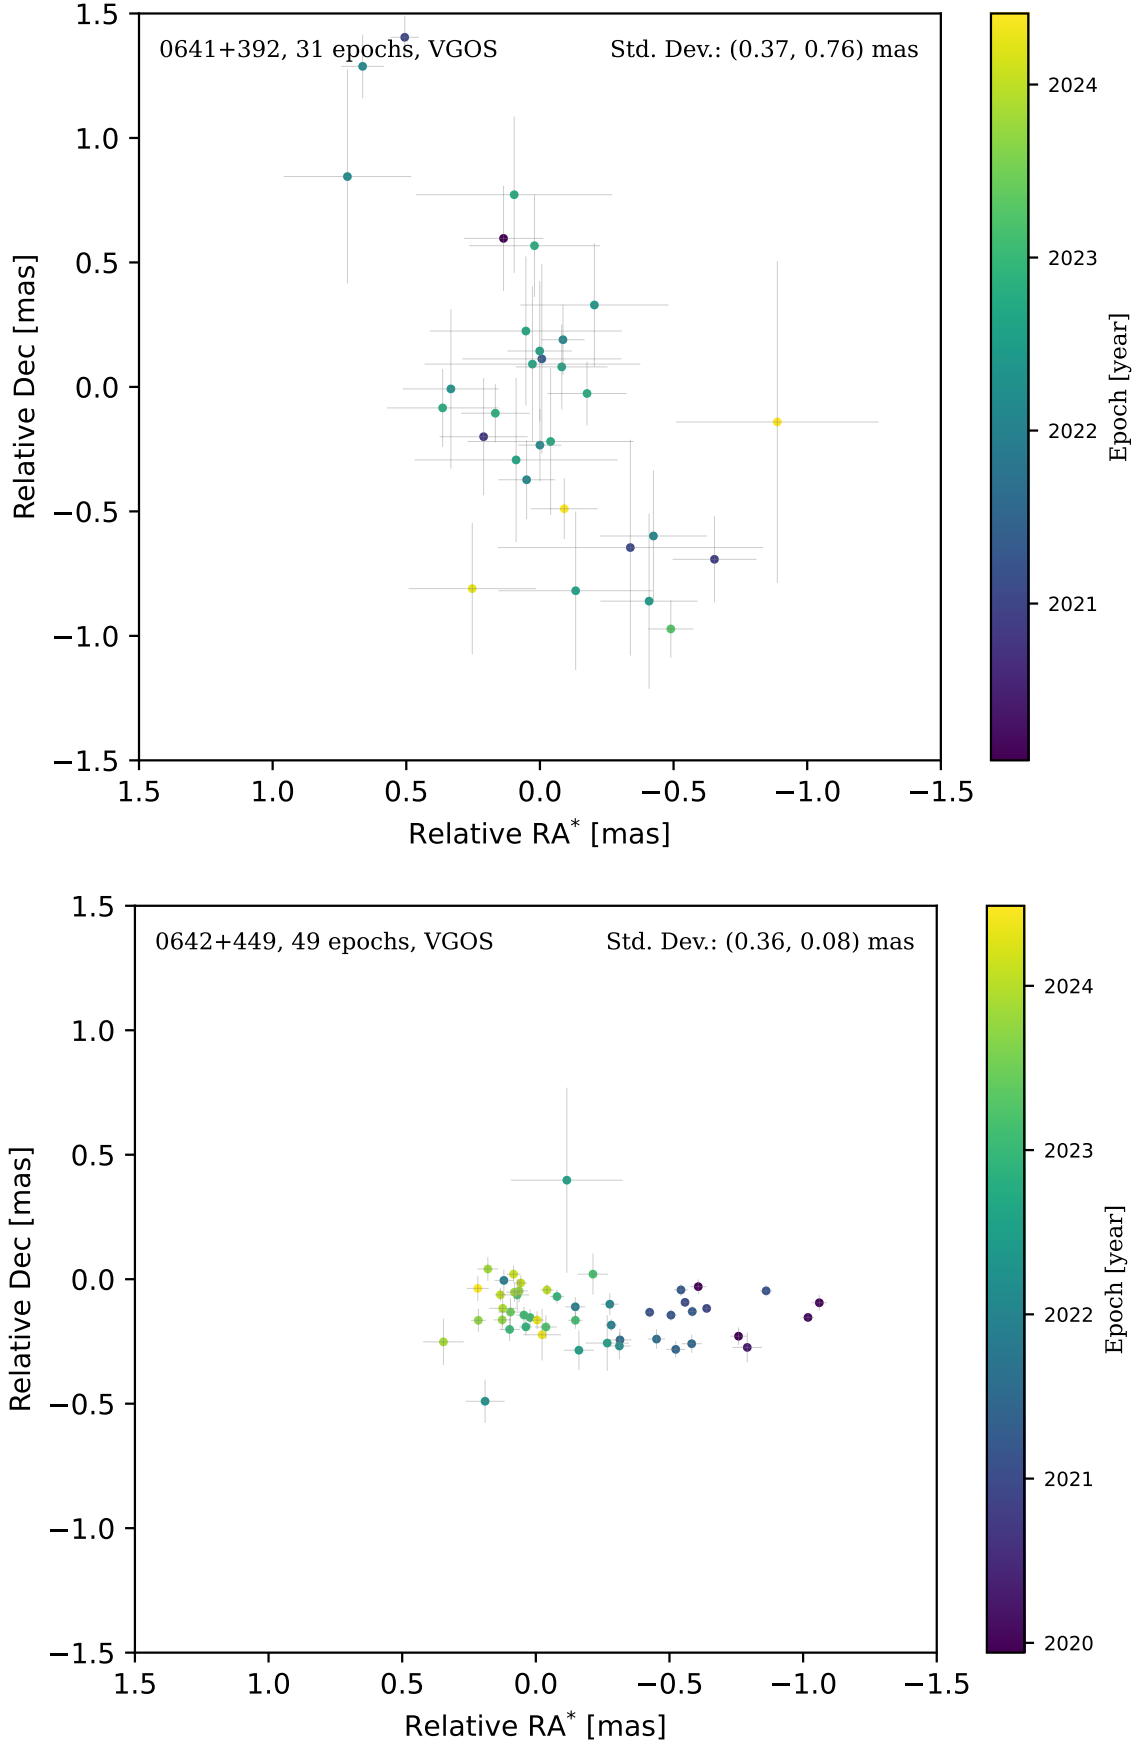

Figure 12. Position time series

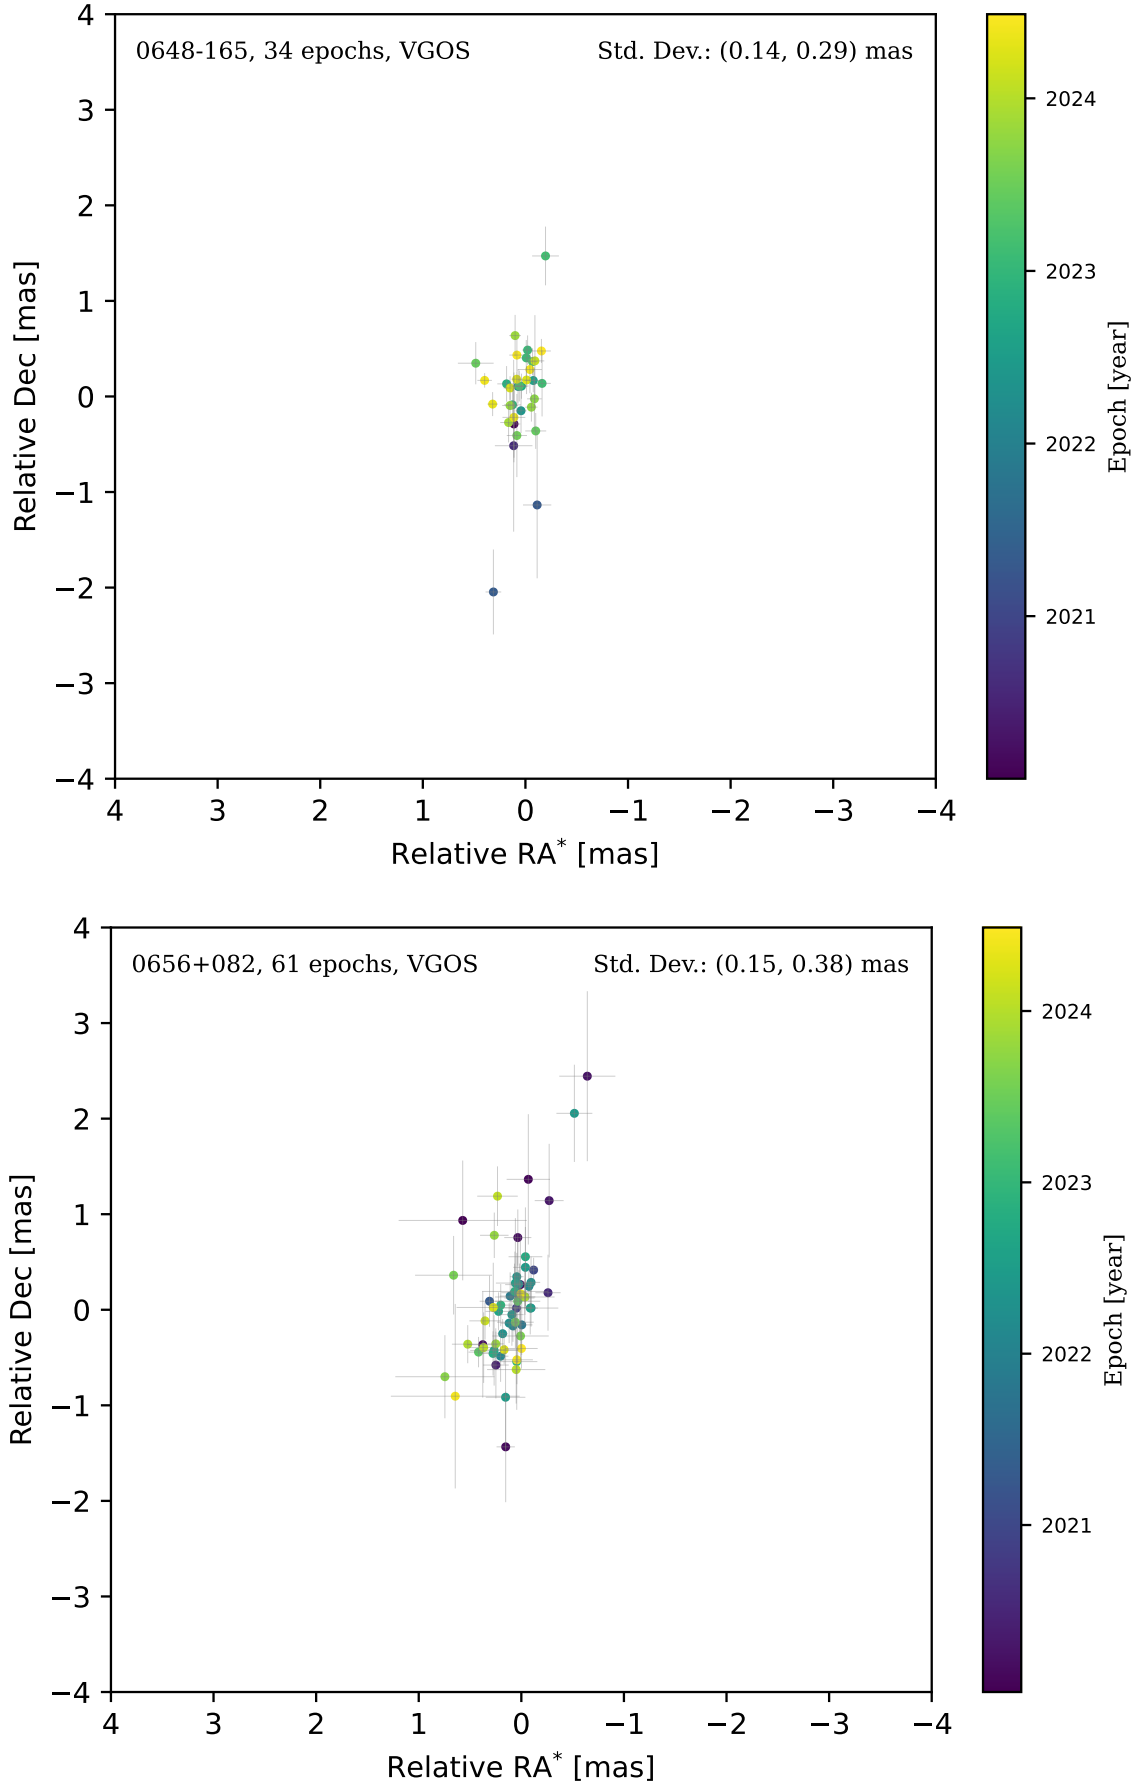

**Figure 13.** Position time series

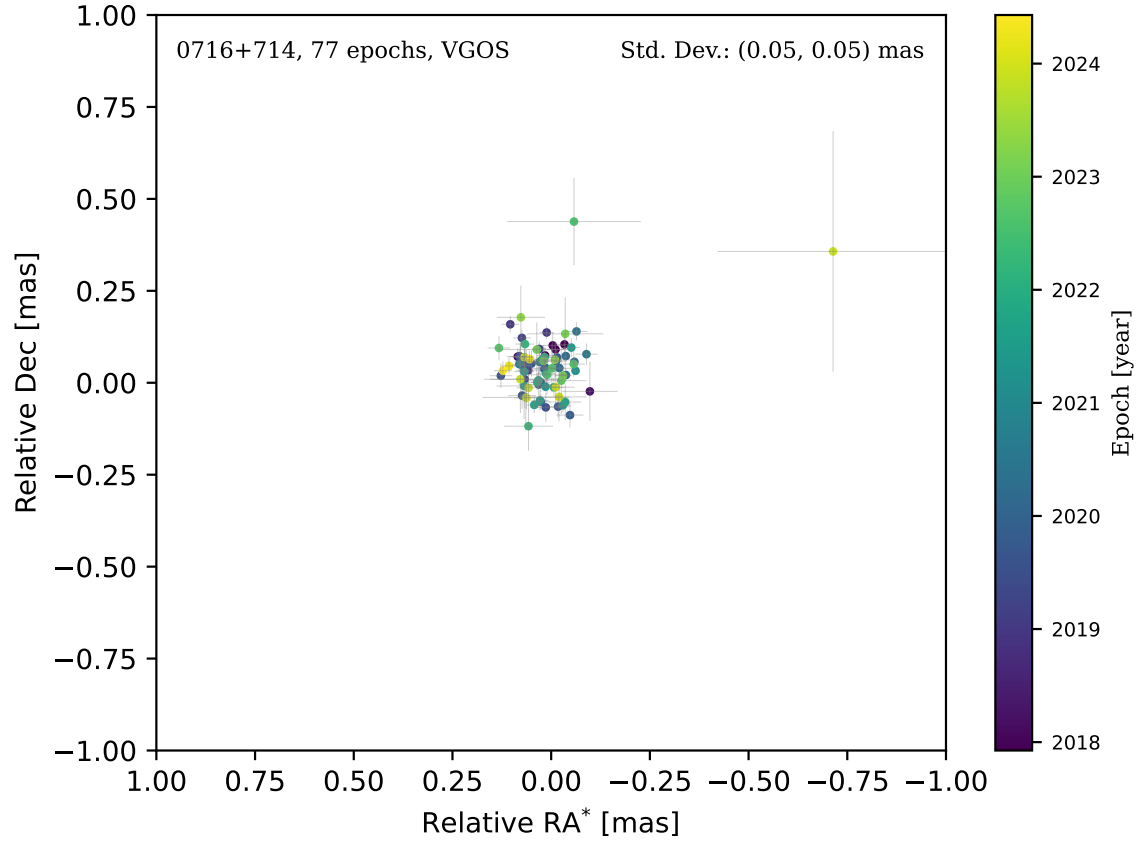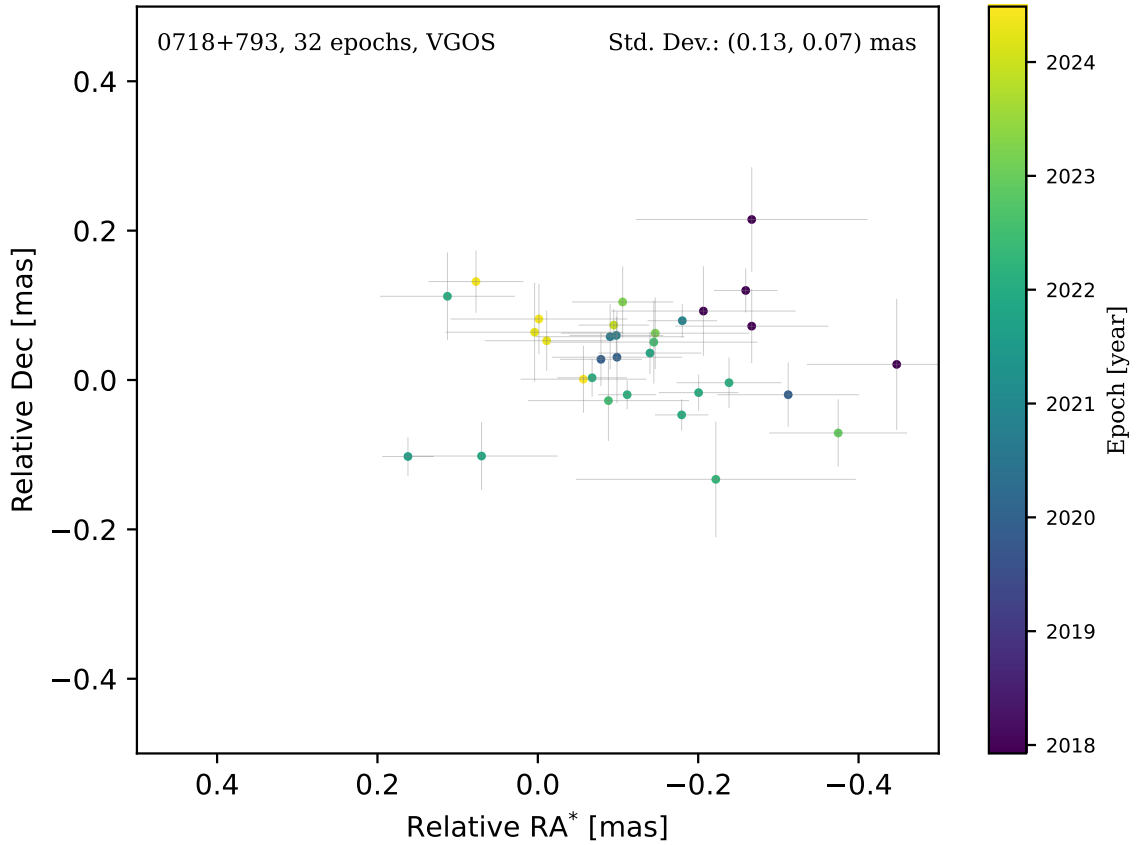

Figure 14. Position time series

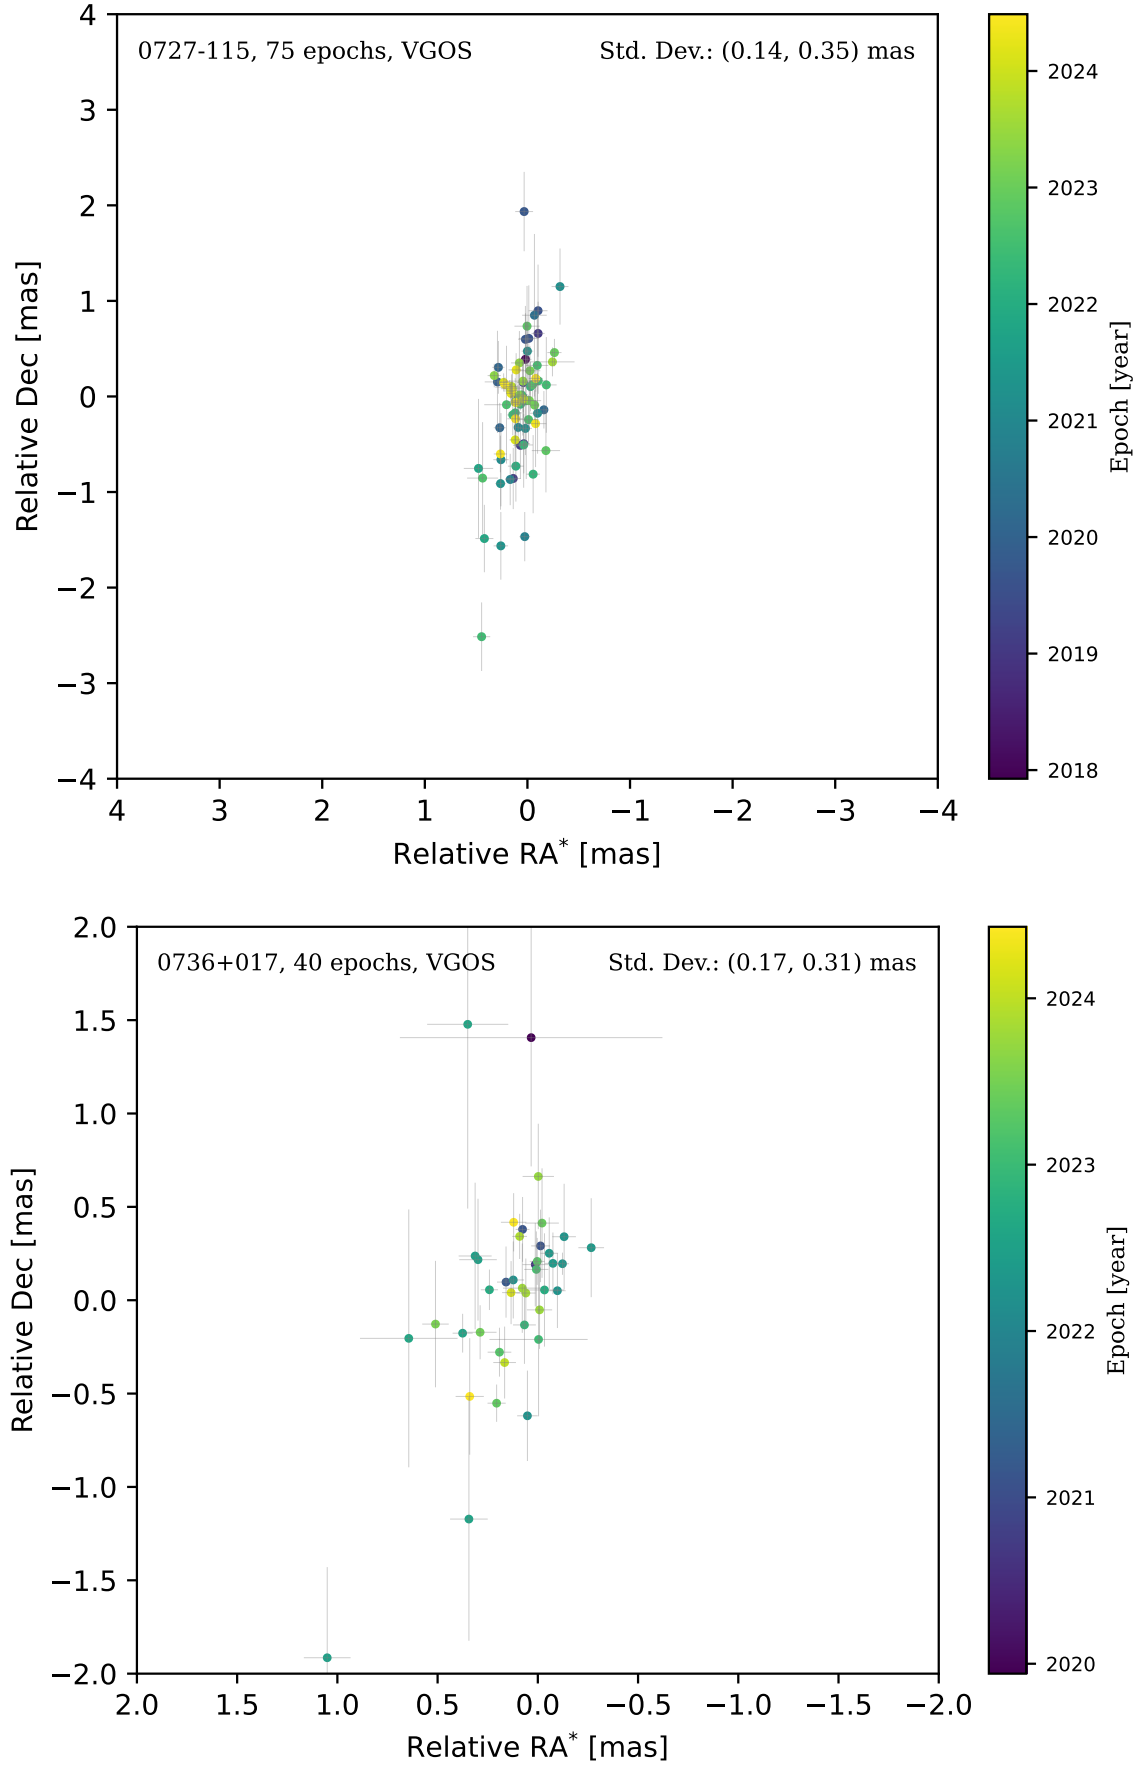

Figure 15. Position time series



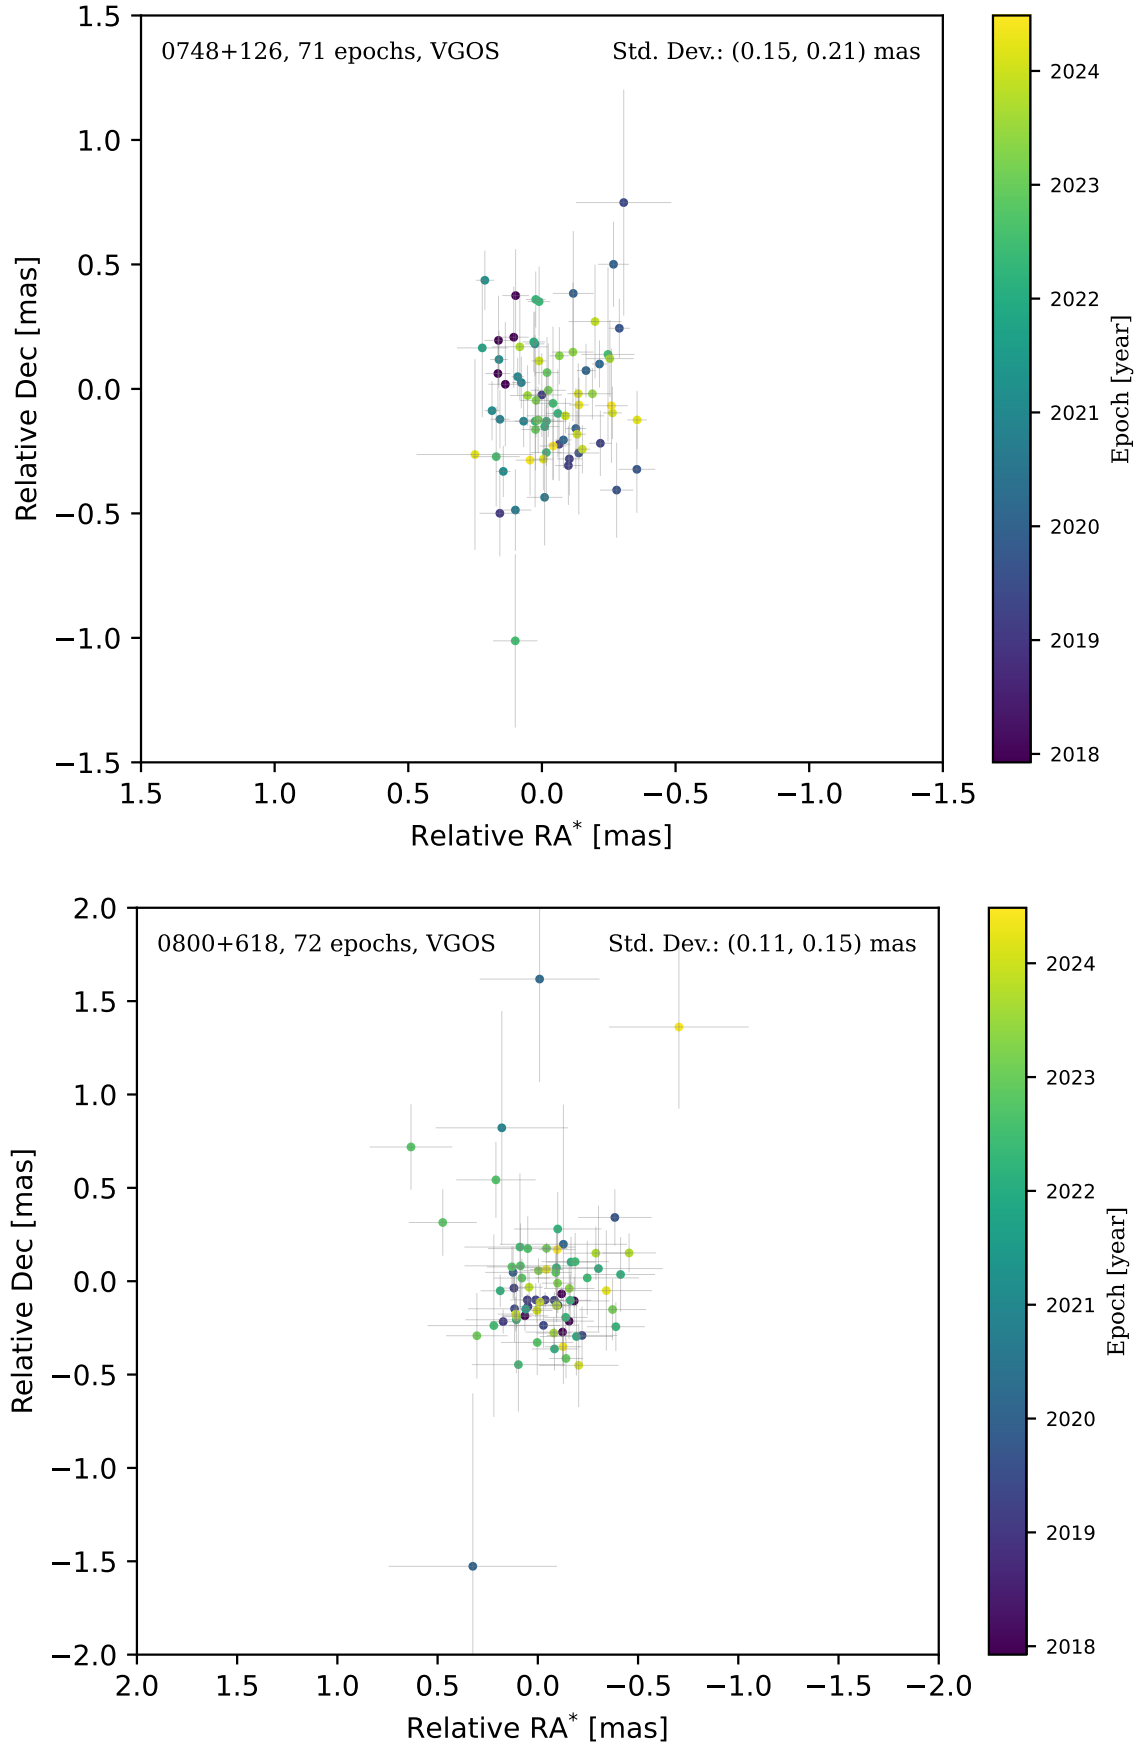

Figure 16. Position time series

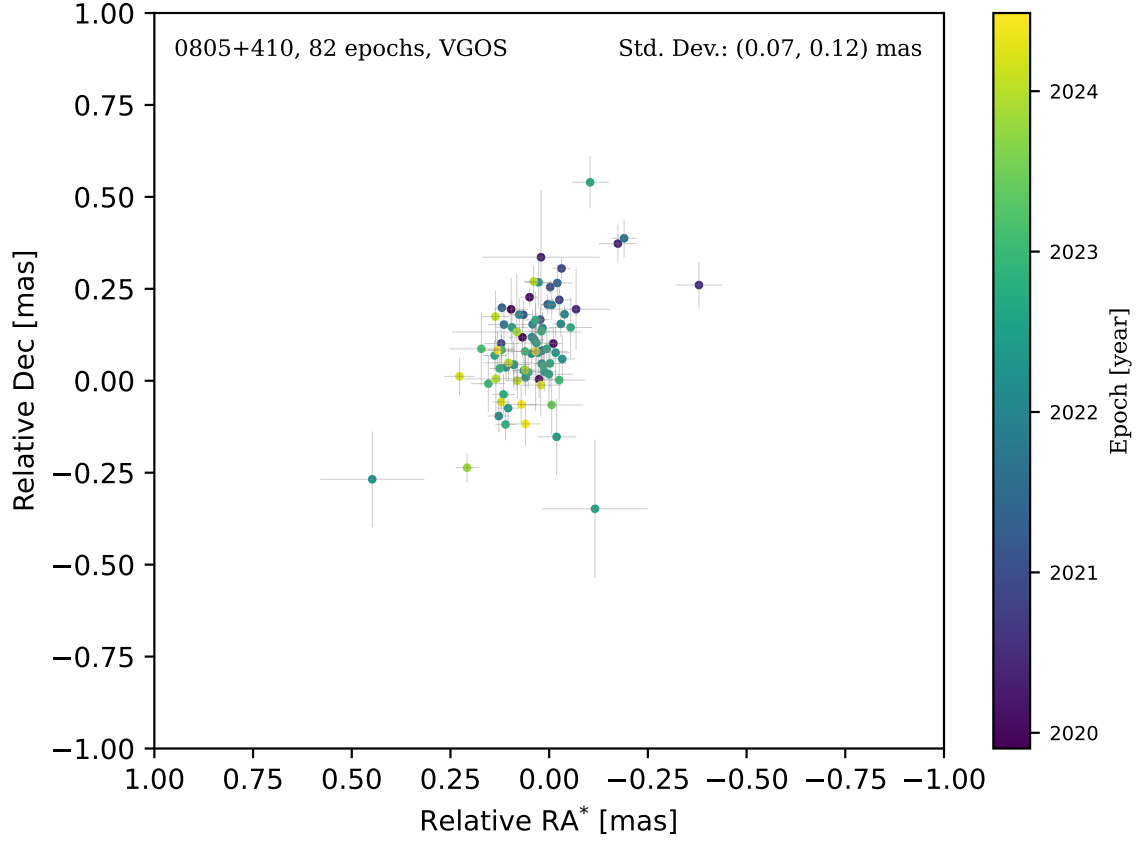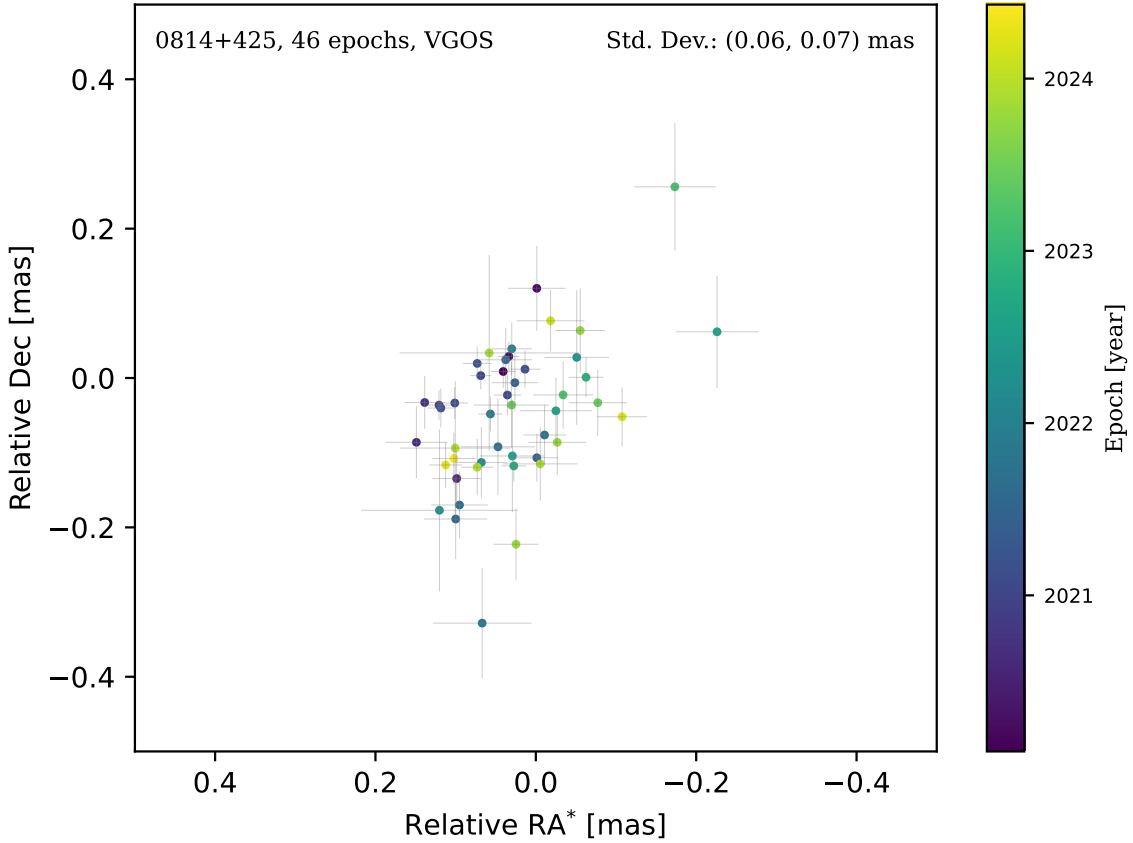

**Figure 17.** Position time series

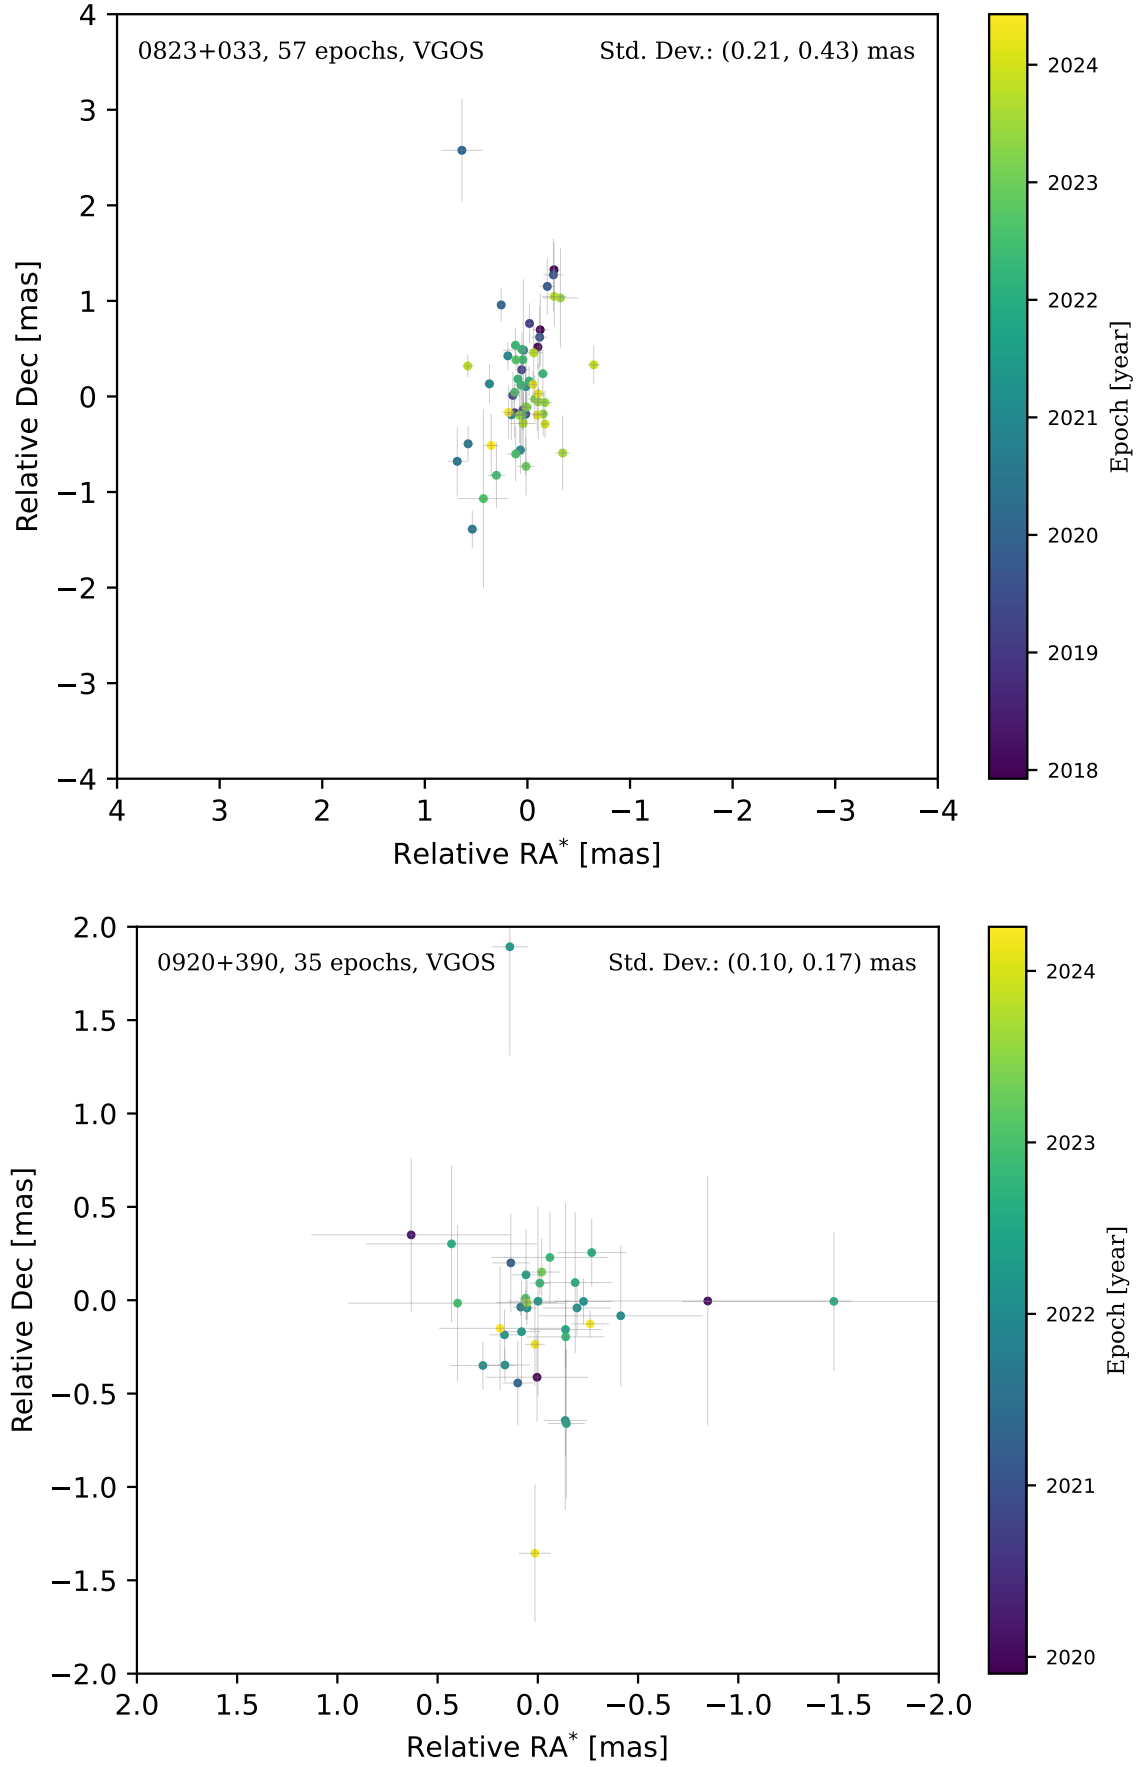

Figure 18. Position time series

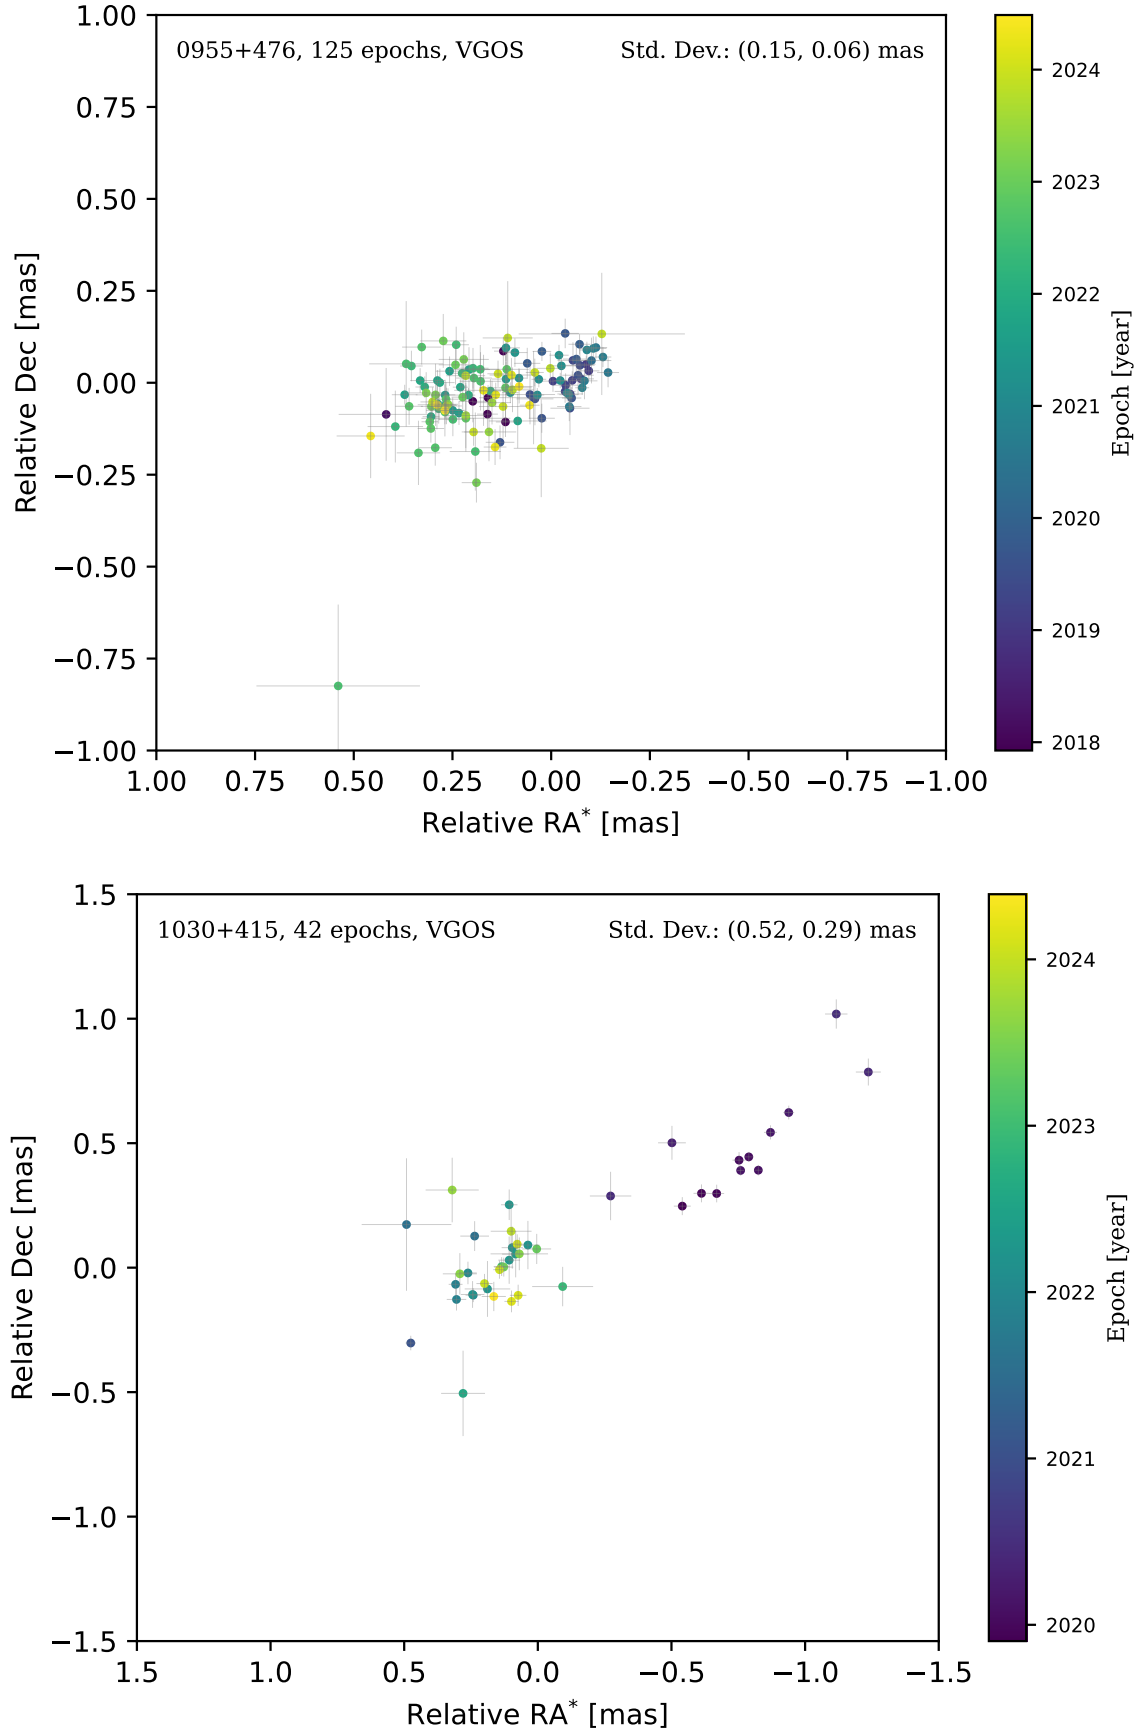

**Figure 19.** Position time series

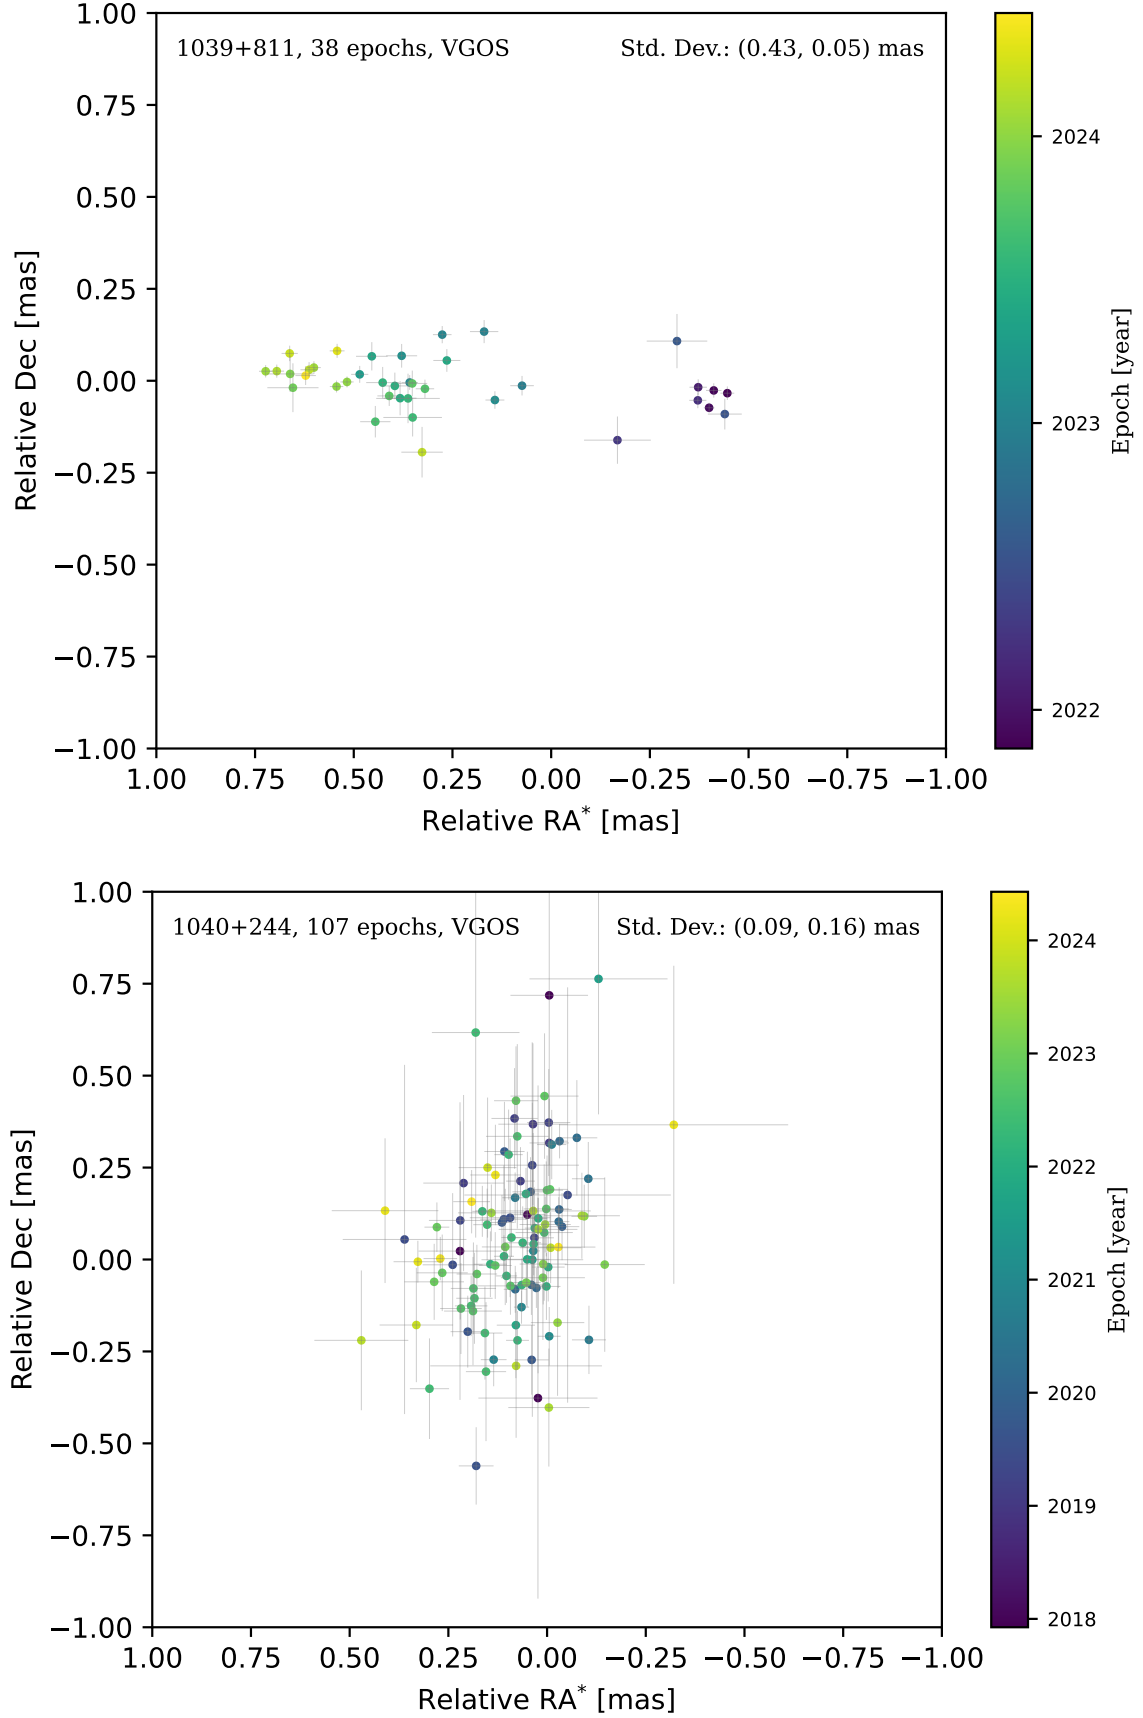**Figure 20.** Position time series

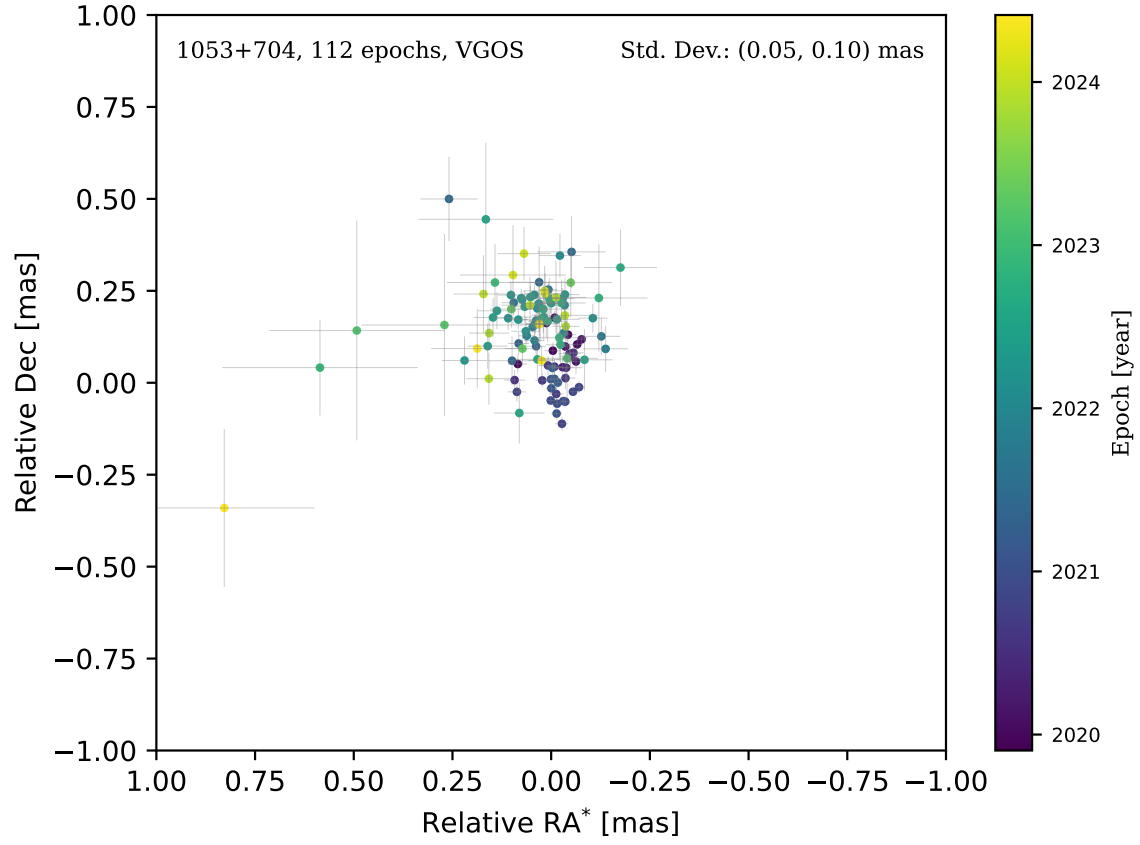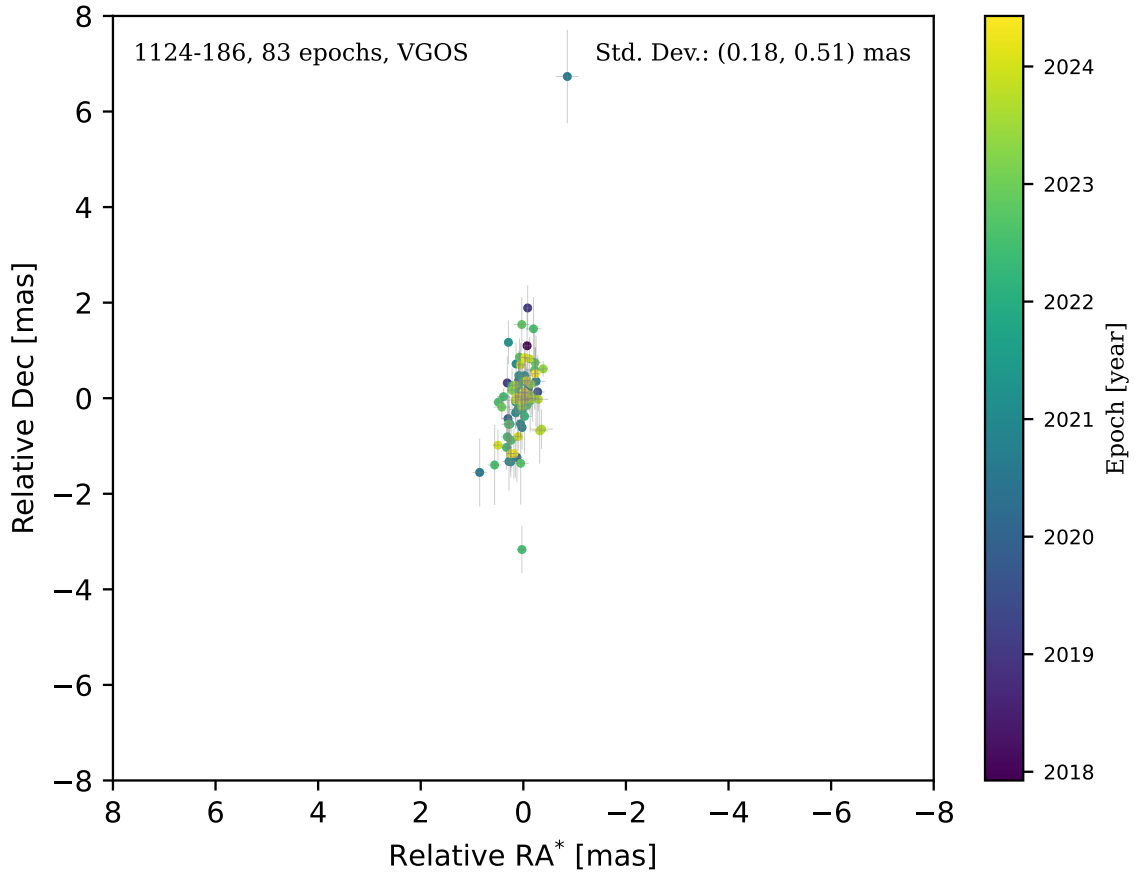

**Figure 21.** Position time series

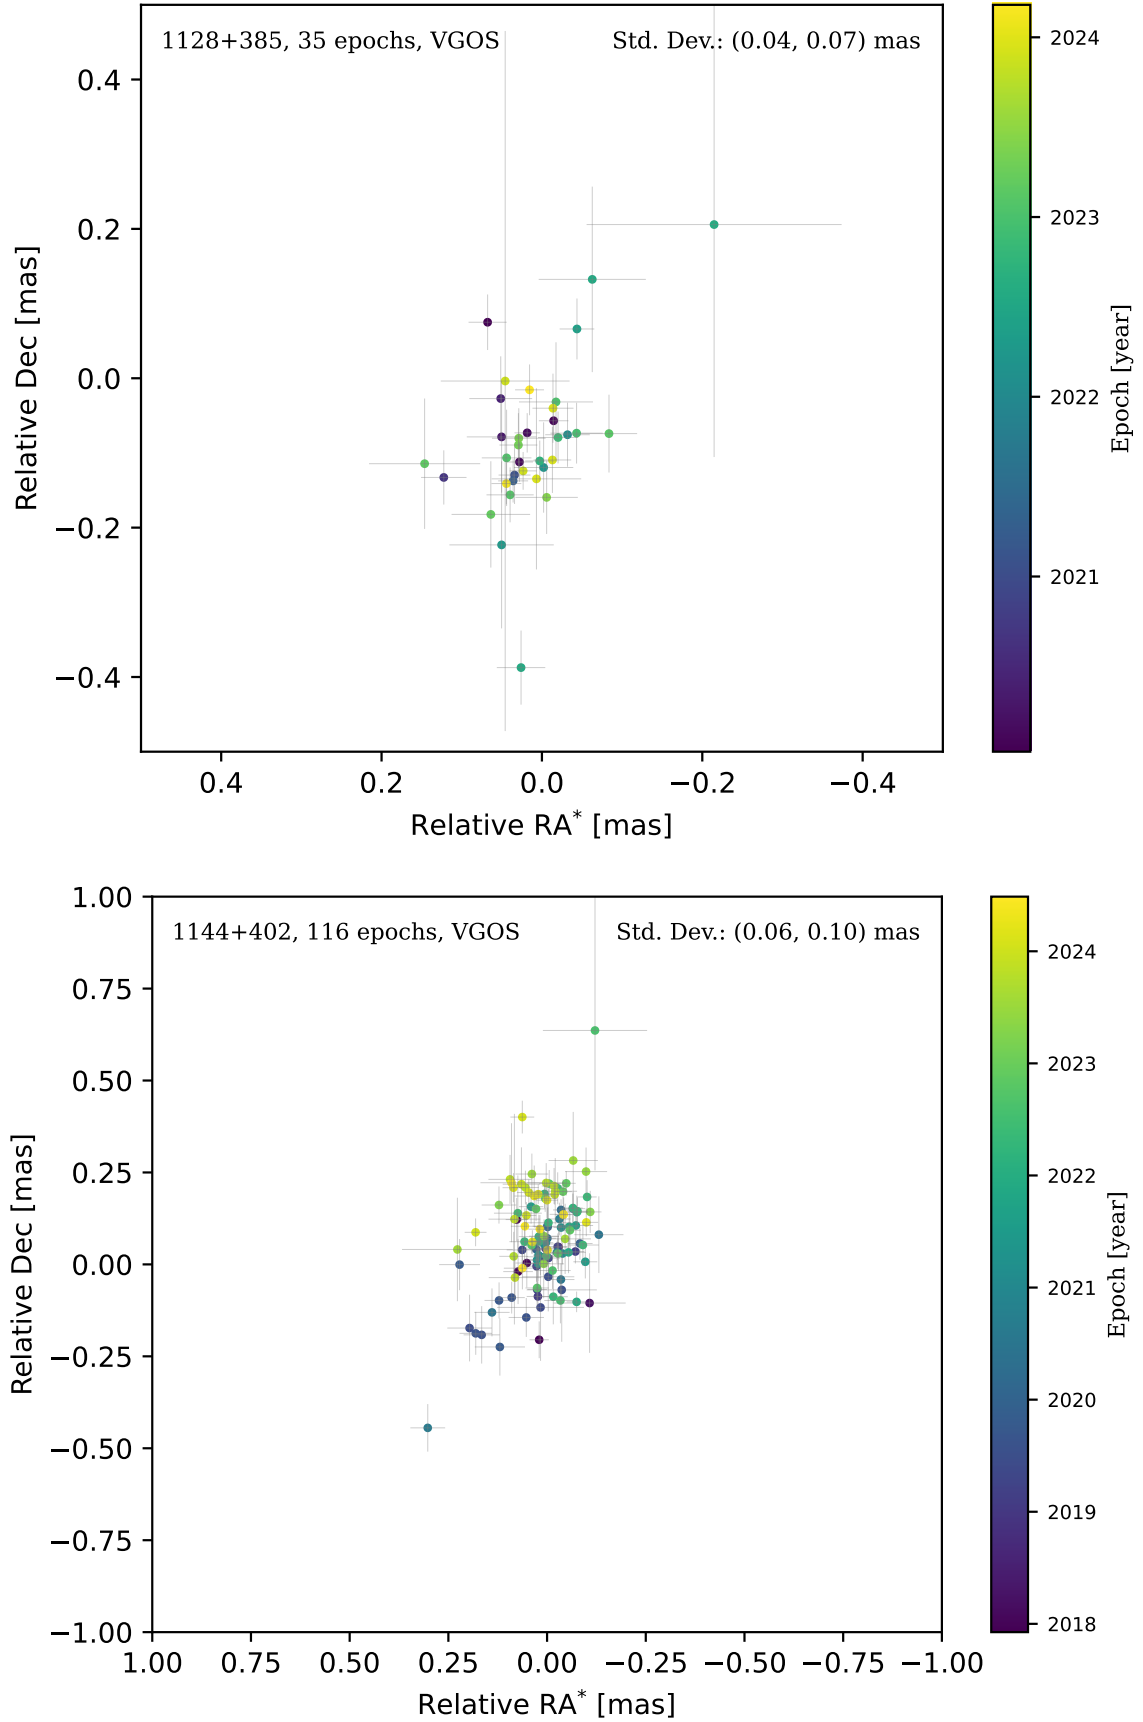**Figure 22.** Position time series

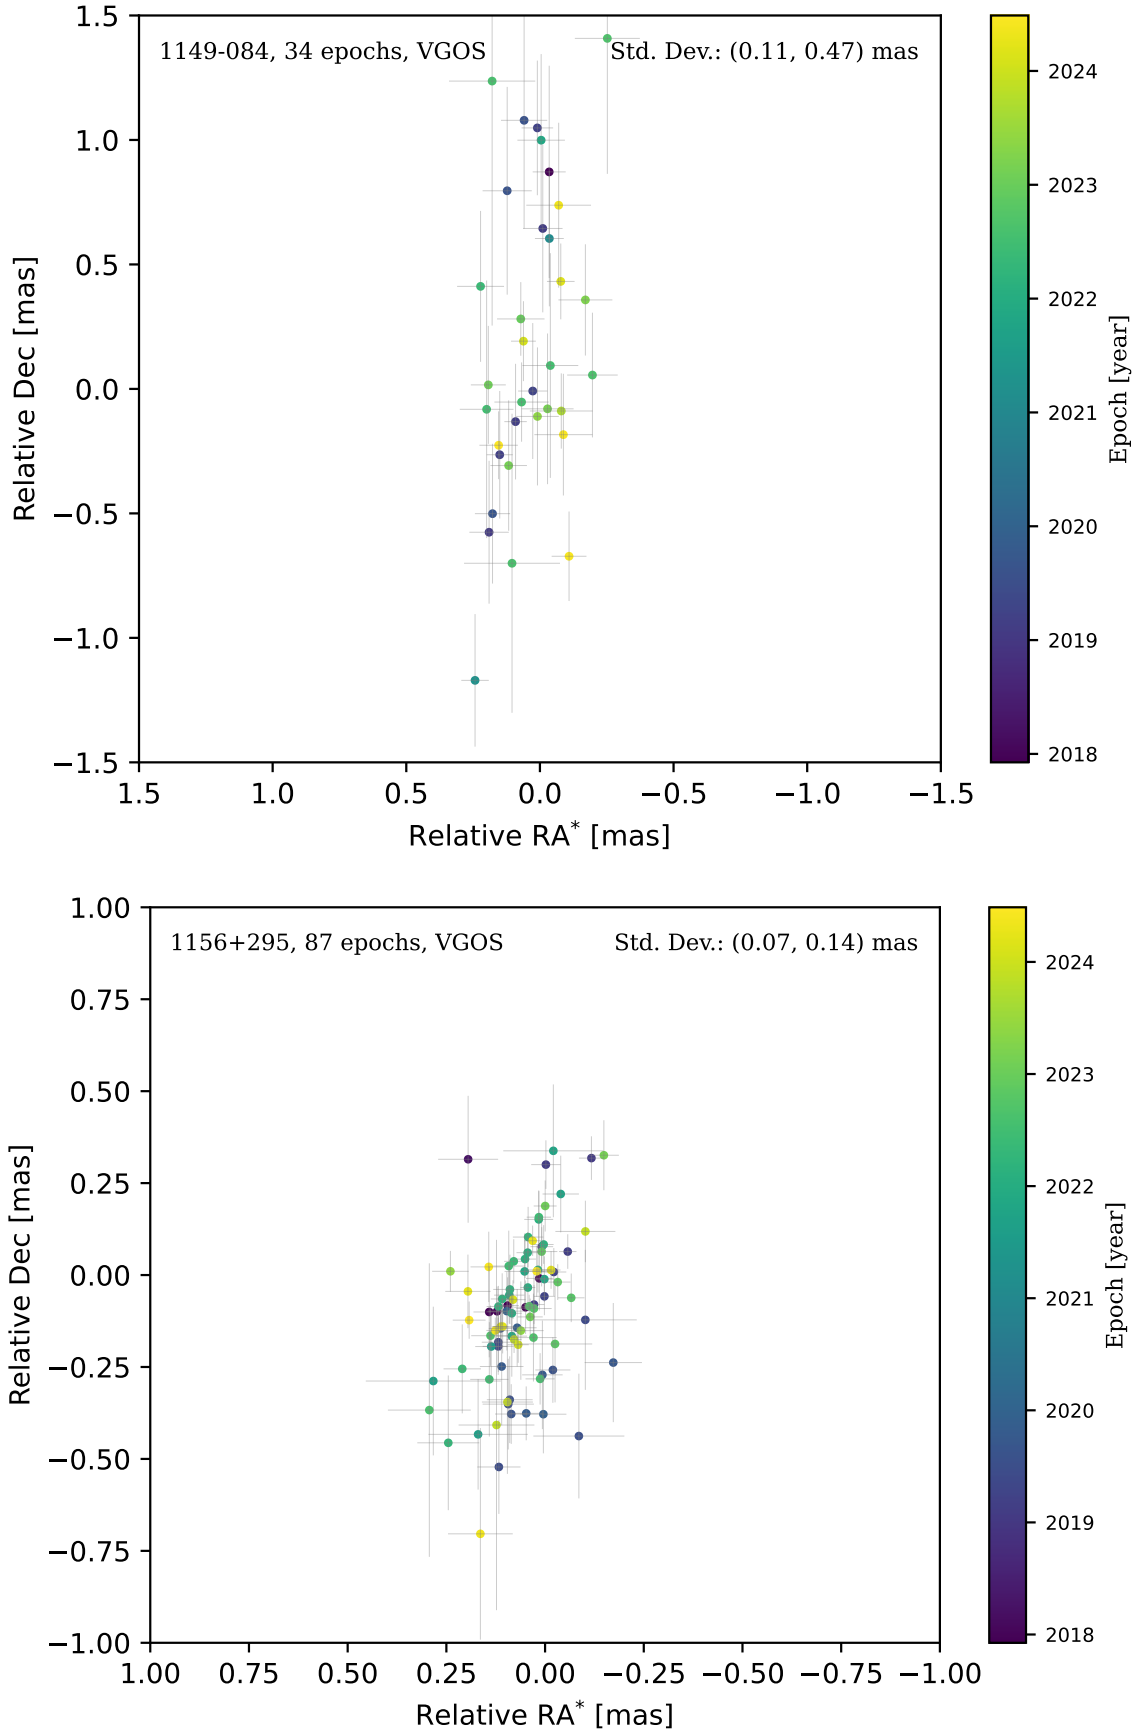

**Figure 23.** Position time series



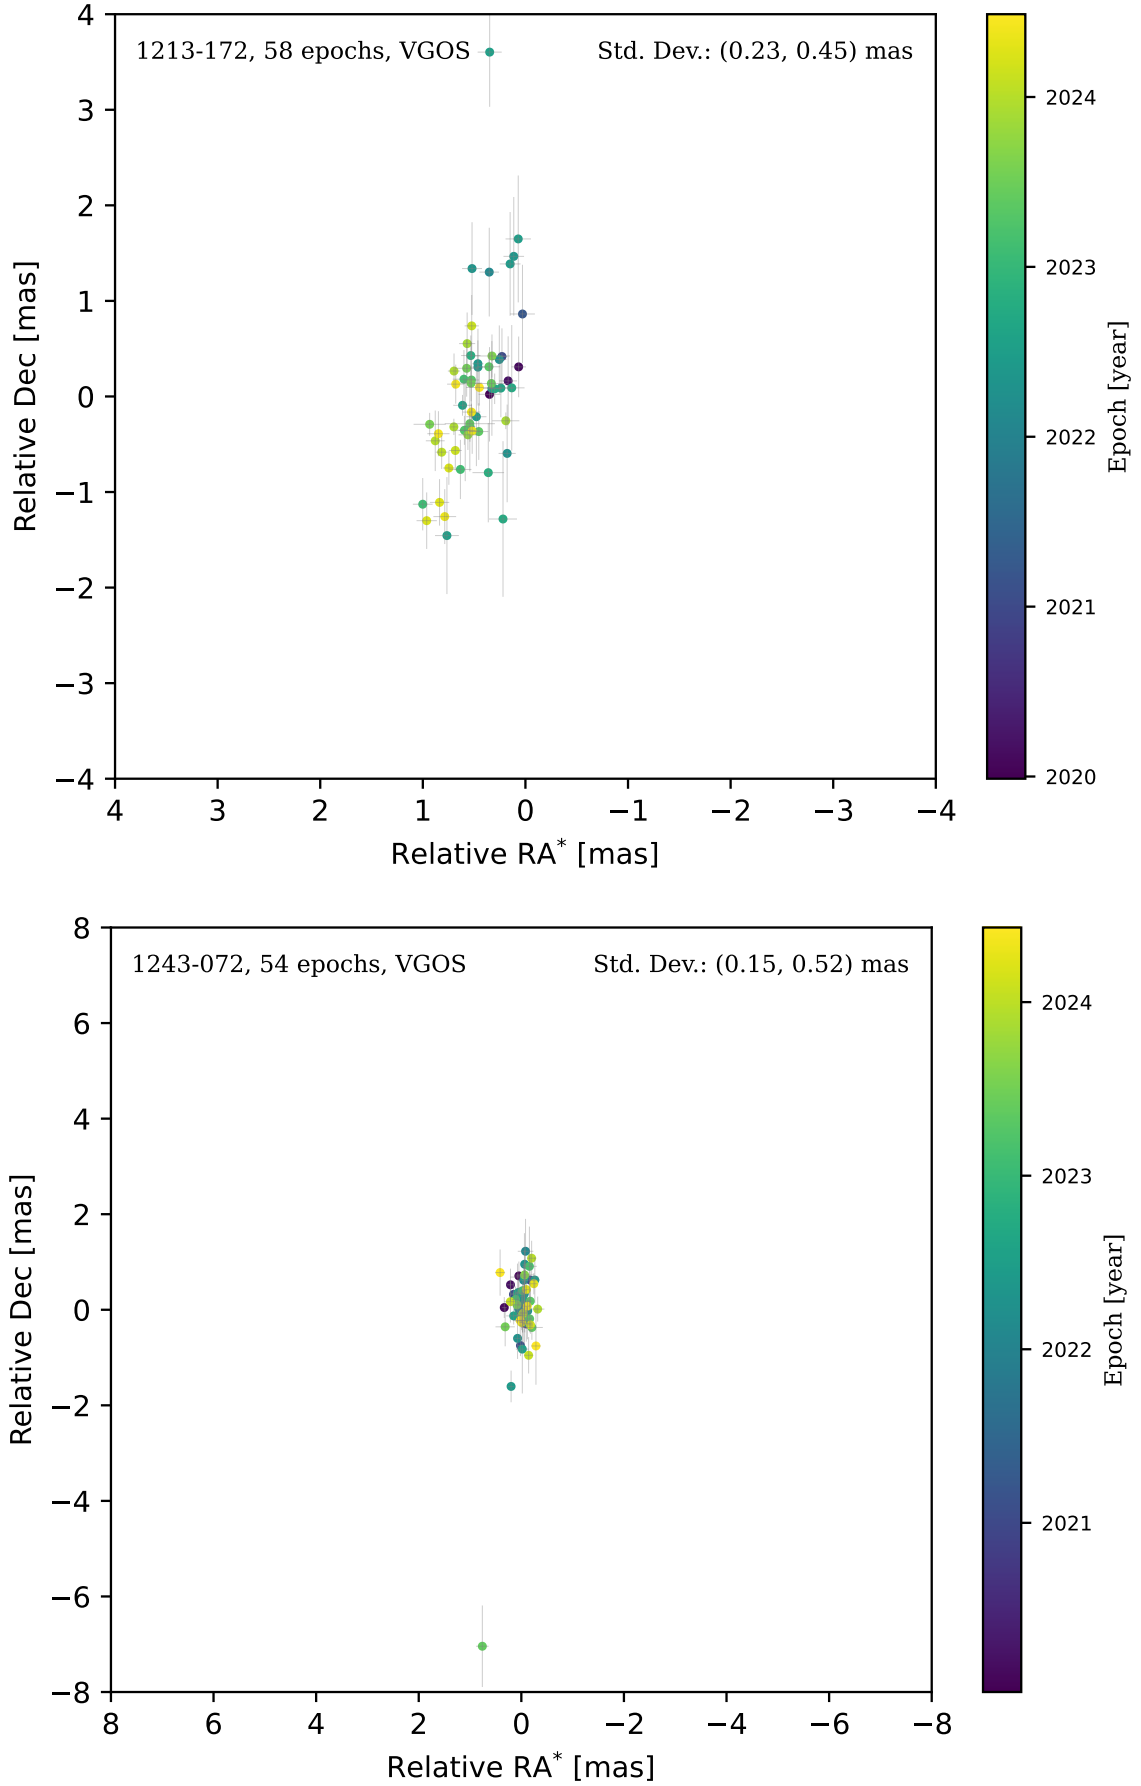**Figure 24.** Position time series

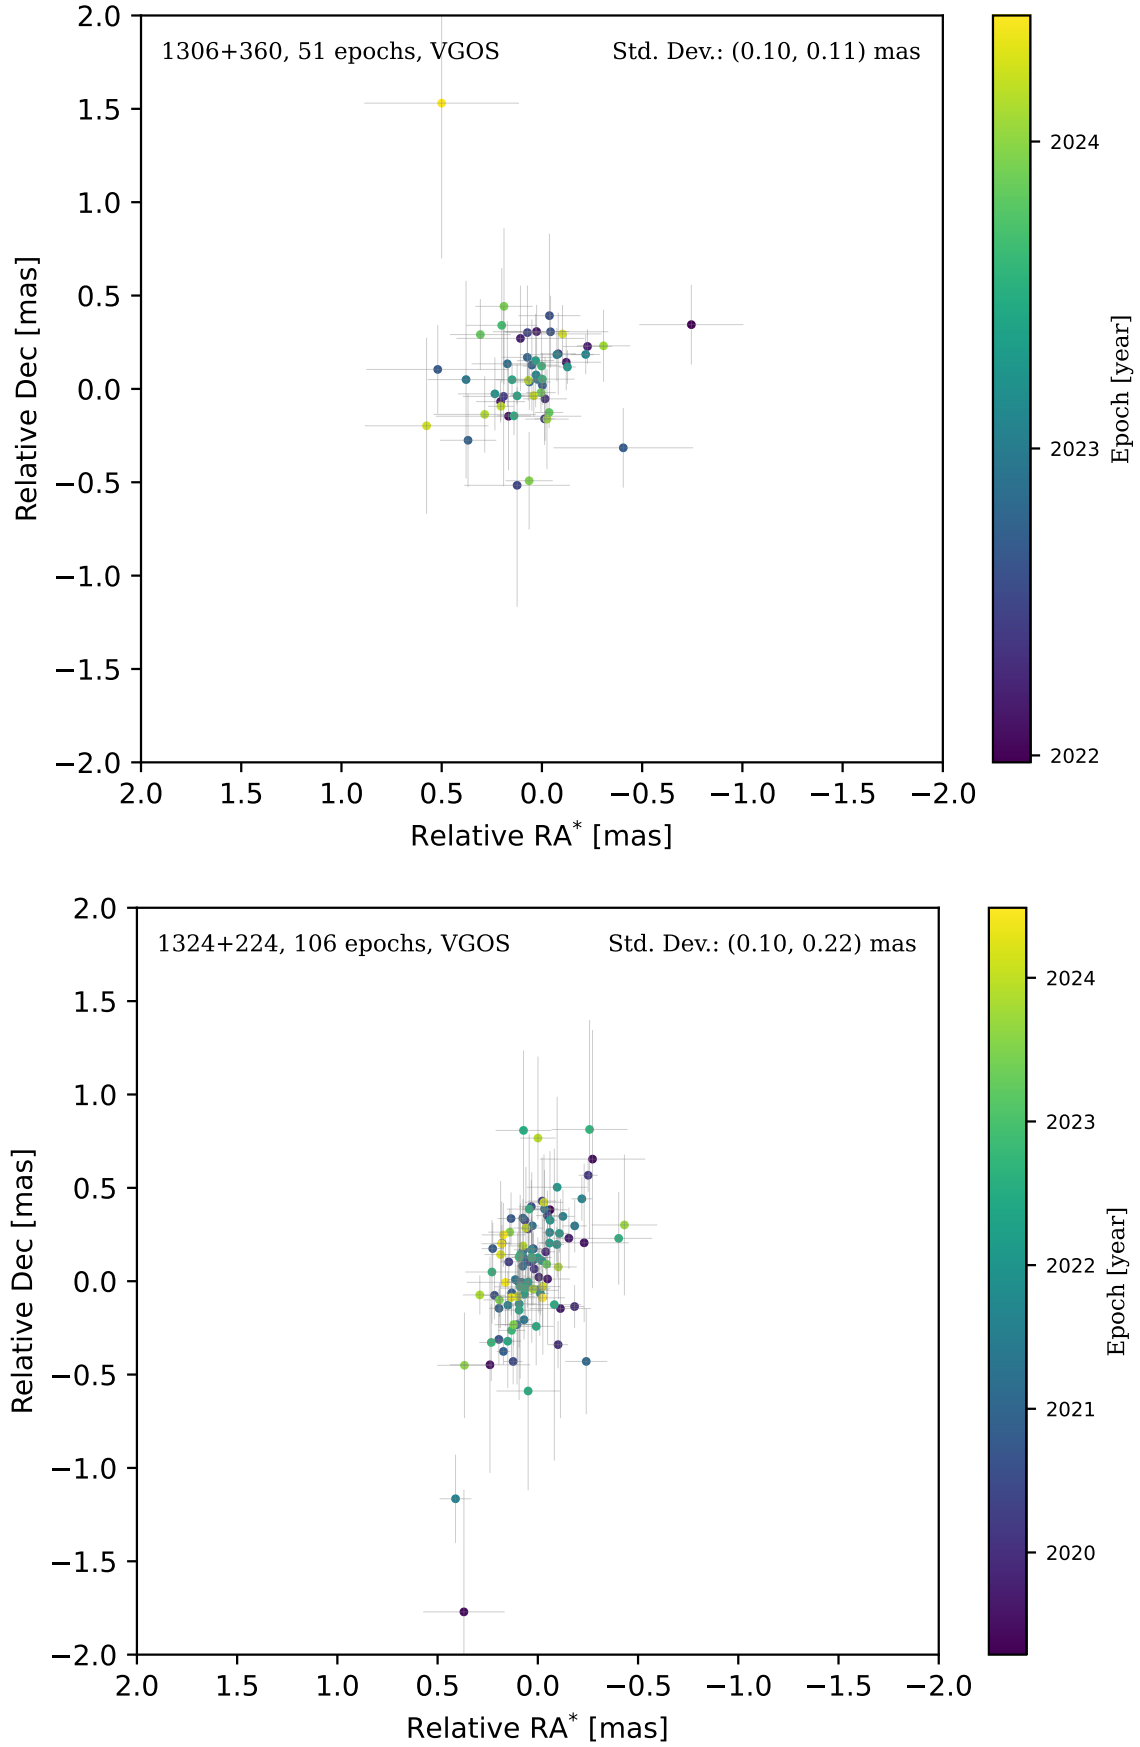

**Figure 25.** Position time series

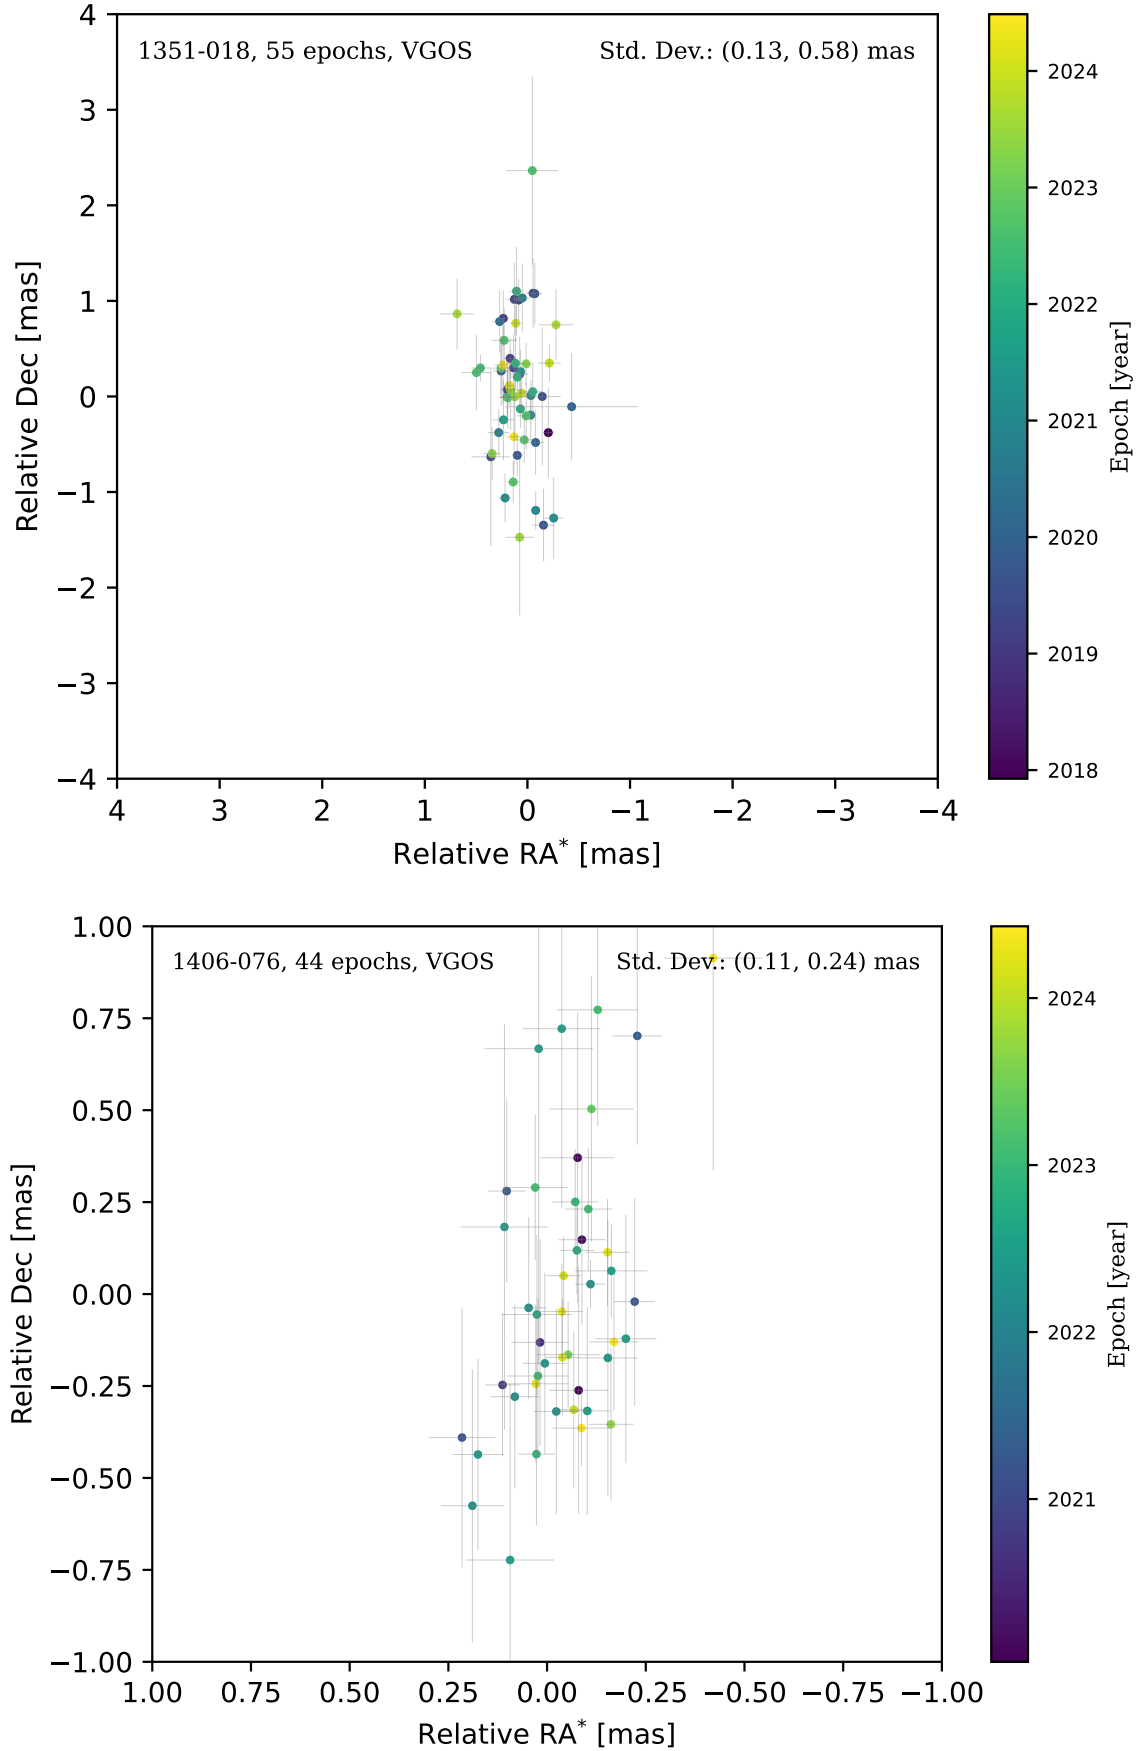**Figure 26.** Position time series

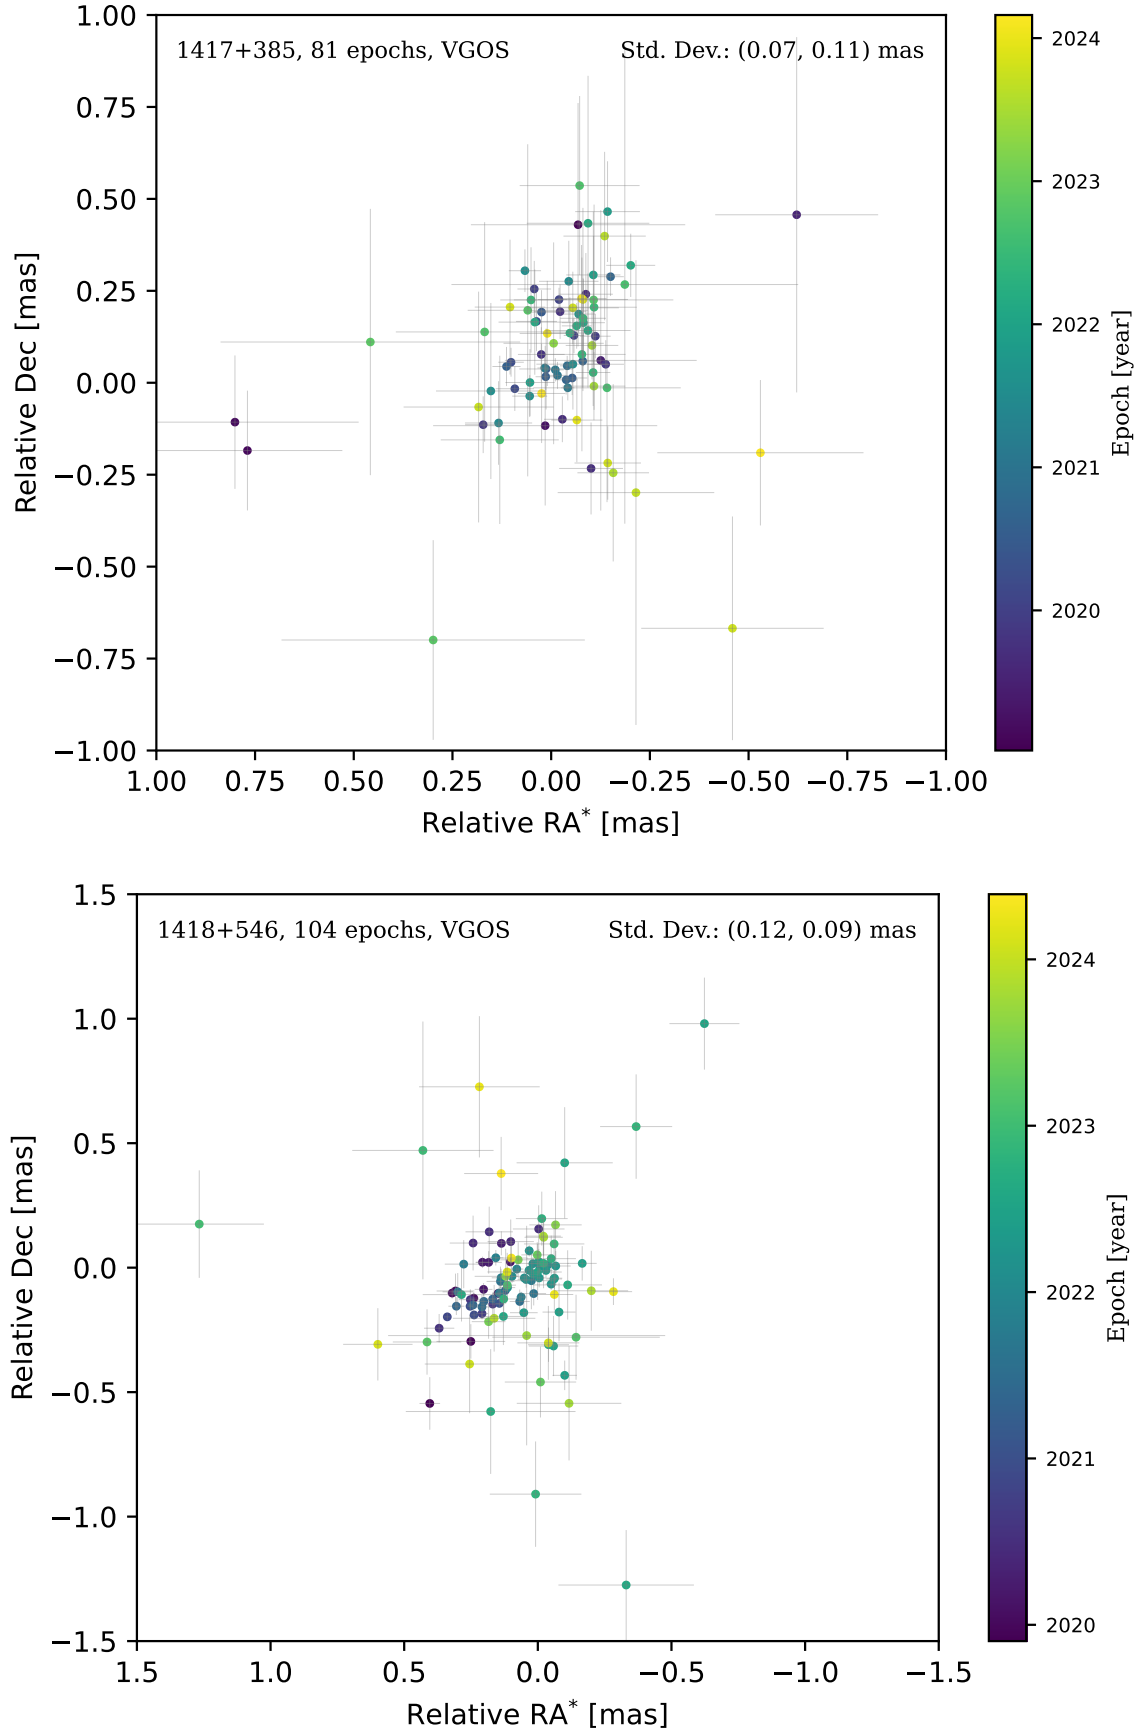

Figure 27. Position time series

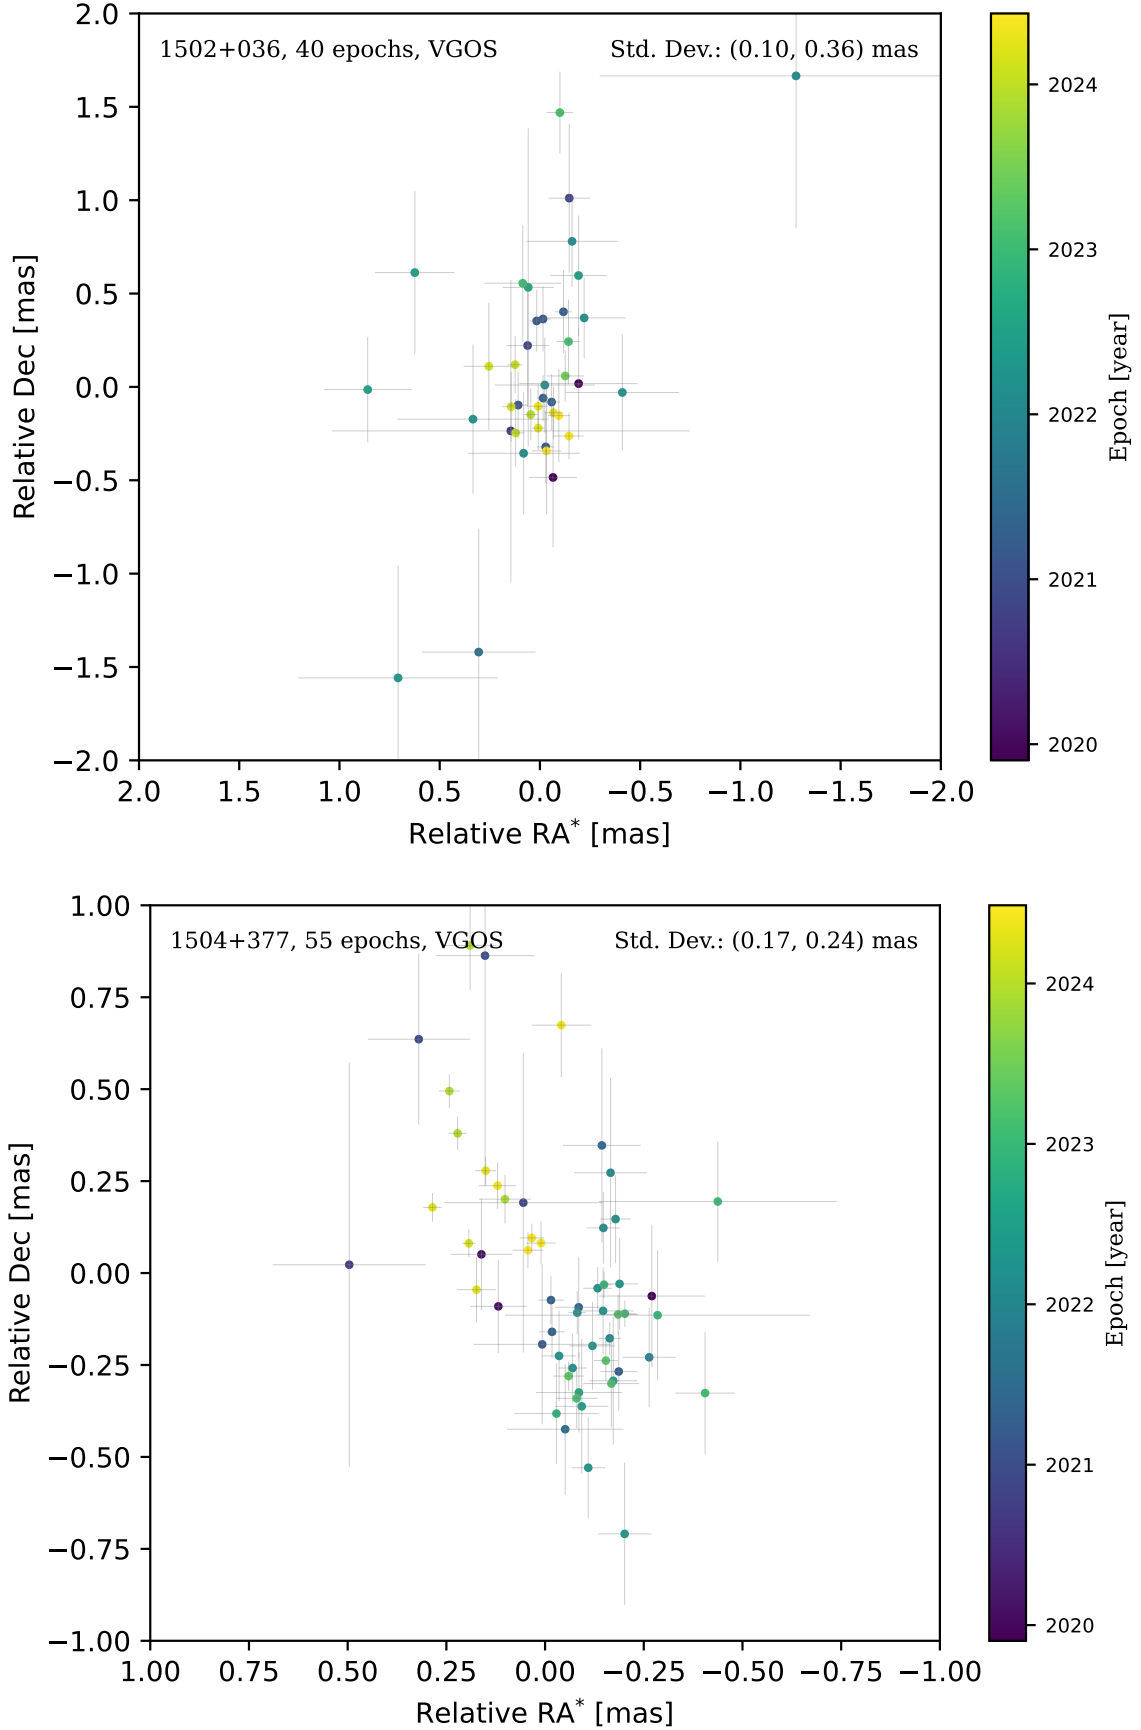**Figure 28.** Position time series

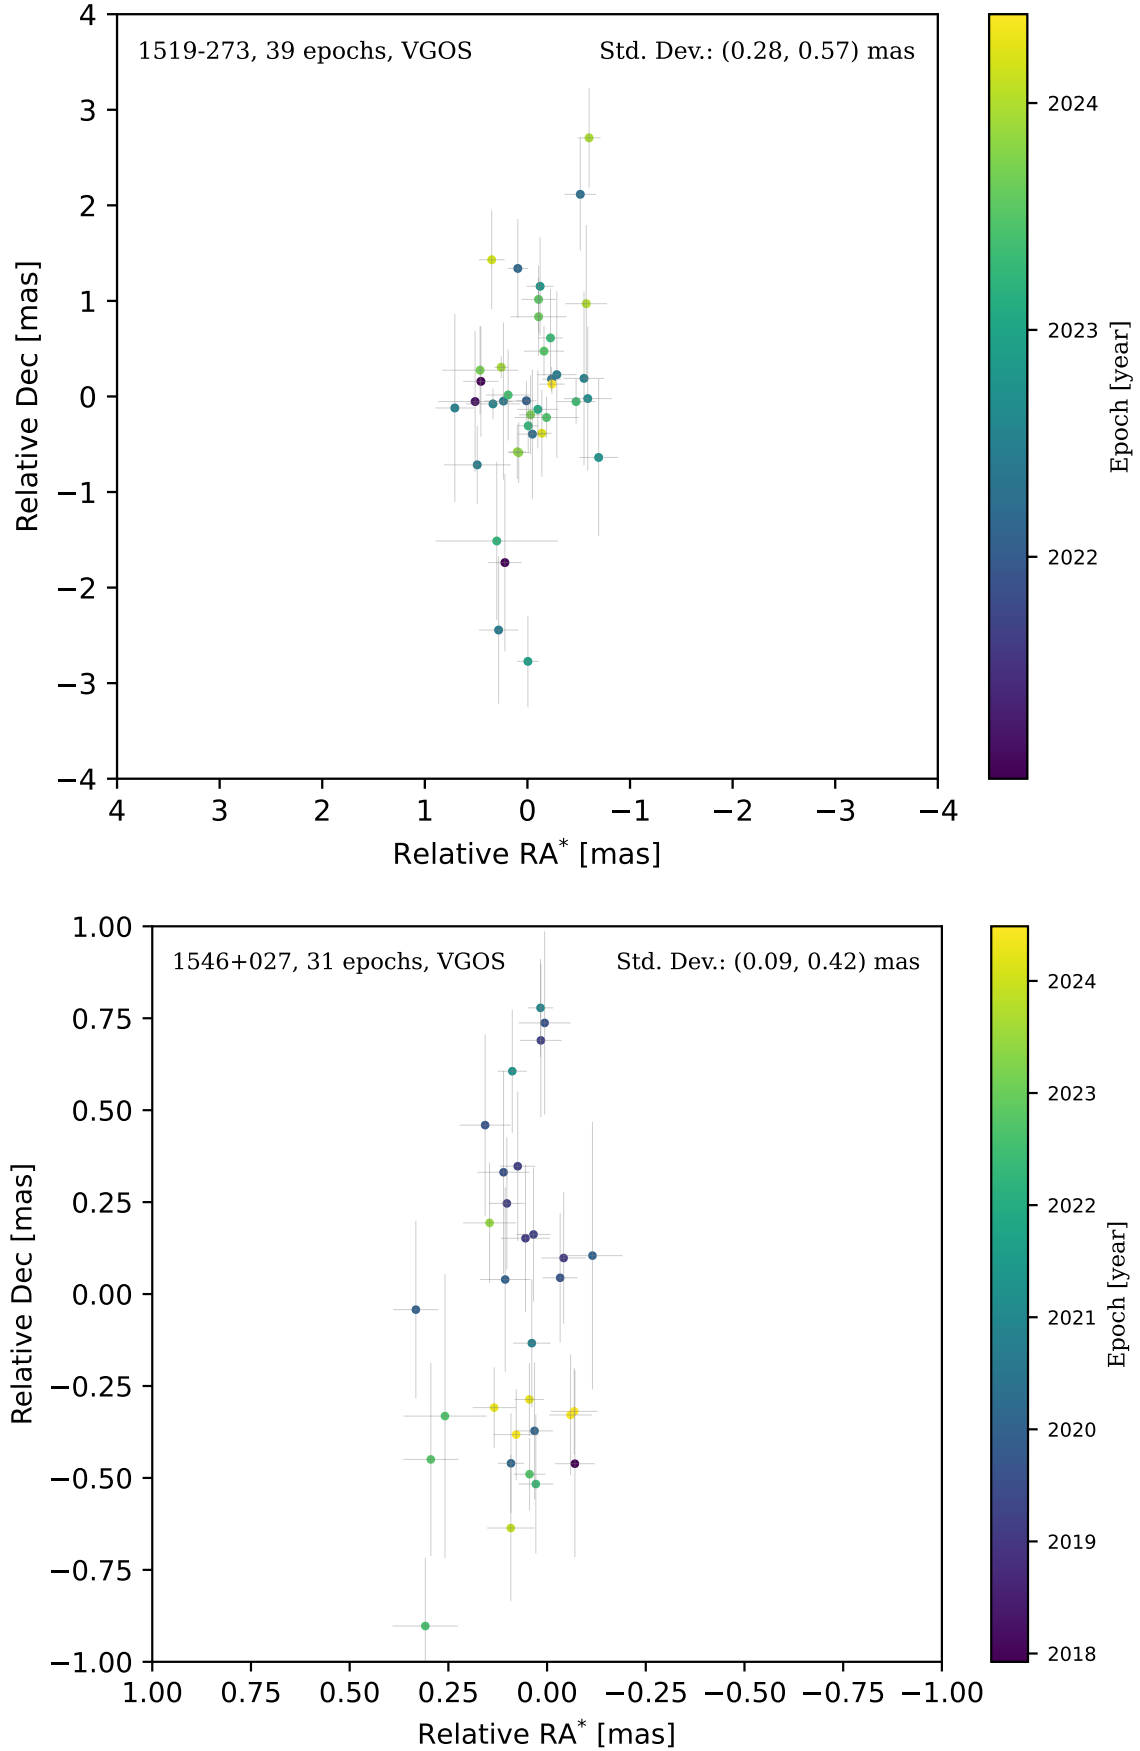

**Figure 29.** Position time series

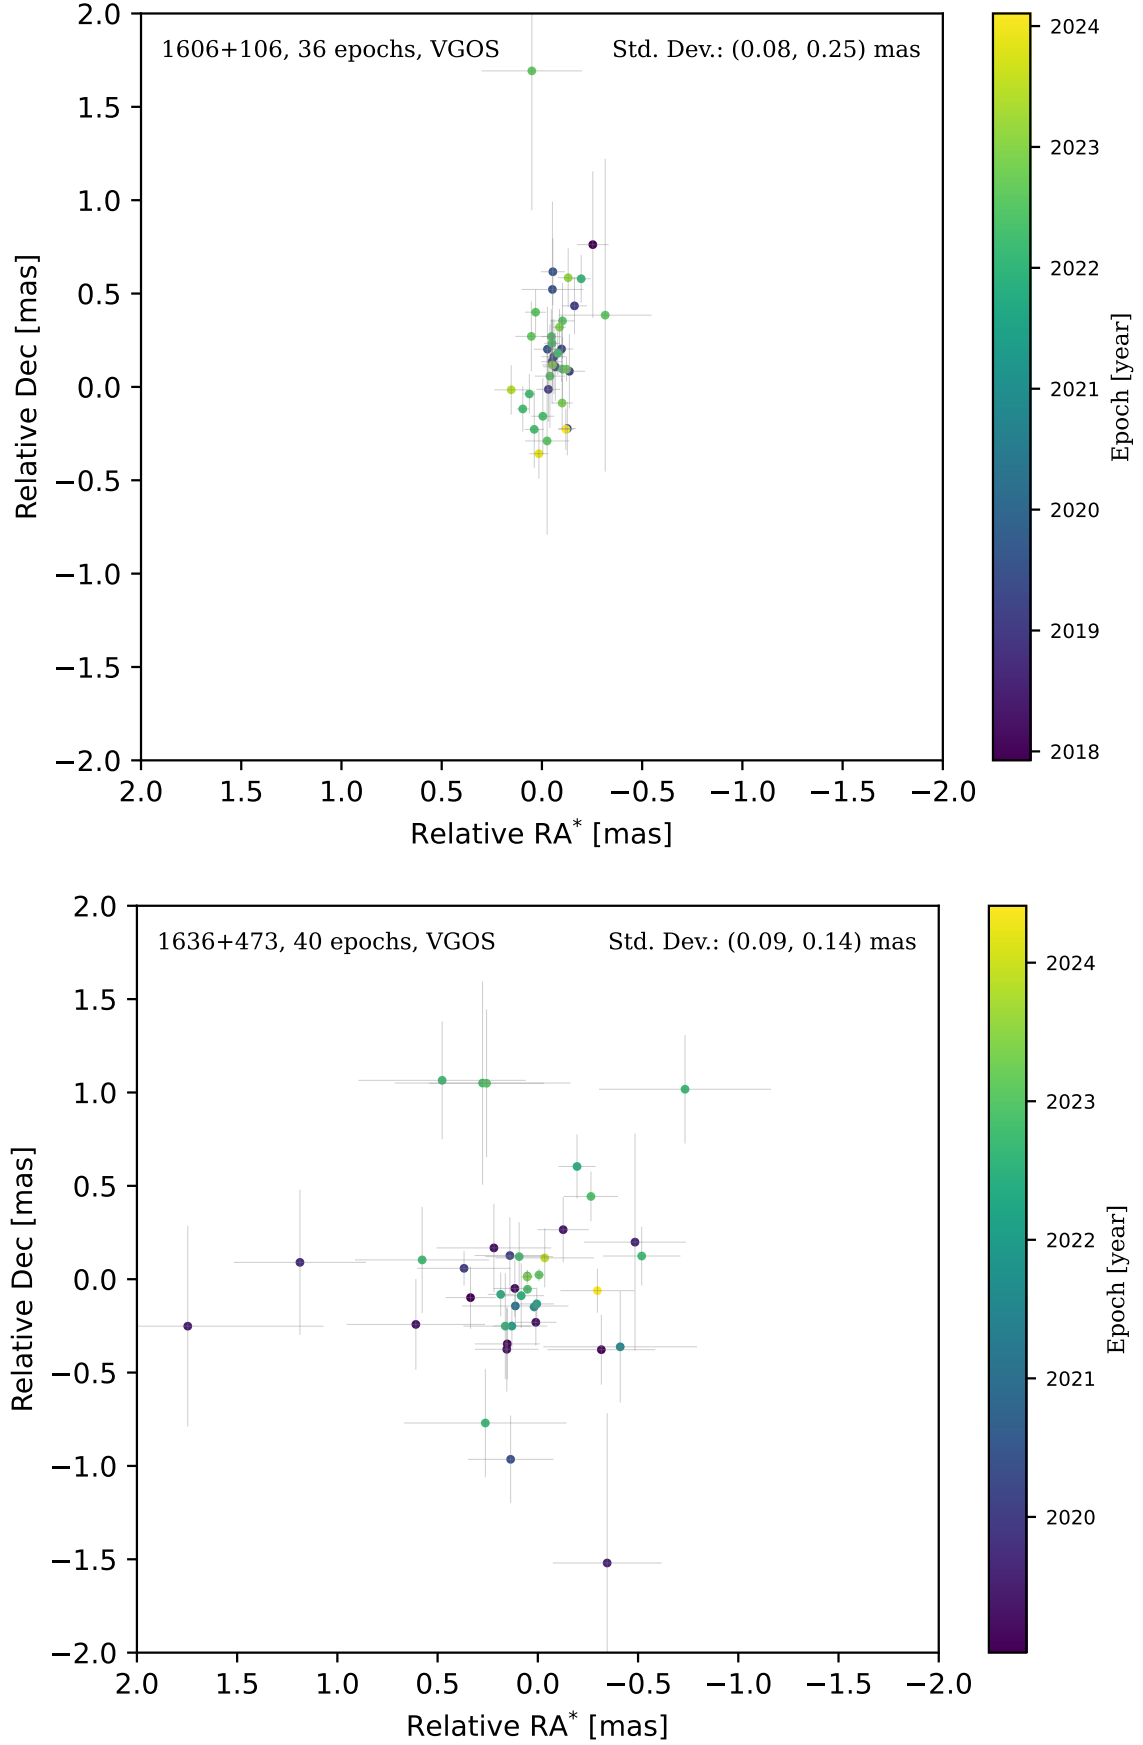

Figure 30. Position time series

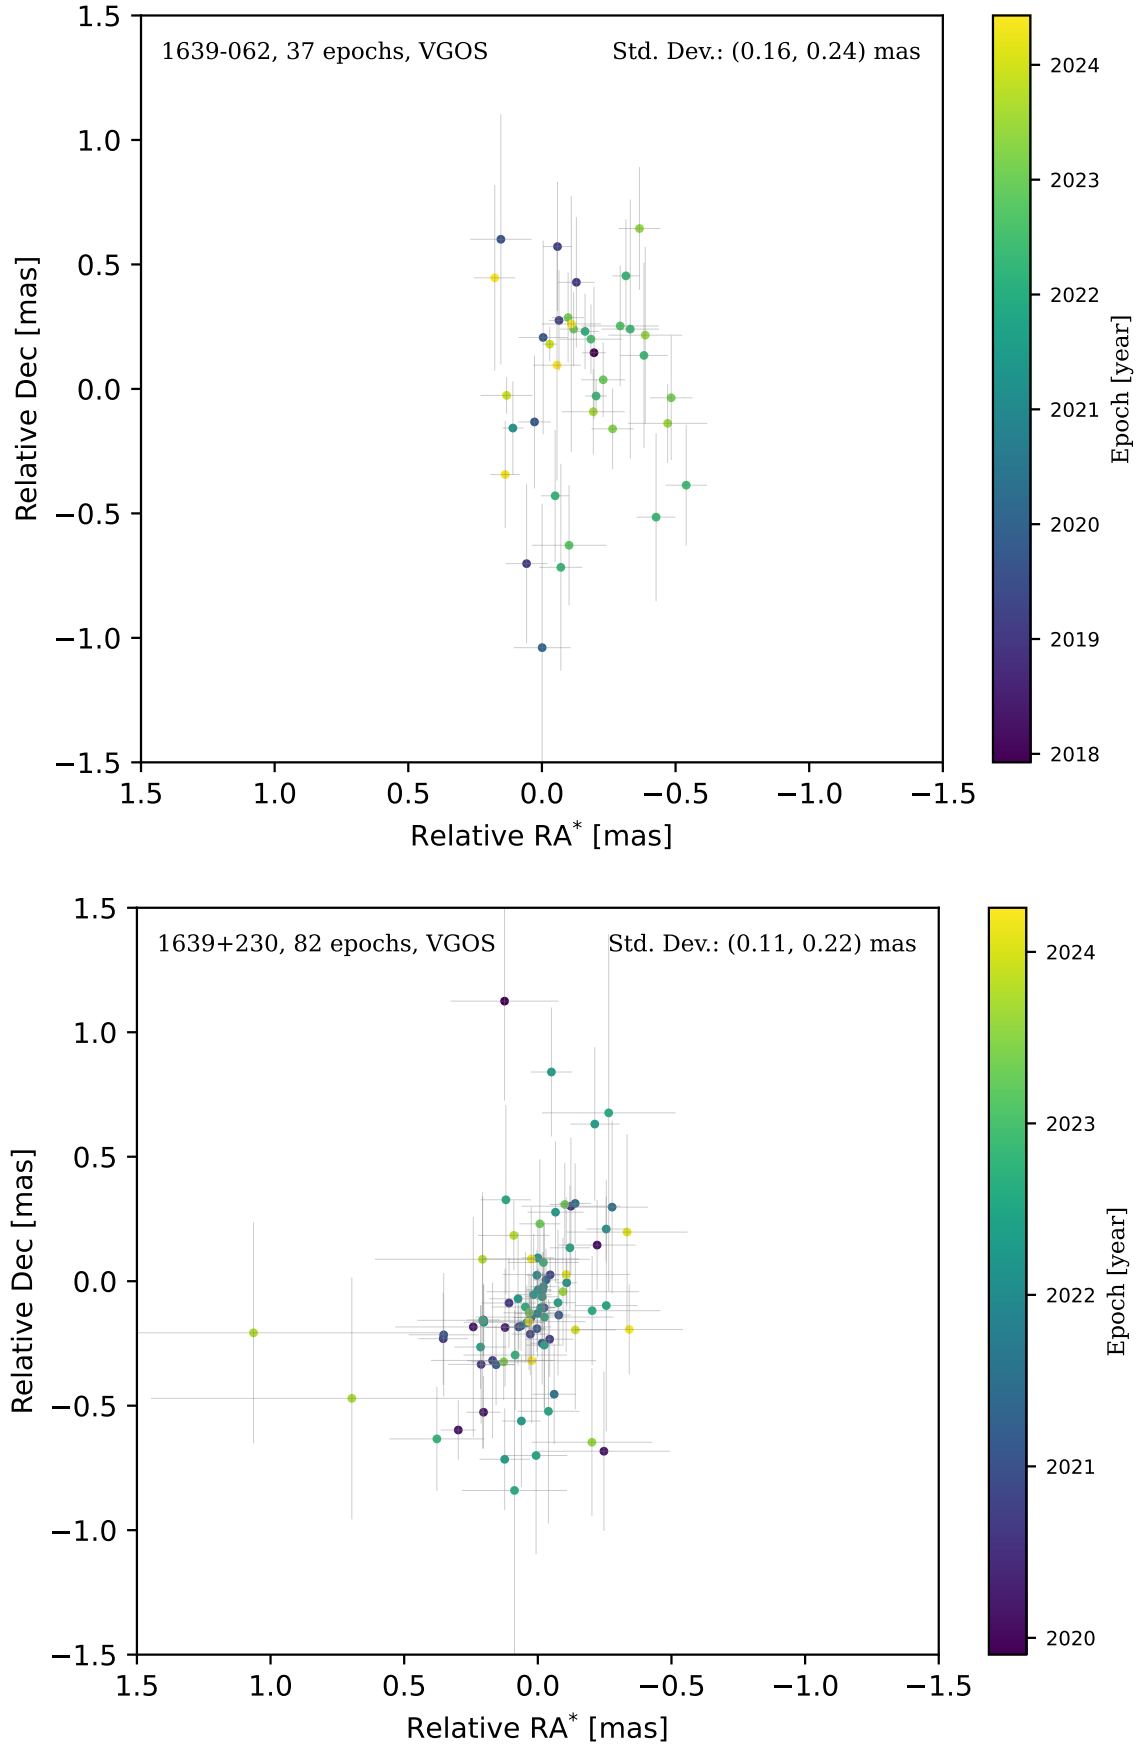

**Figure 31.** Position time series



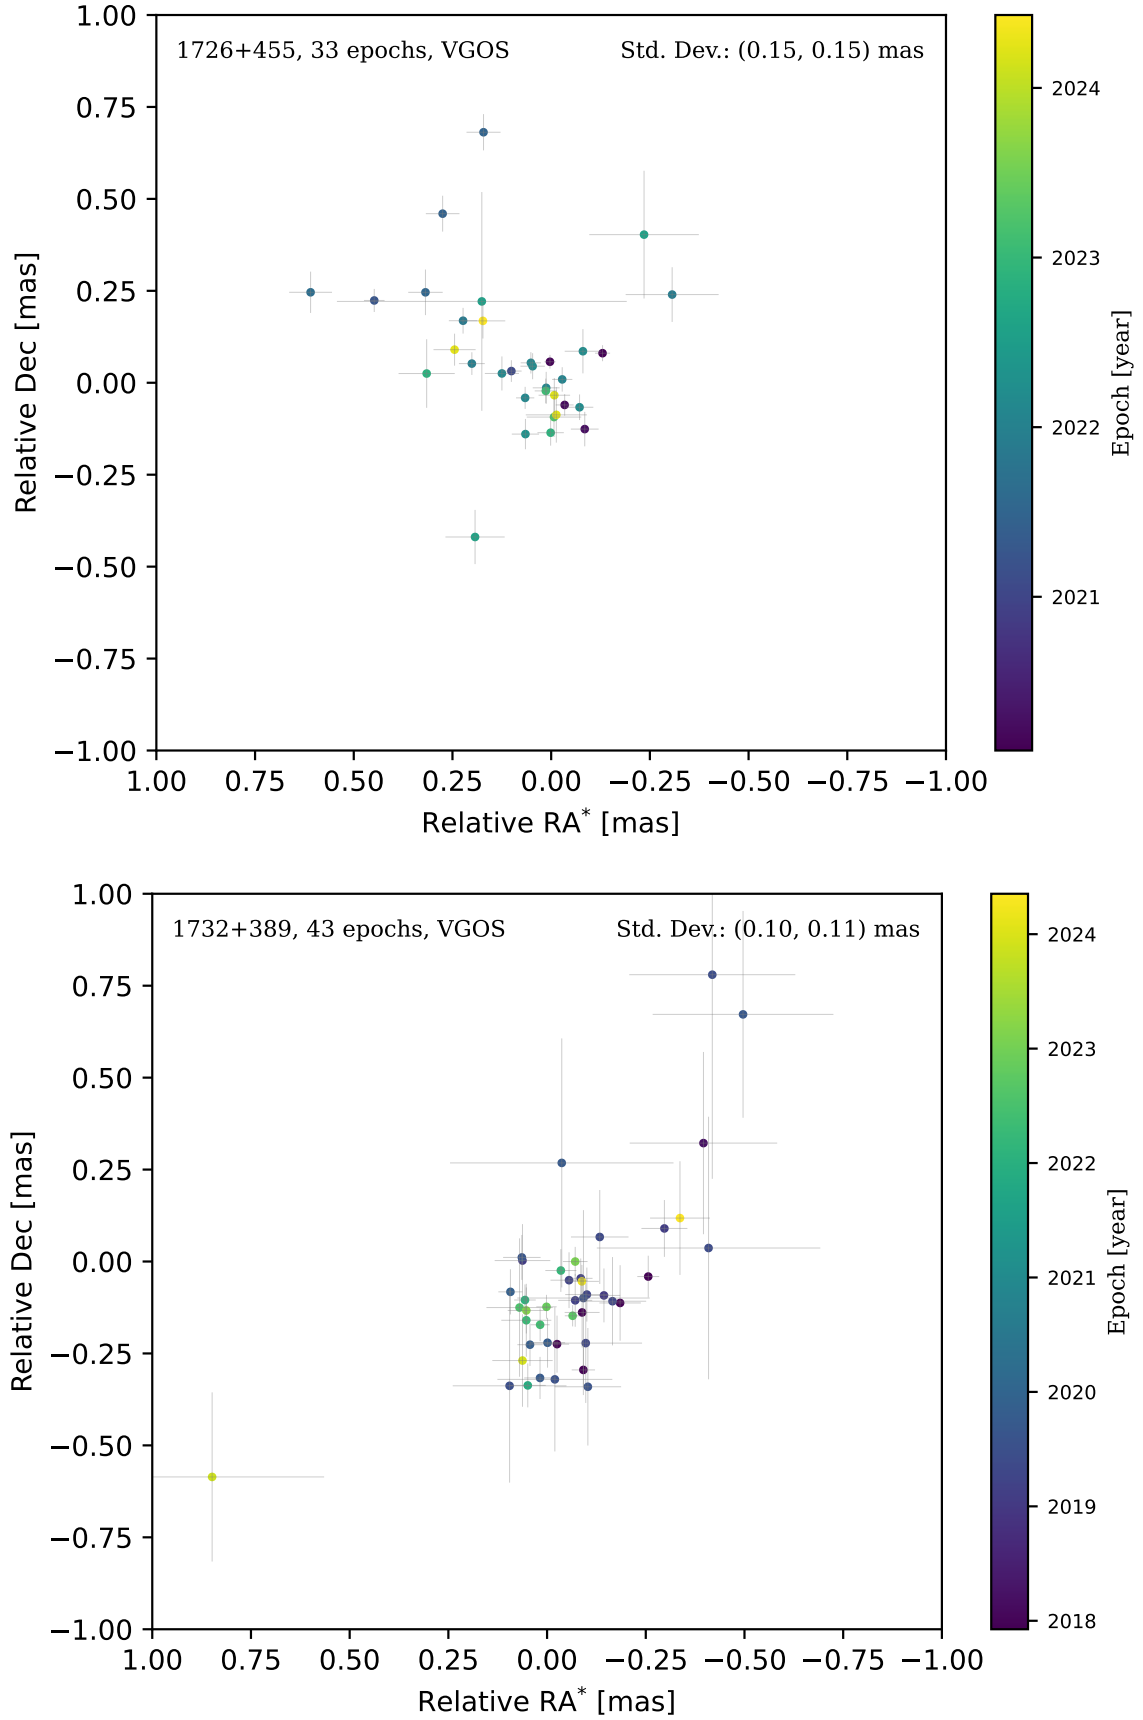

Figure 32. Position time series

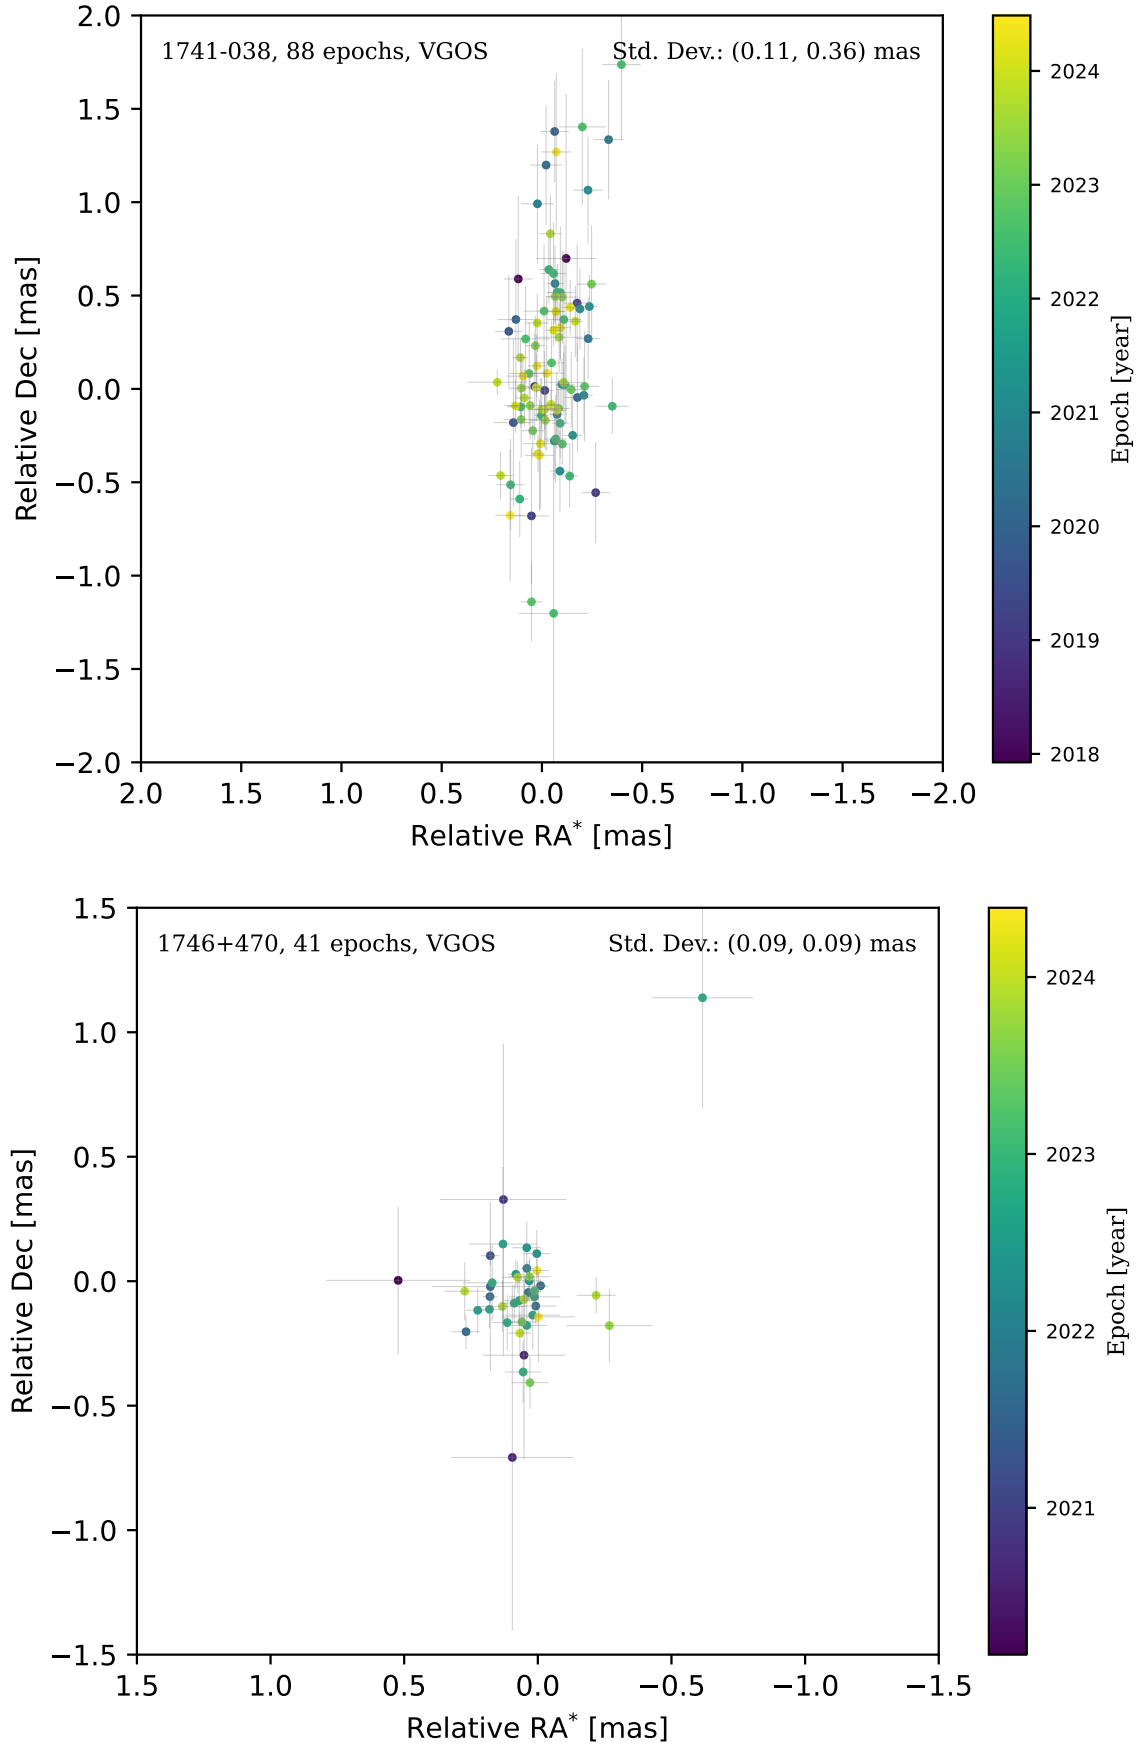

**Figure 33.** Position time series

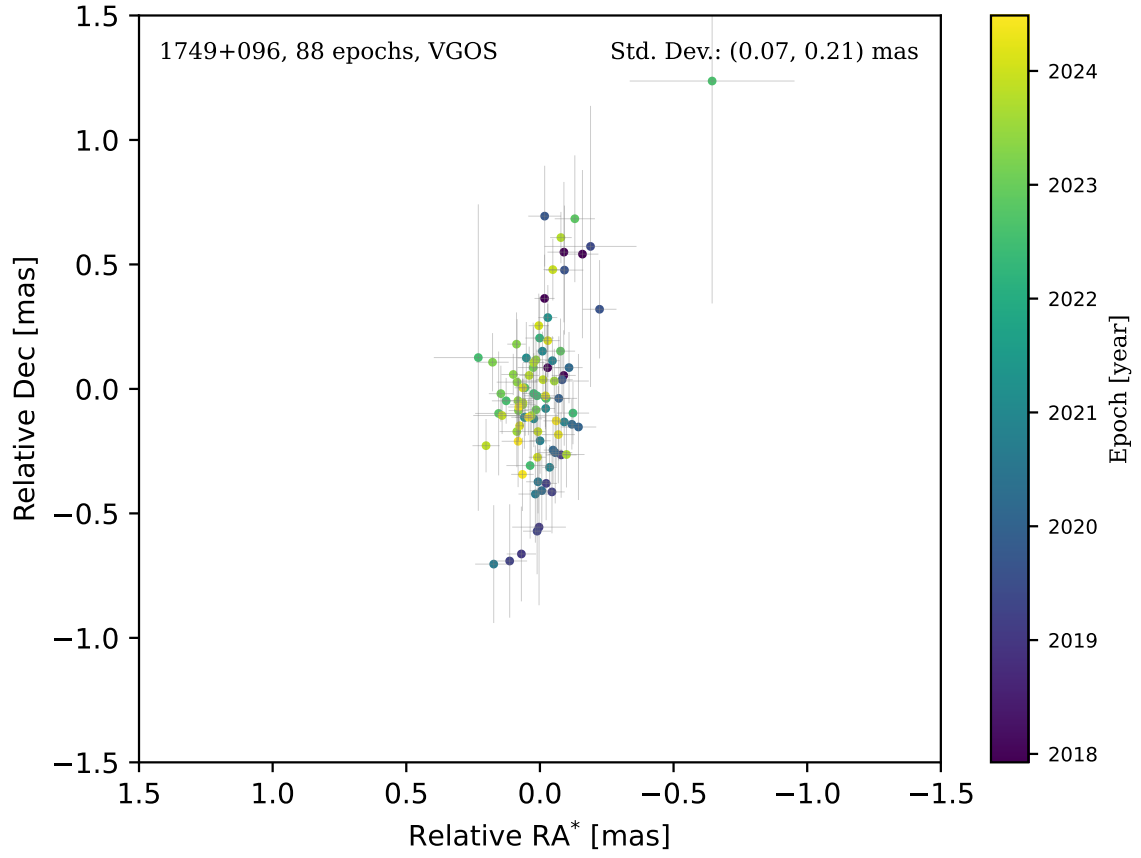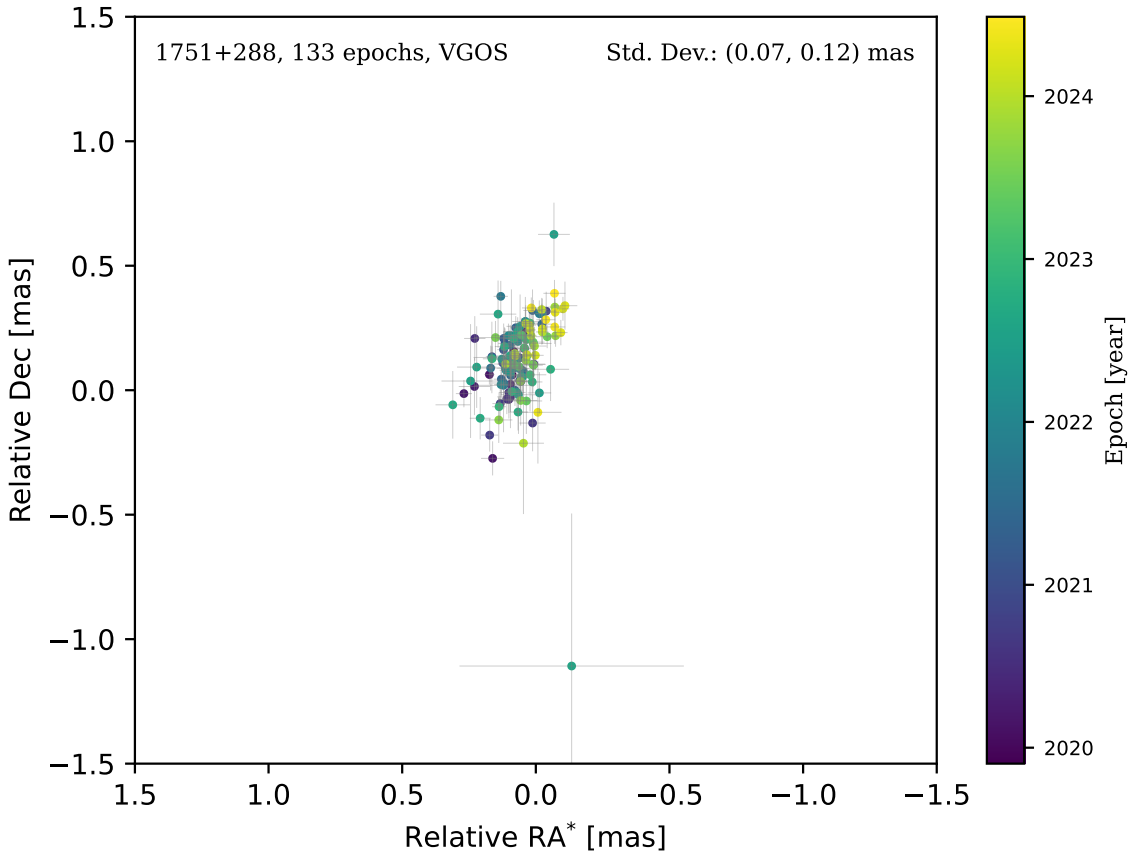

Figure 34. Position time series

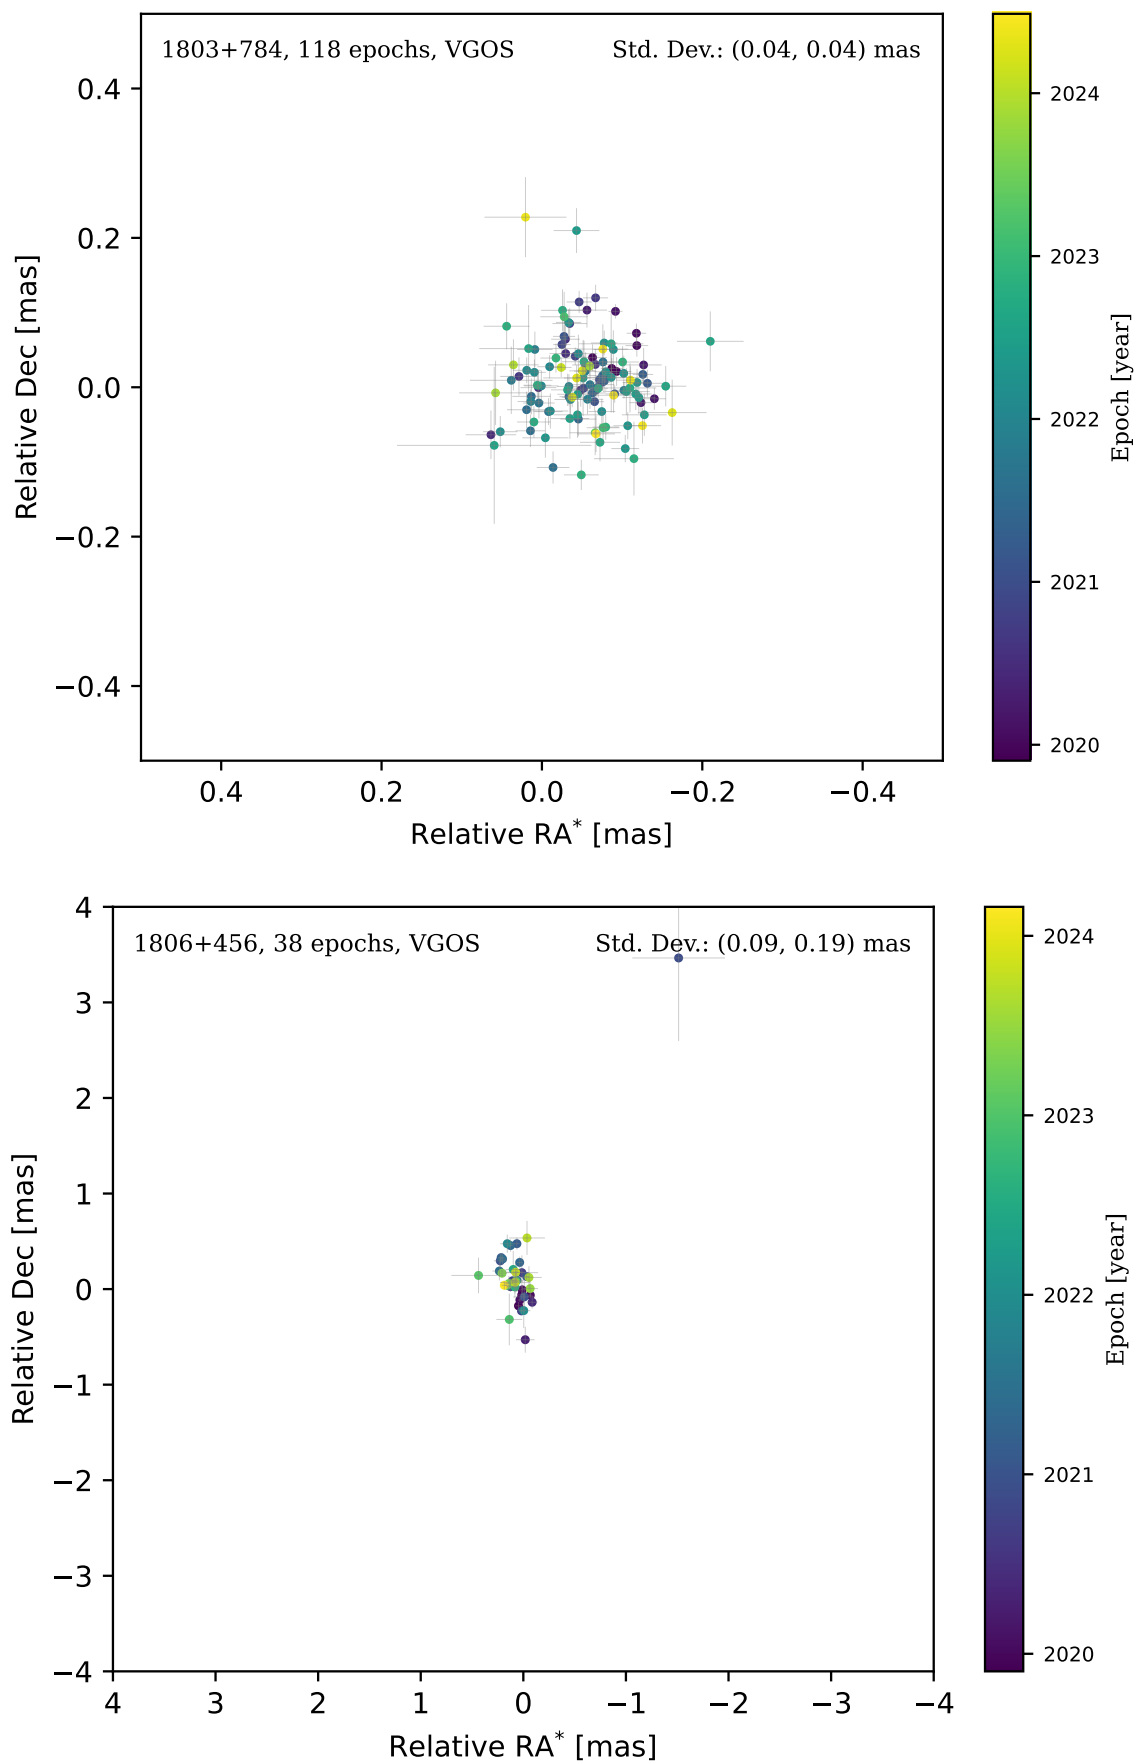

**Figure 35.** Position time series

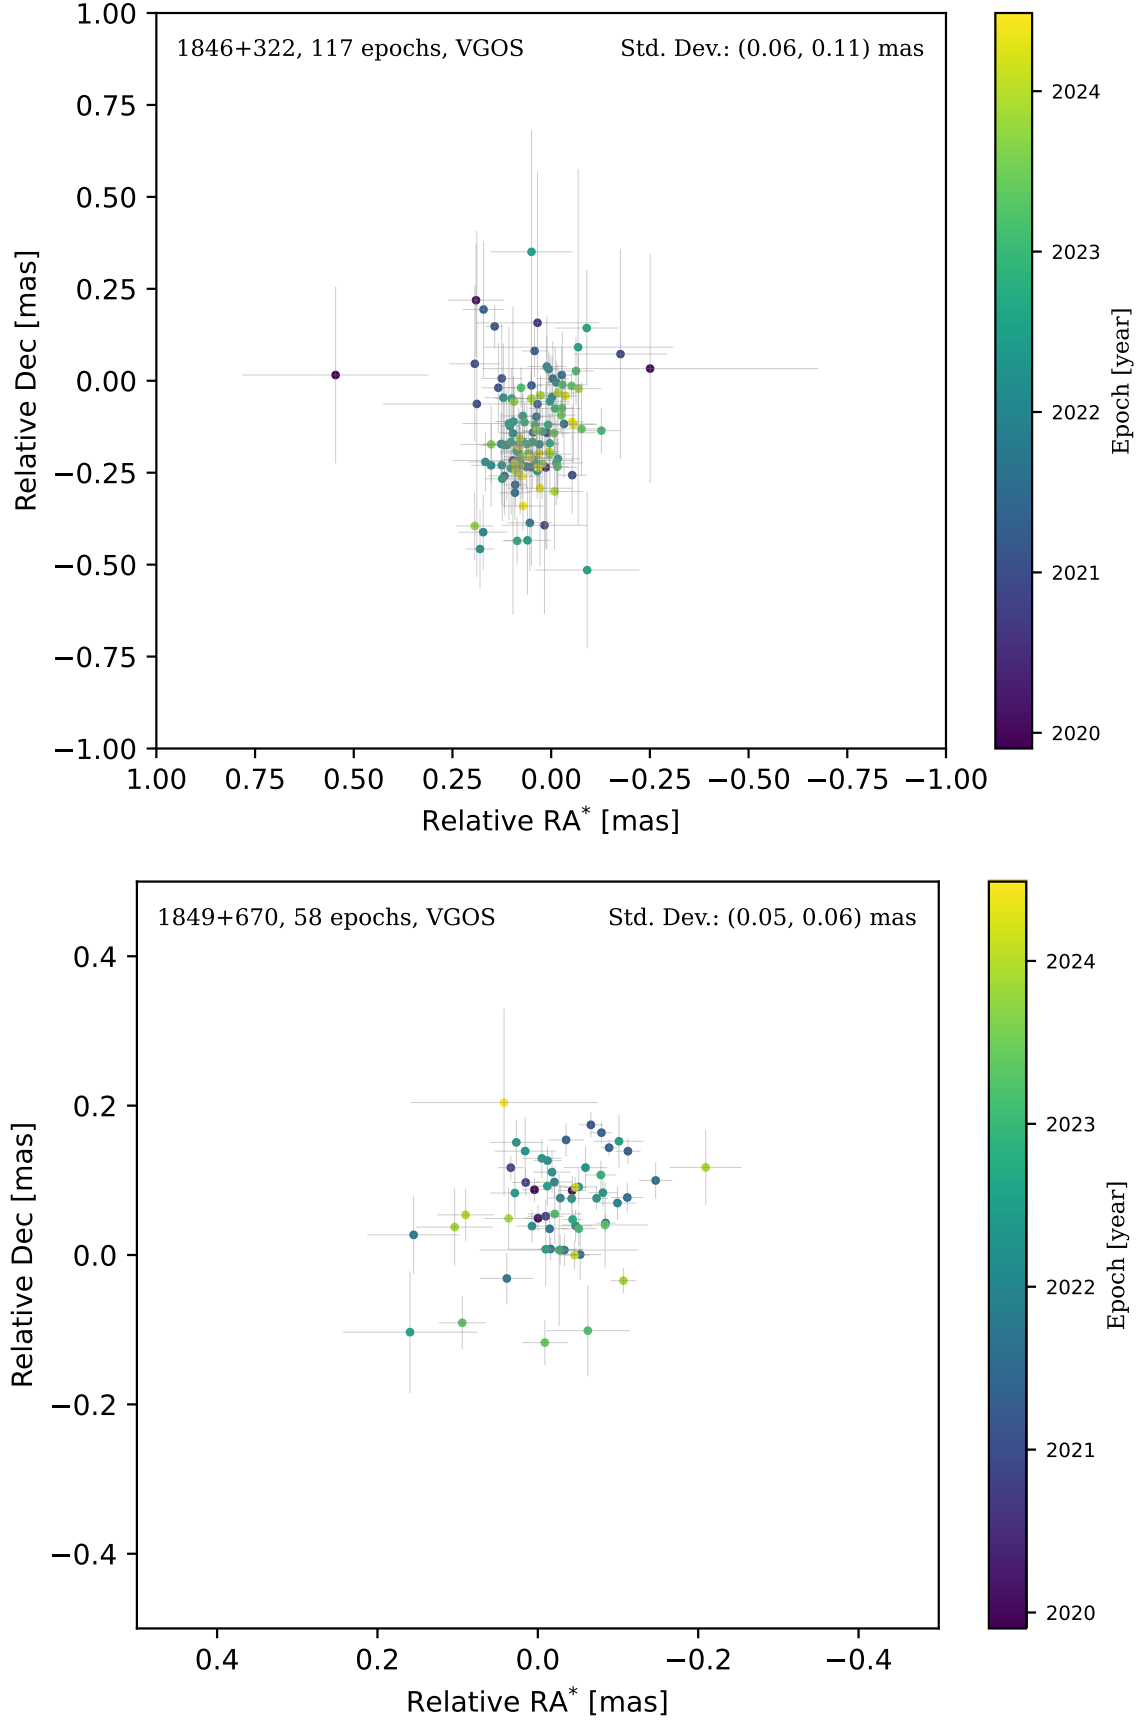**Figure 36.** Position time series

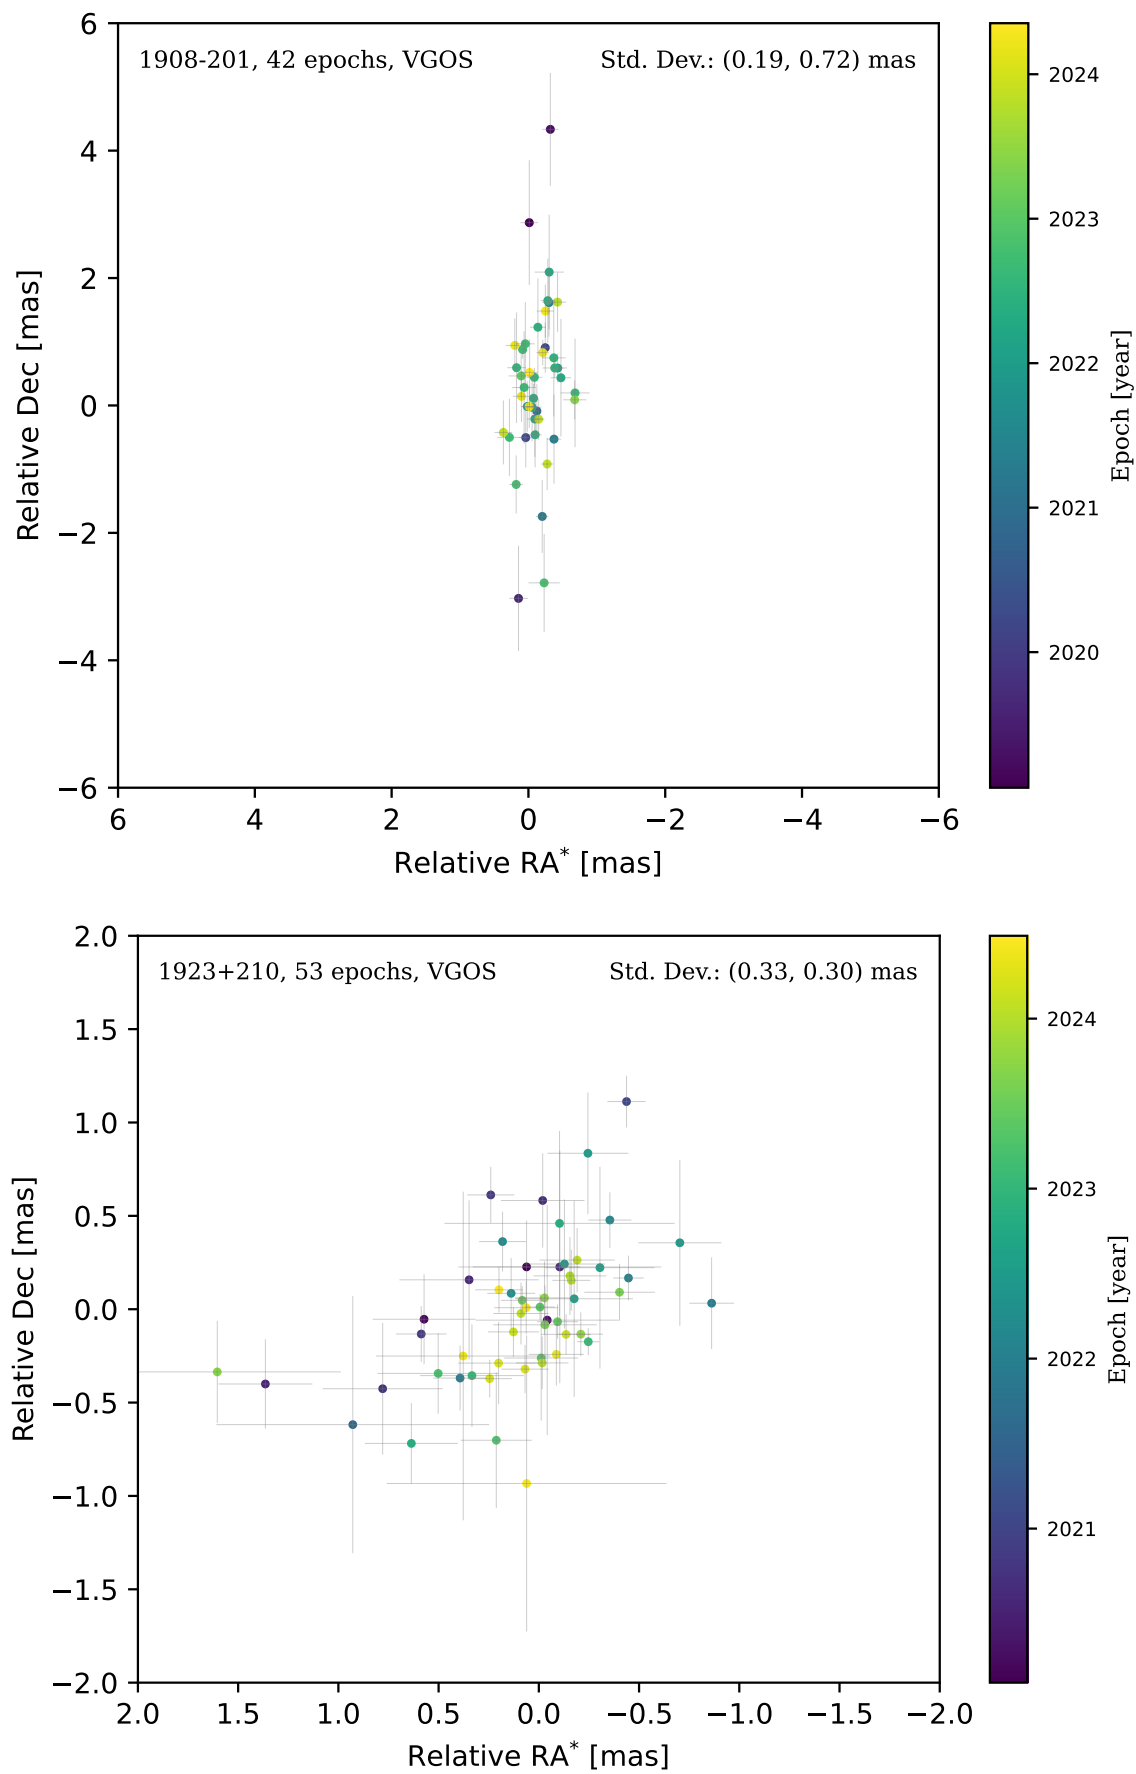

Figure 37. Position time series

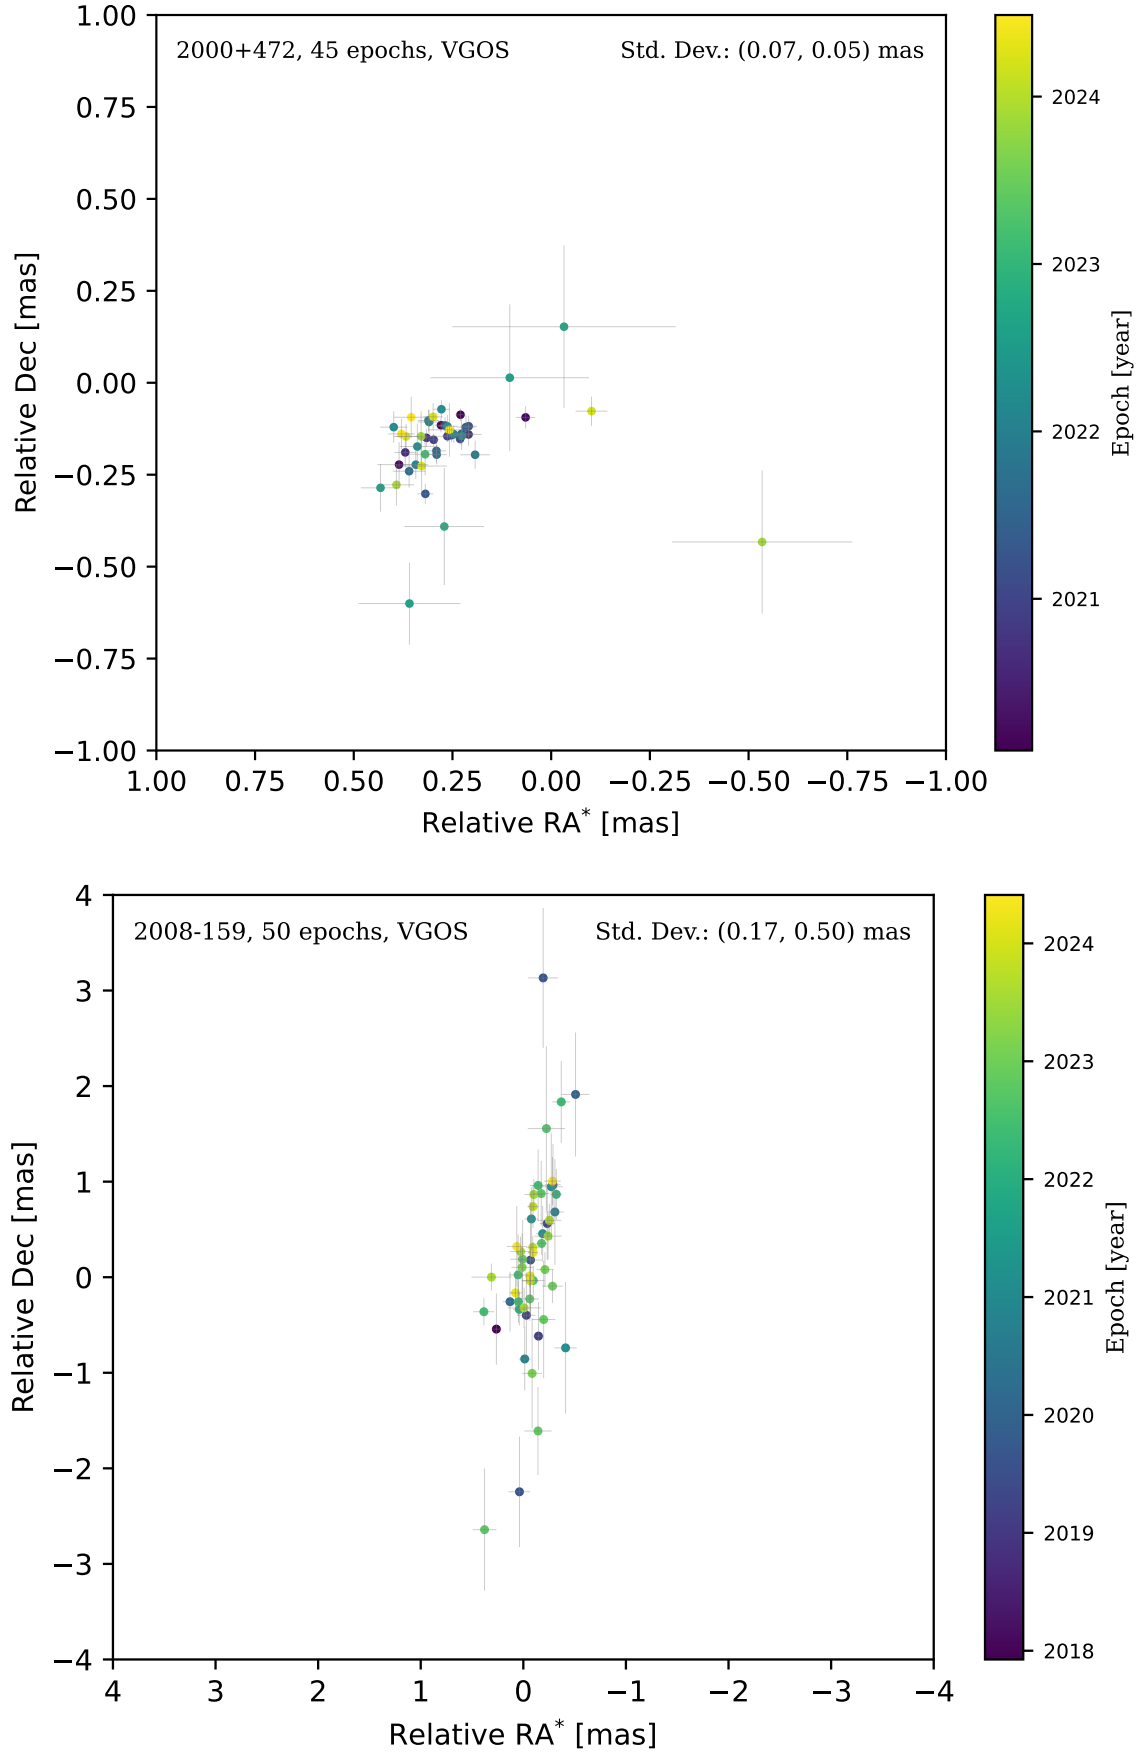**Figure 38.** Position time series

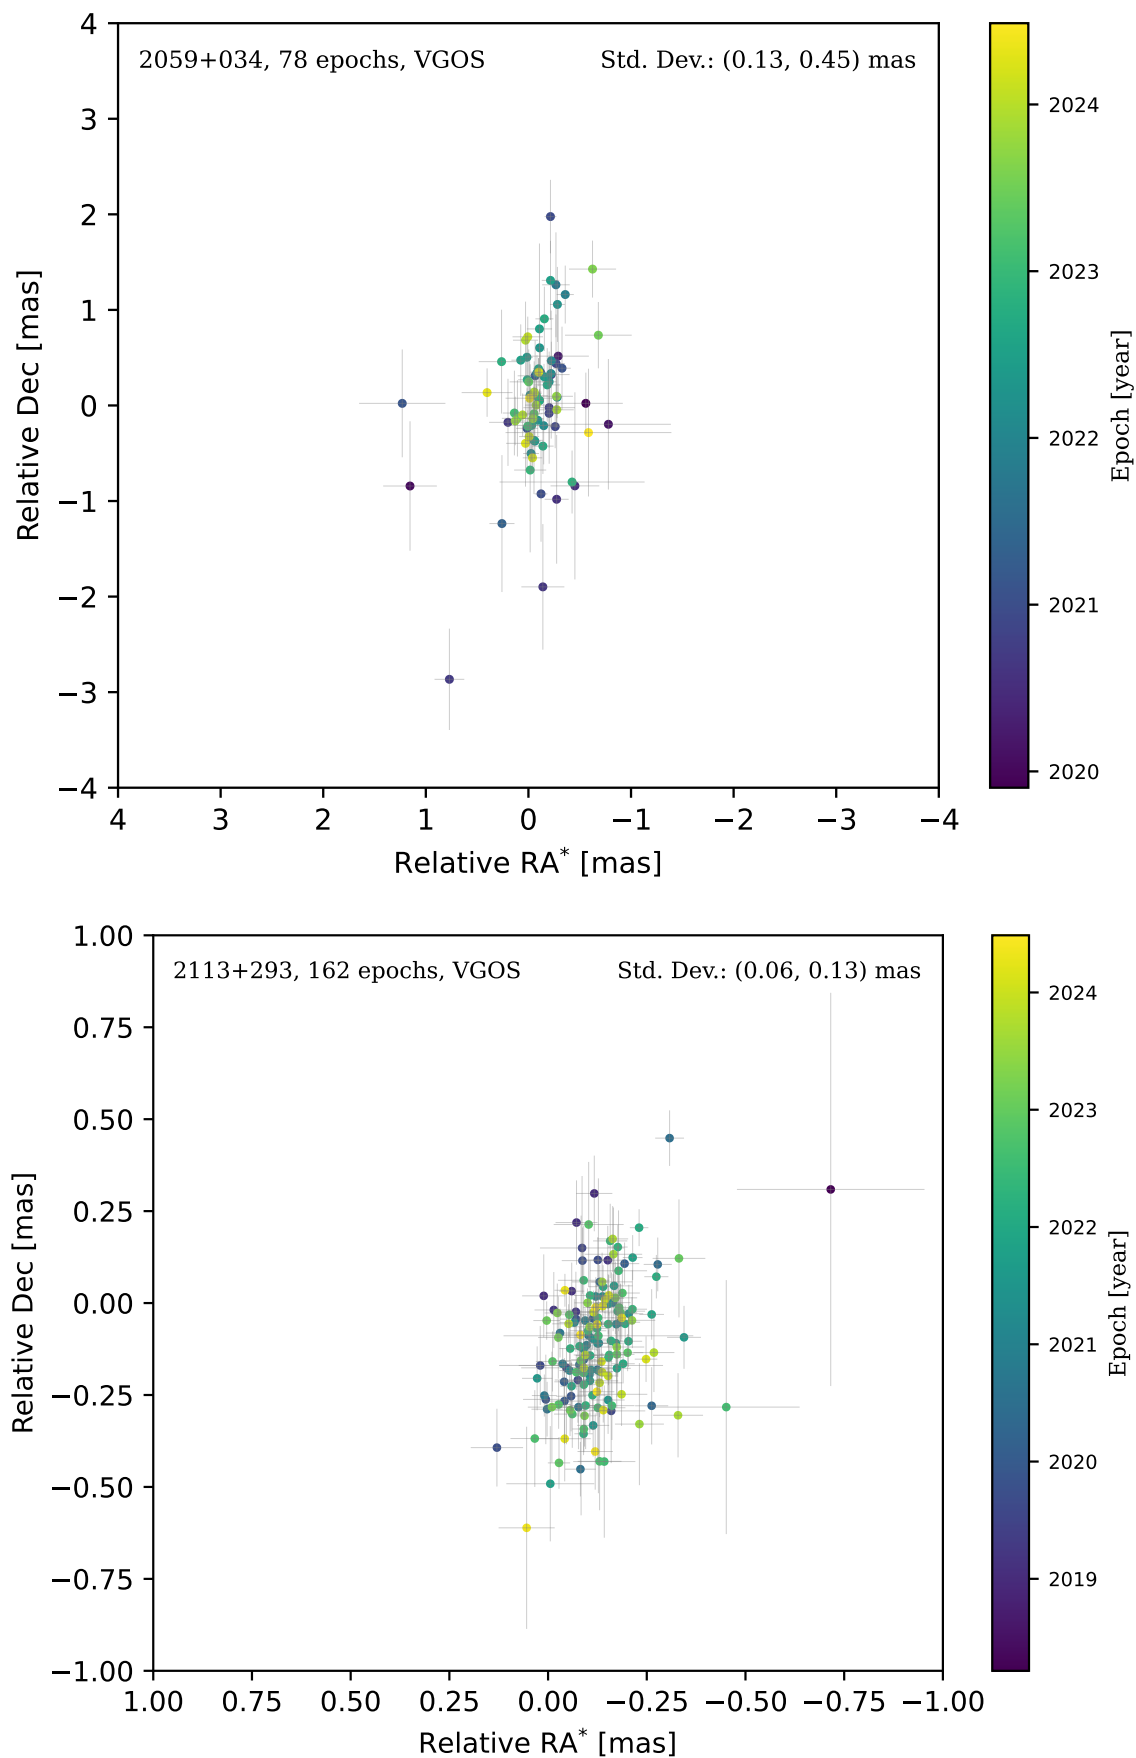

**Figure 39.** Position time series



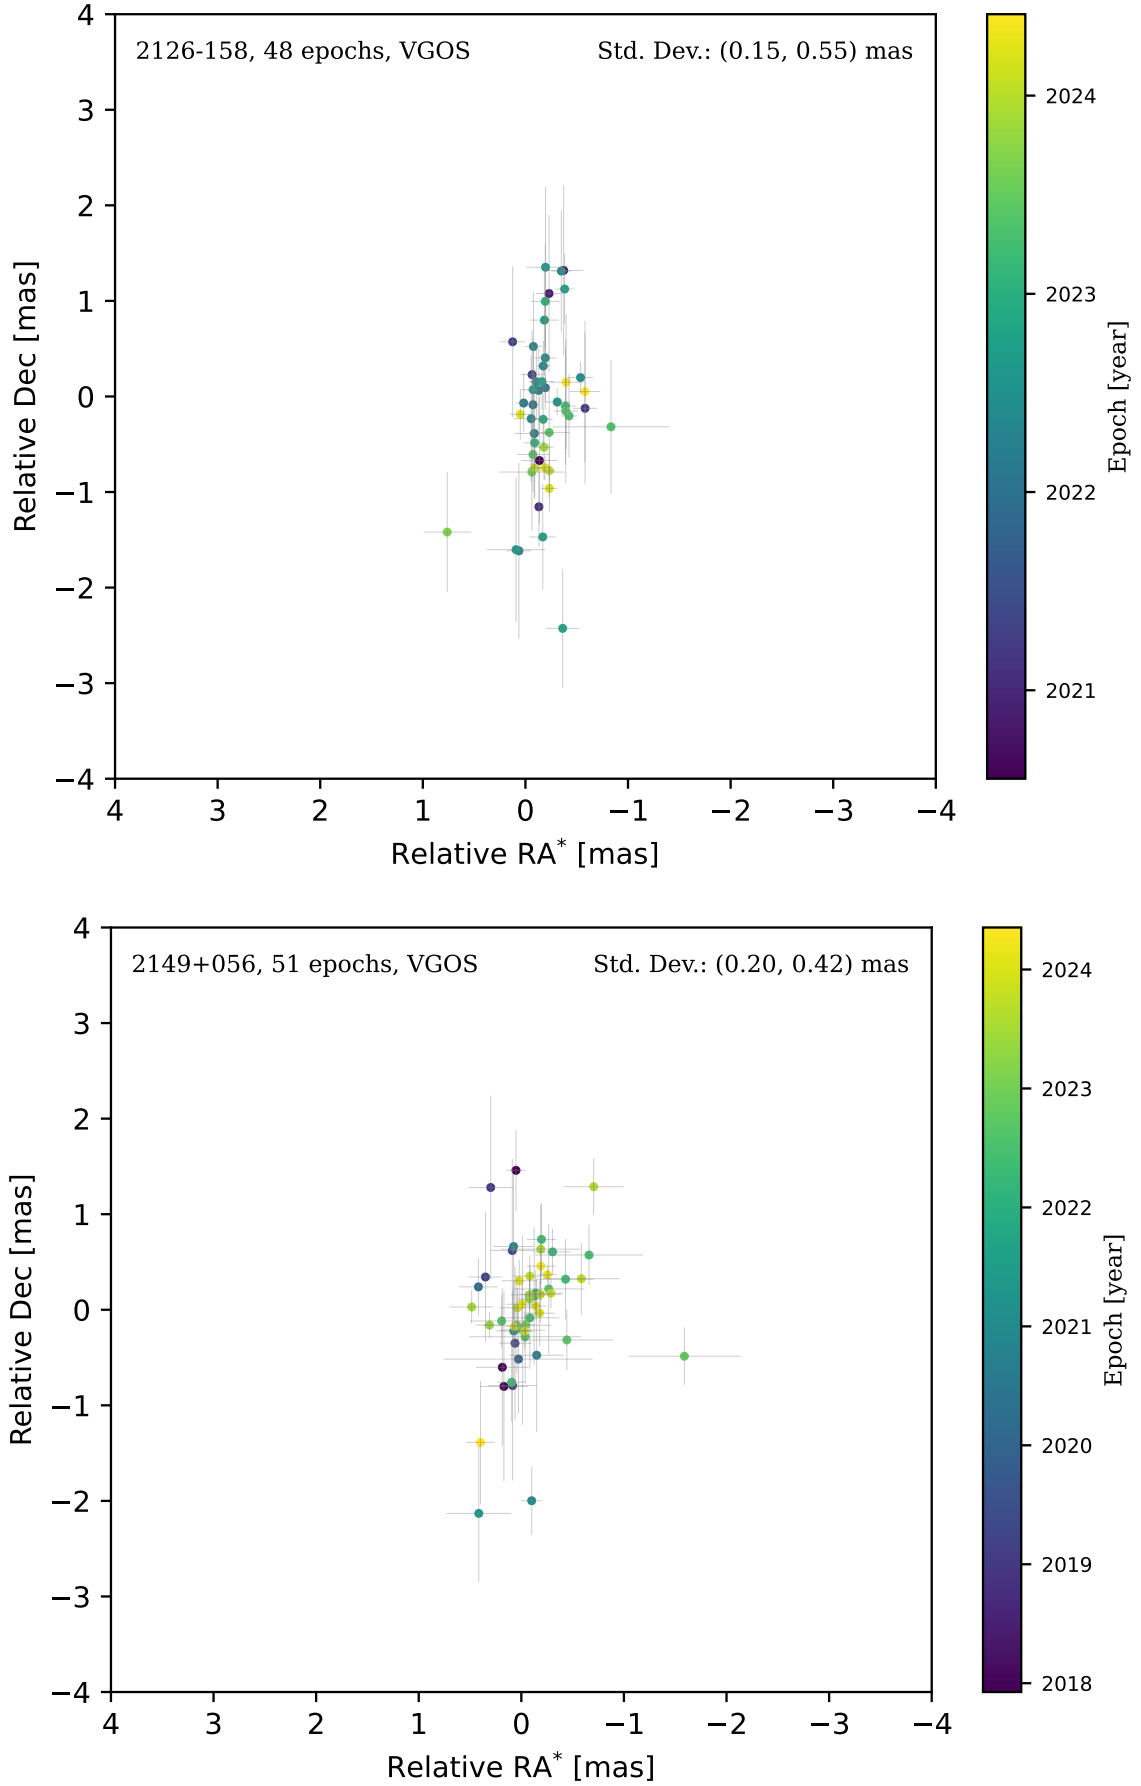**Figure 40.** Position time series

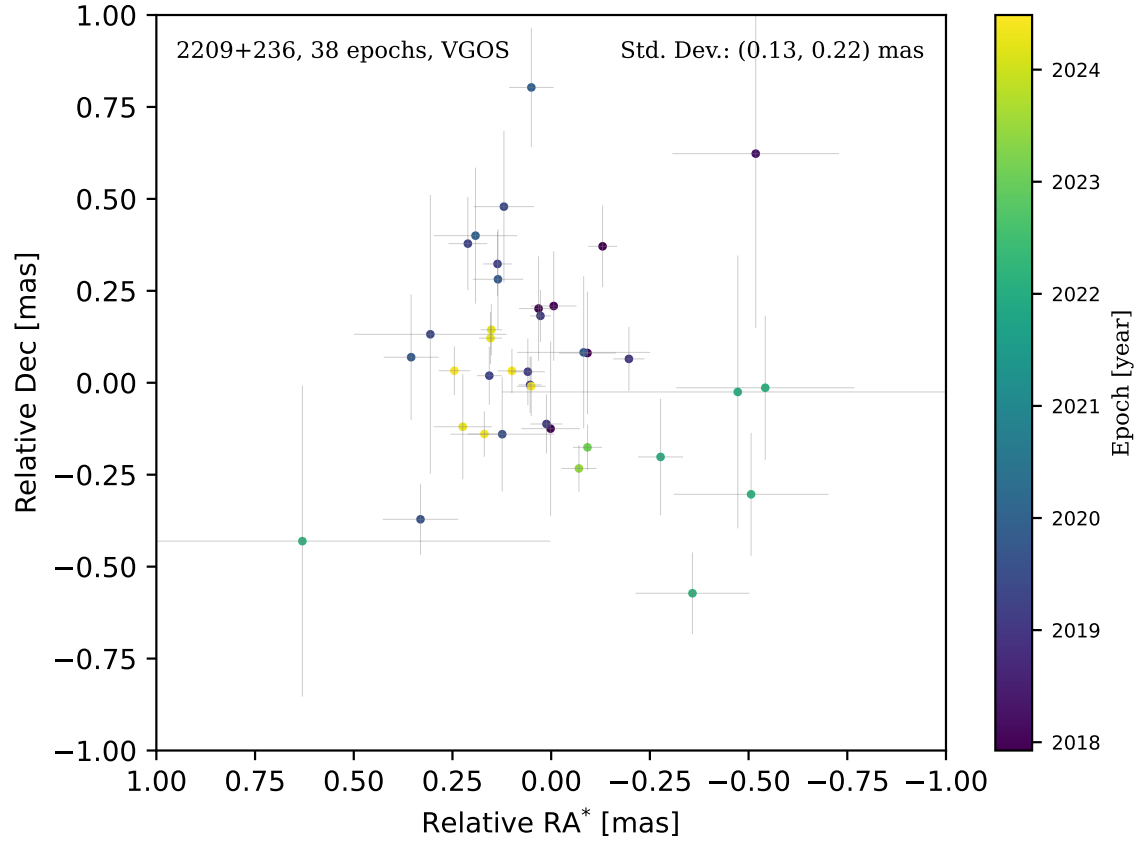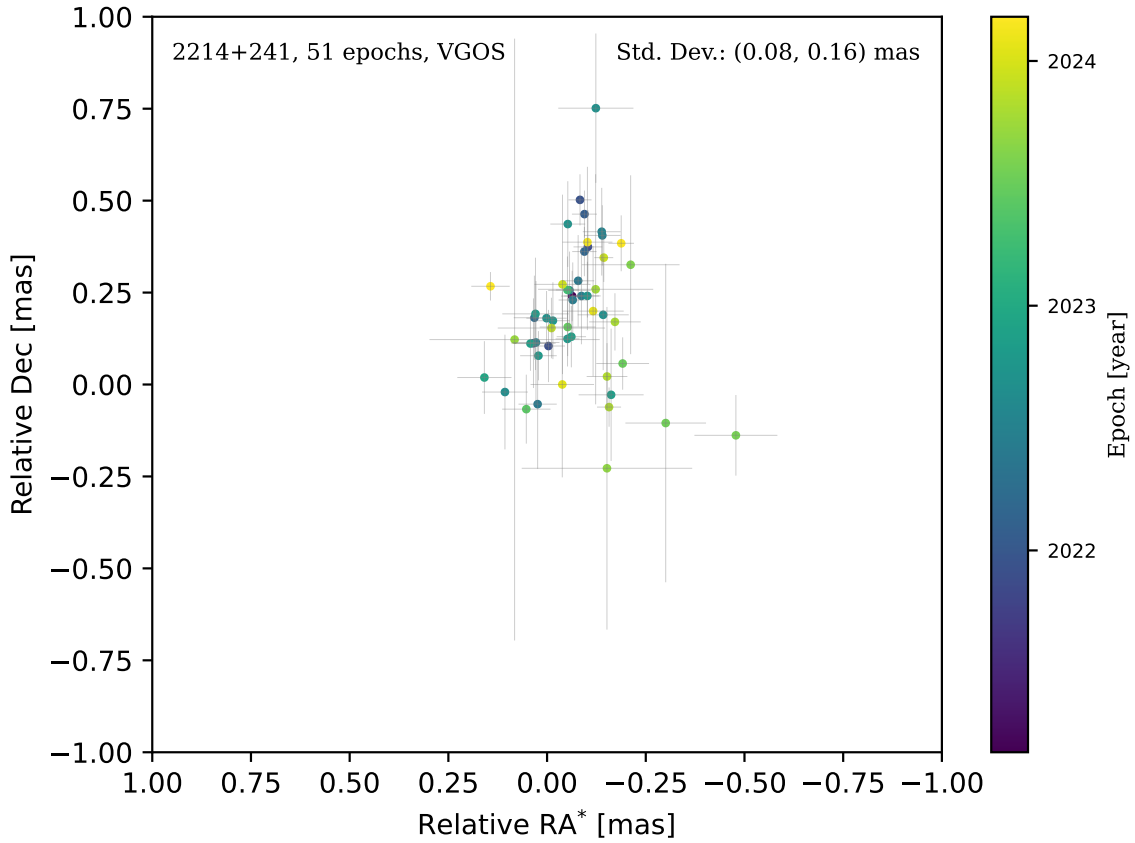

**Figure 41.** Position time series

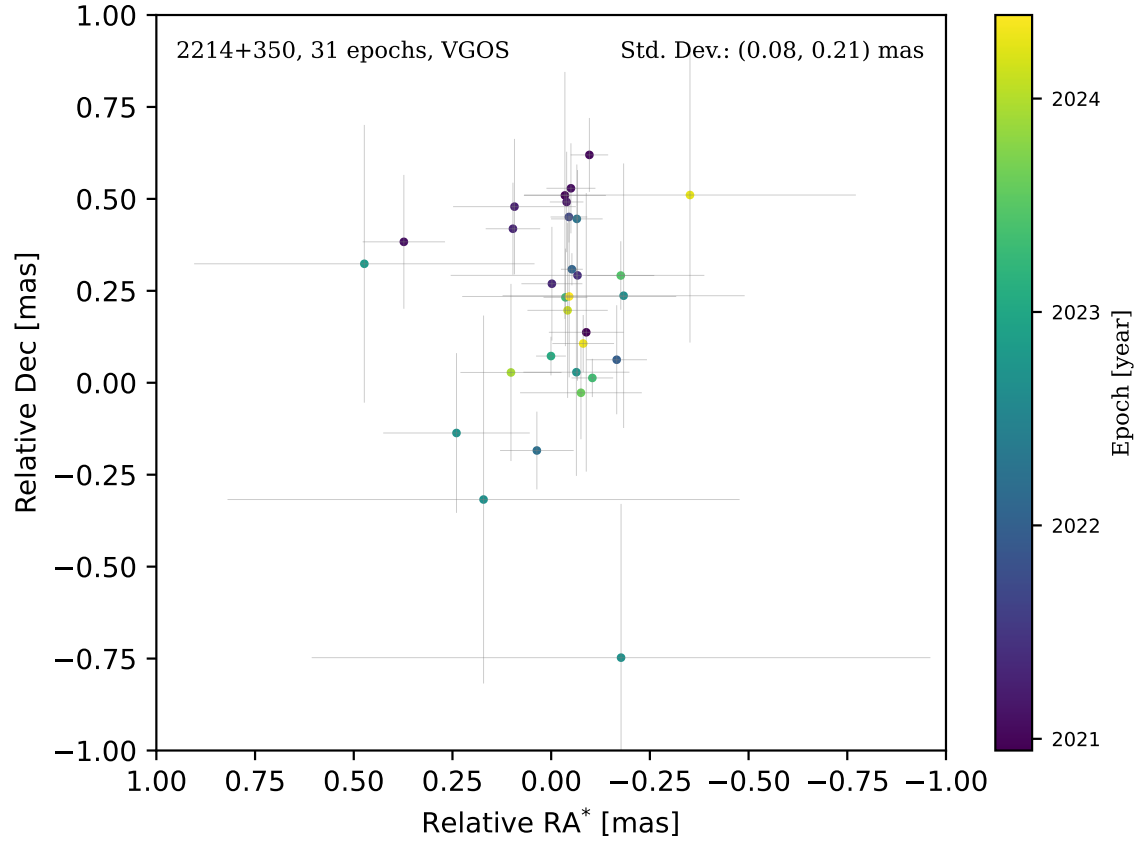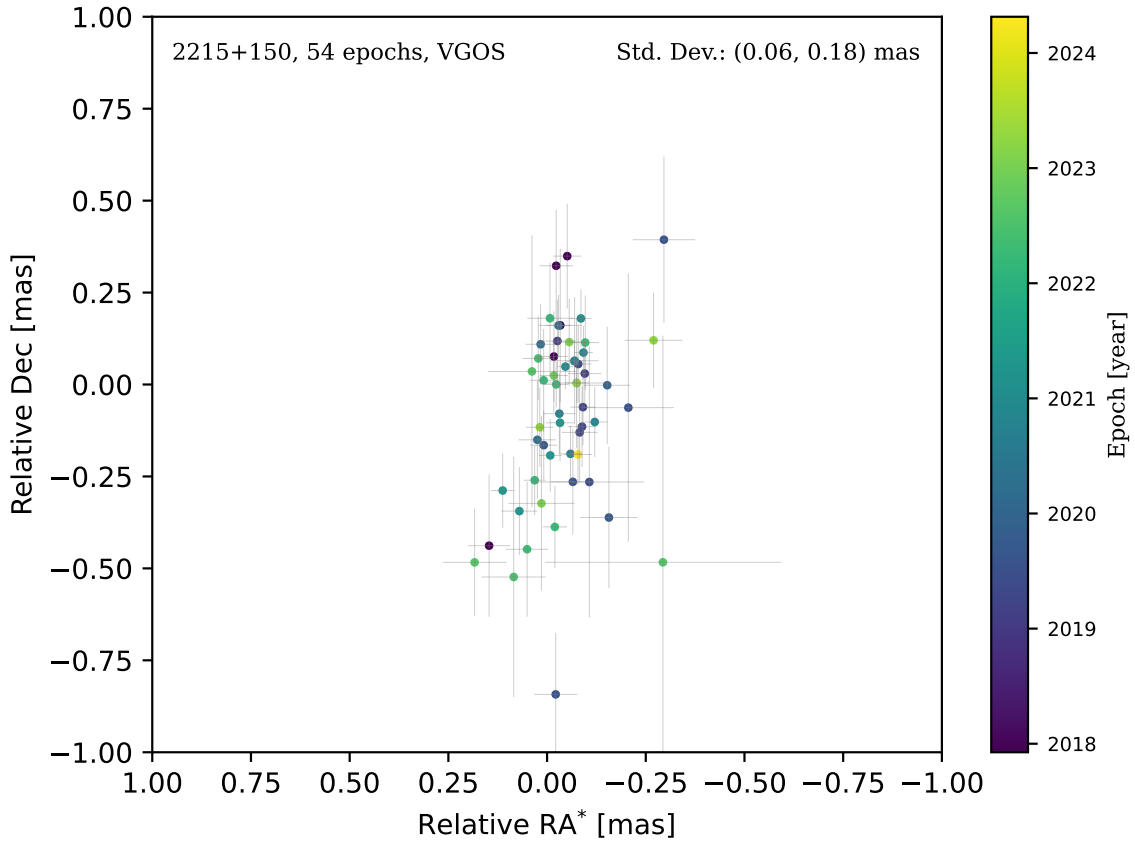

Figure 42. Position time series

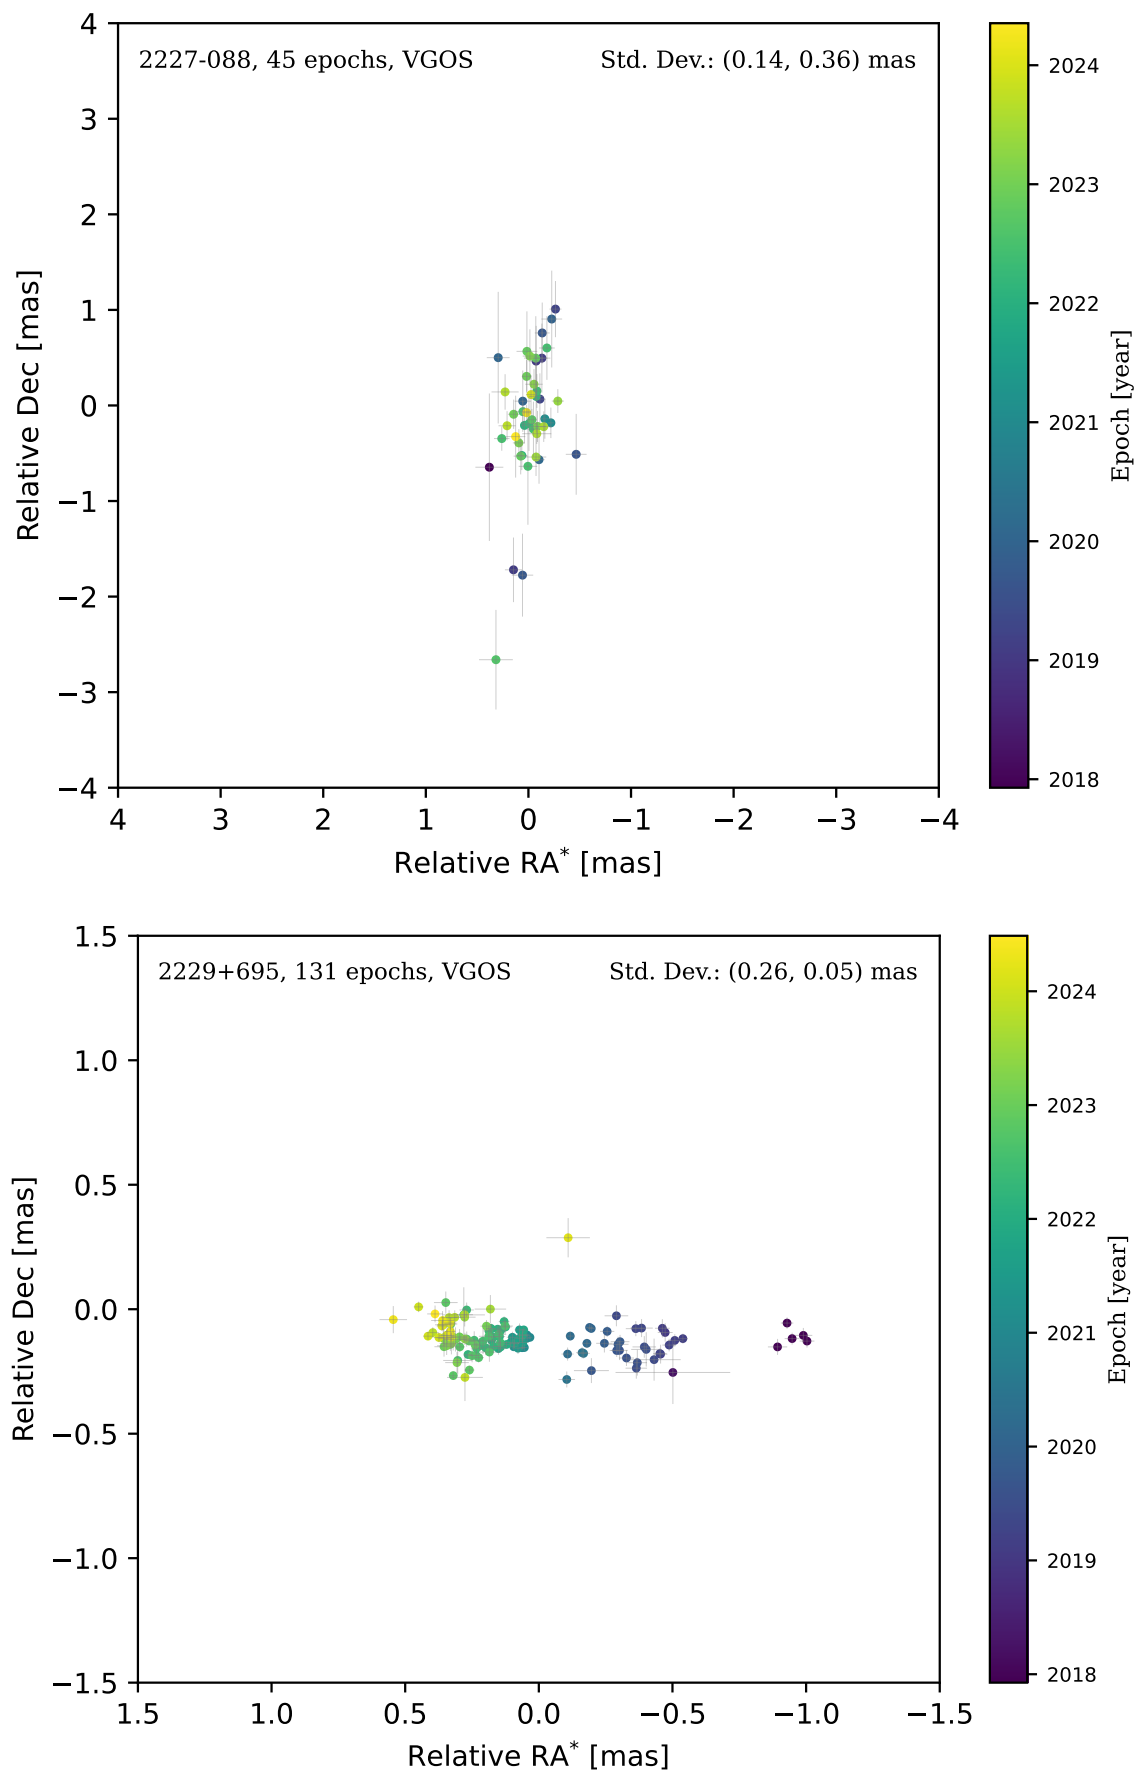

**Figure 43.** Position time series

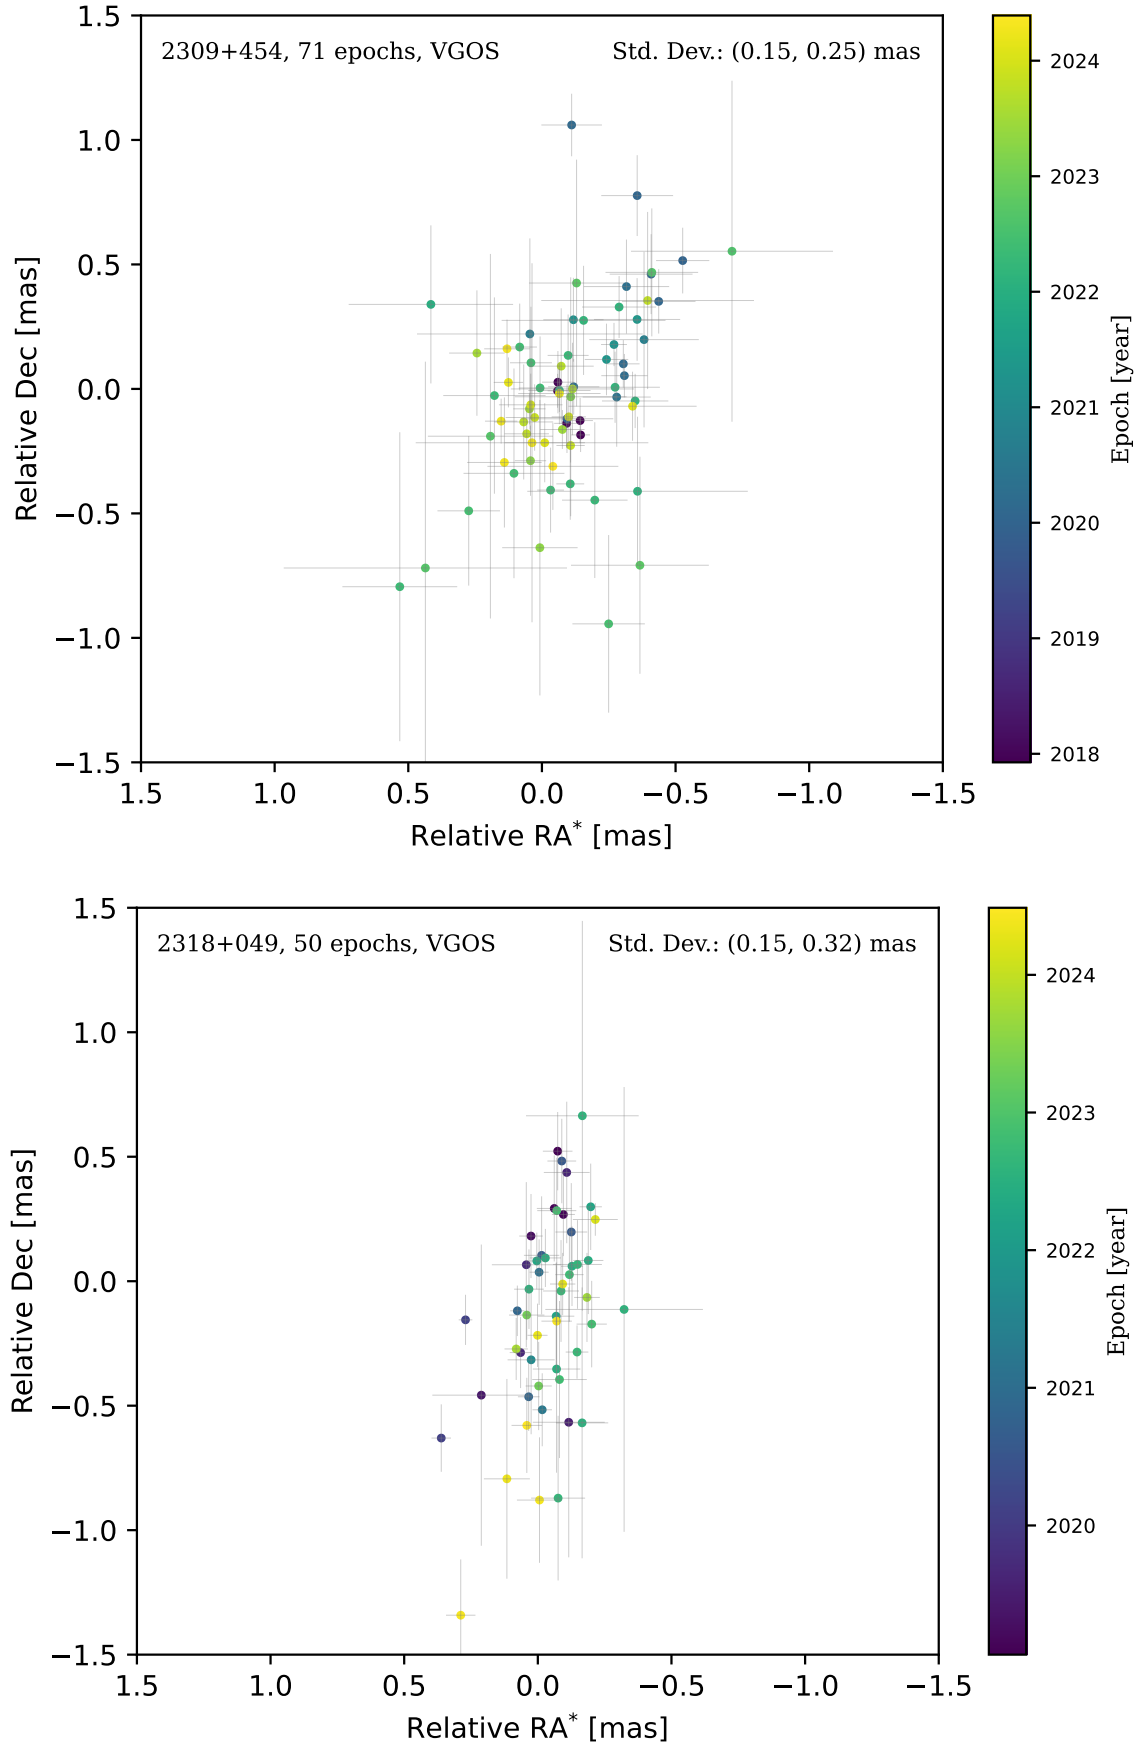

Figure 44. Position time series

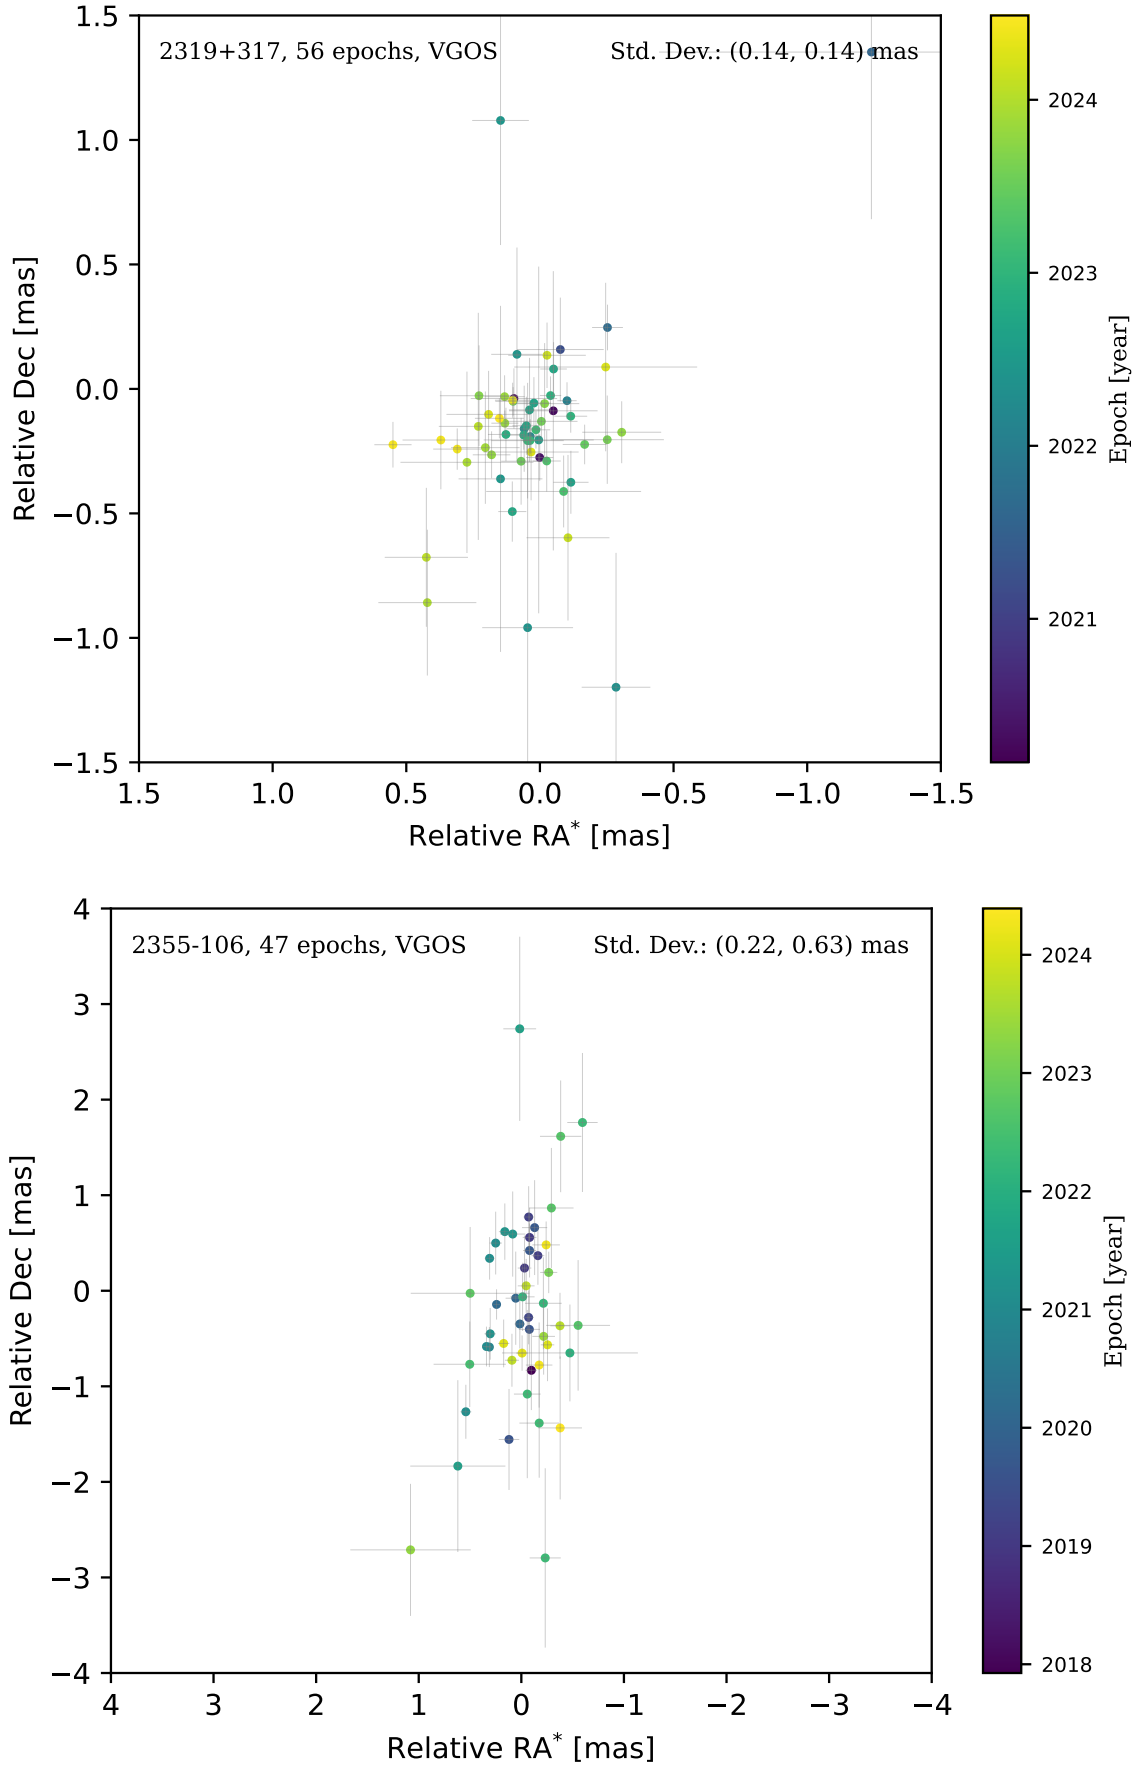

**Figure 45.** Position time series

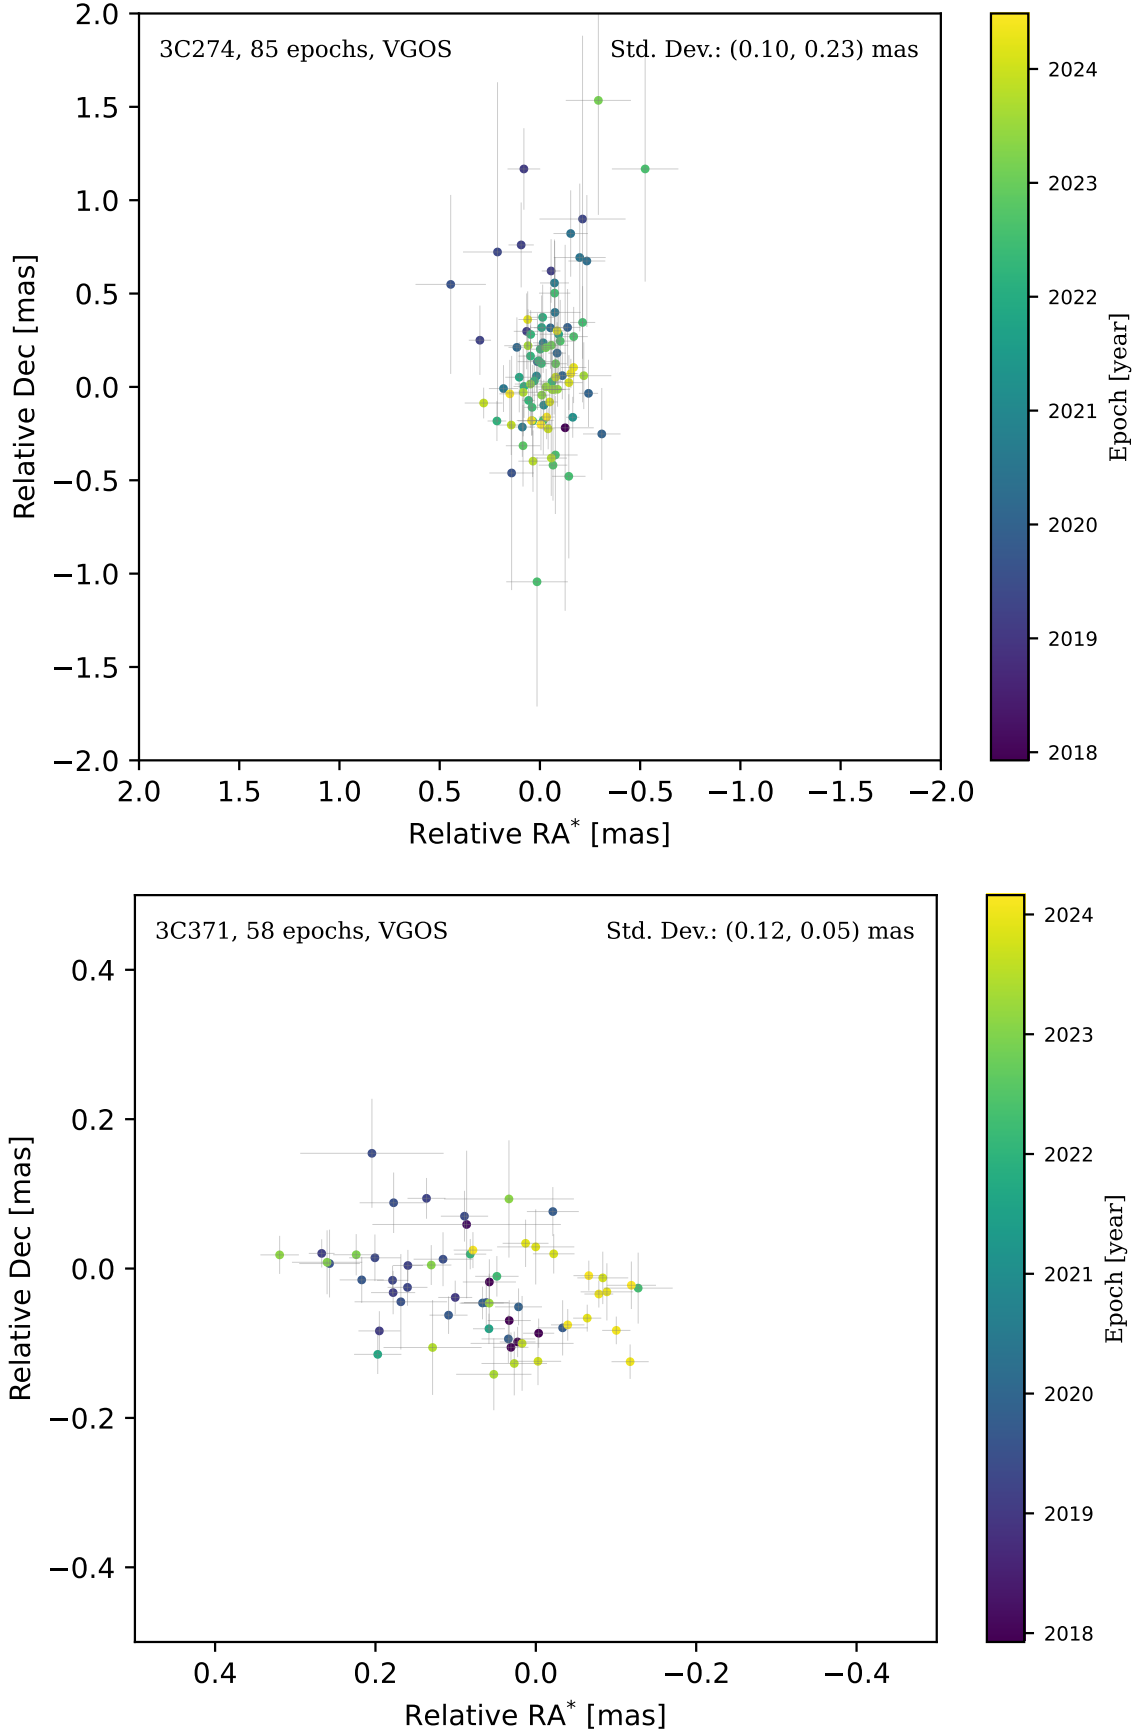

Figure 46. Position time series

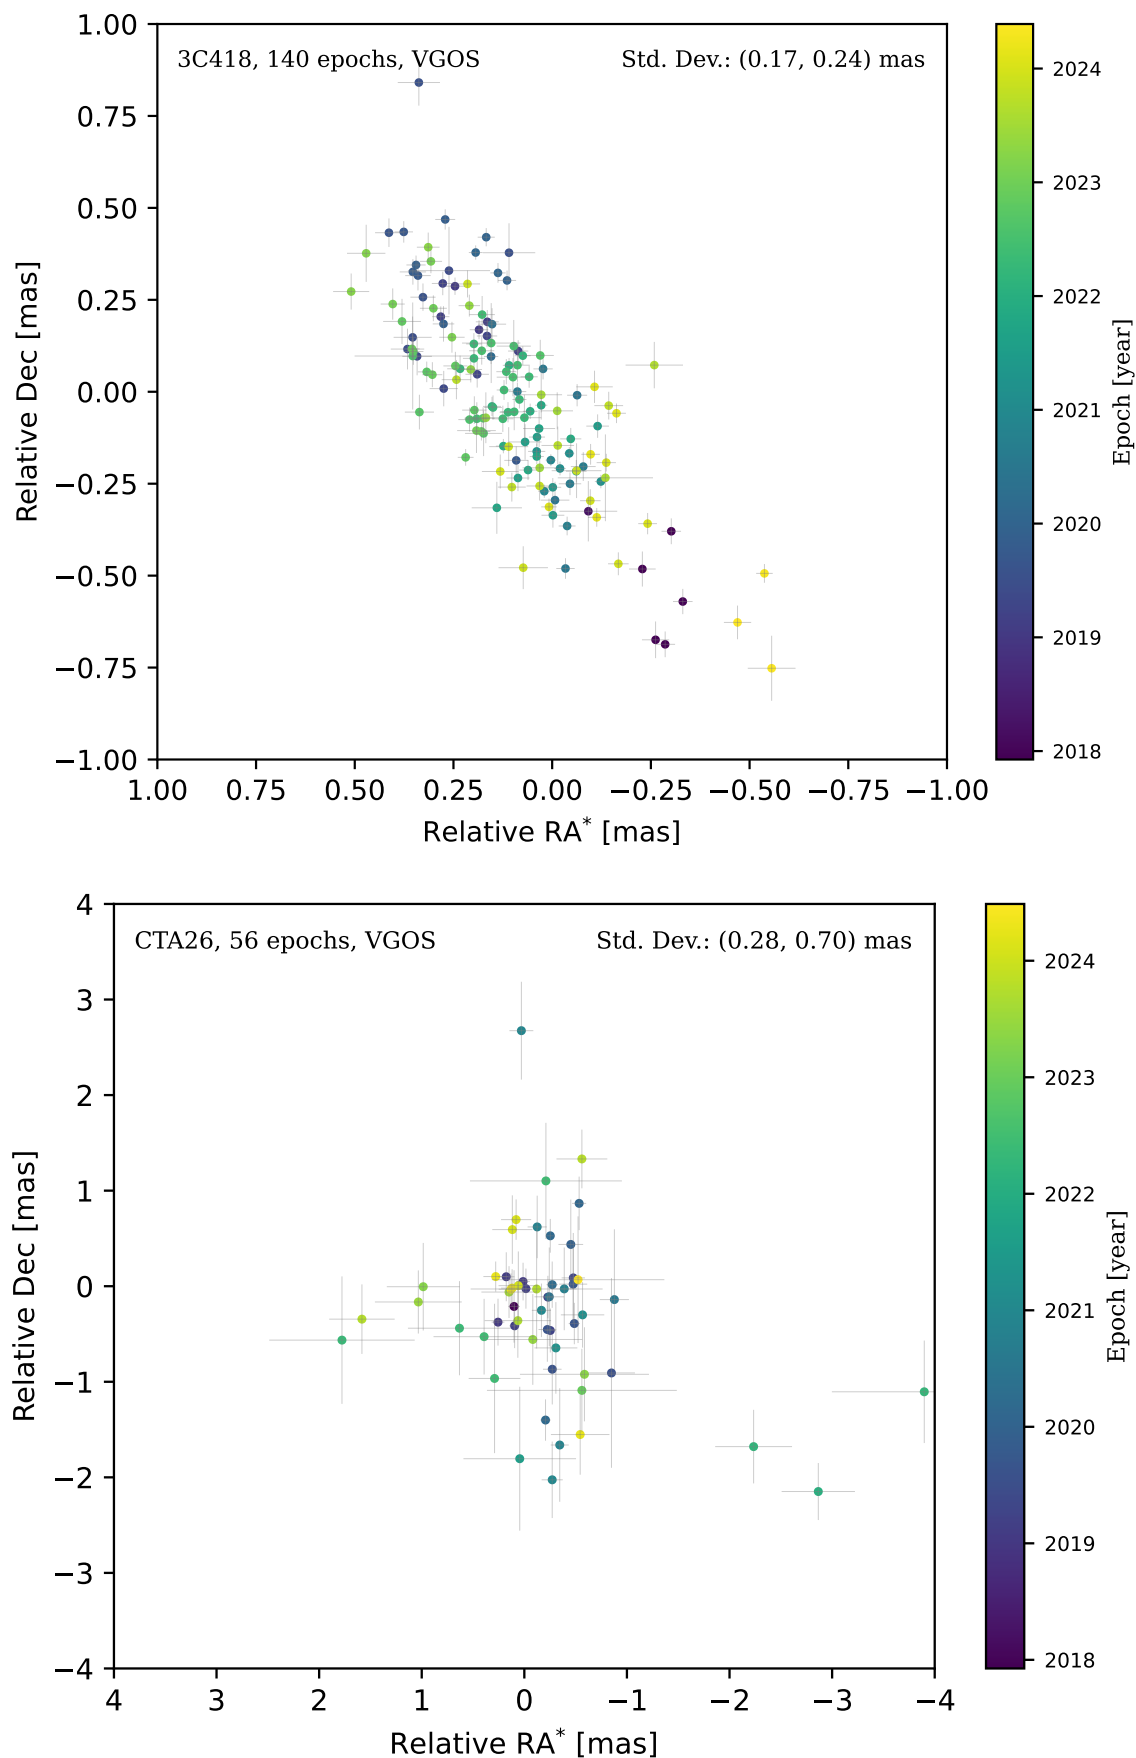

**Figure 47.** Position time series



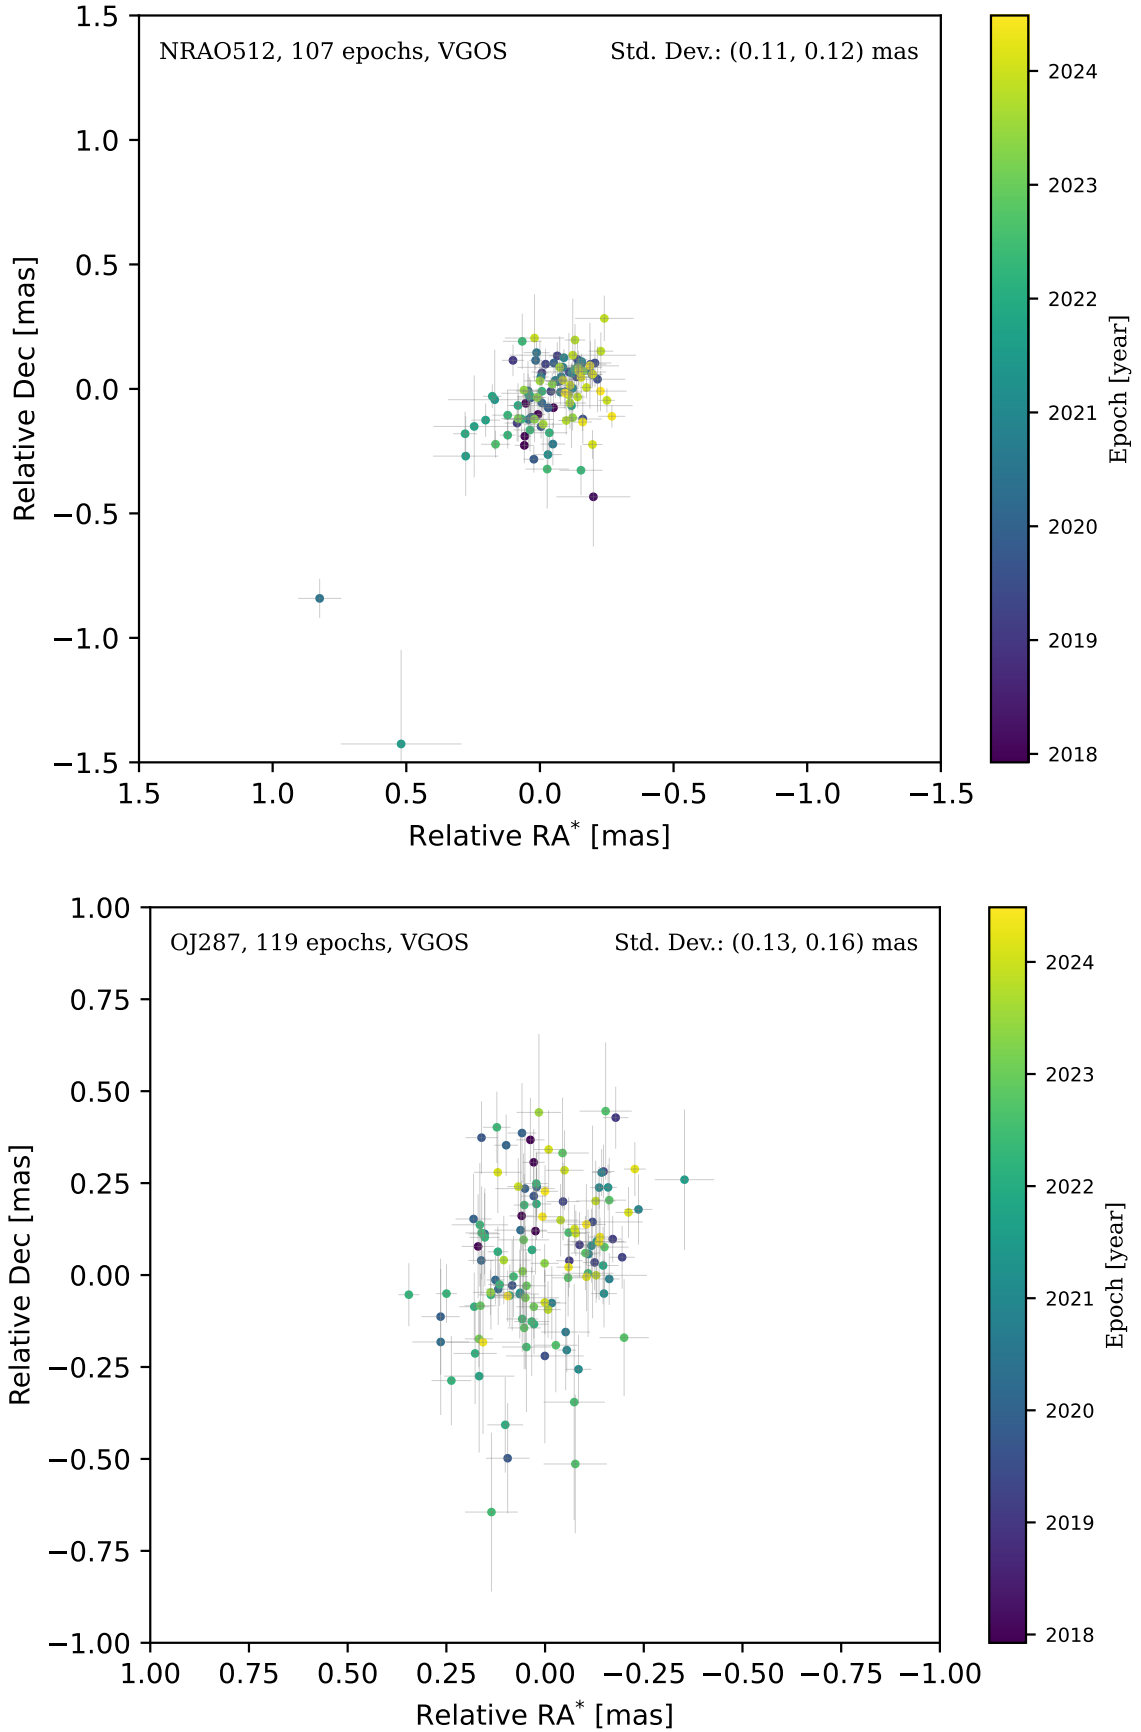**Figure 48.** Position time series
